# Supplementary material for: A guide to state-space modeling of ecological time series
Source: arXiv:2002.02001 ancillary file (2021-03-12)
Supplement: Supplementary file 1 [file Appendix_S2.pdf]

**Supporting Information.** Auger-Méthé, M., K. Newman, D. Cole, F. Empacher, R. Gryba, A.A. King, V. Leos-Barajas, J. Mills Flemming, A. Nielsen, G. Petris, L. Thomas. 2021. A guide to state-space modeling of ecological time series.

# Appendix S2: Methods to fit state-space models to data

## S2 1 Fitting SSMs

In the main text we introduce the main methods used to fit state-space models (SSMs) to data. In this Appendix, we present more technical details on these methods. We follow the same general structure as the main text, where we present the frequentist and Bayesian approaches separately. We use the toy model described in the main text to explain the different methods. We repeat here the definition of the model to facilitate comprehension of the methods:

$$z_t = \beta z_{t-1} + \epsilon_t, \qquad \epsilon_t \sim \mathrm{N}\left(0, \sigma_p^2\right), \tag{1}$$

$$y_t = \alpha z_t + \eta_t, \qquad \eta_t \sim \mathrm{N}\left(0, \sigma_o^2\right), \tag{2}$$

where $z_t$ is the state at time time $t$, $y_t$ is the observation at time $t$, $\beta$ is the autocorrelation in the states, $\alpha$ allows the observation at time $t$ to be a biased estimate of the state at time $t$, and $\sigma_p^2$ and $\sigma_o^2$ are the variances of the process variation and observation error. For our toy example, we view $z_0$ as a fixed and unknown parameter. This SSM can also be characterized in terms of probability distributions for the states and the observations:

$$f(z_t|z_{t-1}, \boldsymbol{\theta}_p), \qquad t = 1, \ldots, T, \tag{3}$$

$$g(y_t|z_t, \boldsymbol{\theta}_o), \qquad t = 1, \ldots, T, \tag{4}$$

where $f$ and $g$ are two normal probability density functions. See main text for more detail.

## S2 1.1 Frequentist approach

As discussed in the main text, when we fit a model with a frequentist approach, we often search for the parameter values that maximize the likelihood, a procedure we call maximum likelihood estimation. For our toy model, the joint likelihood for $\boldsymbol{\theta}$ and $\mathbf{z}_{1:T}$ is defined as:

$$L_{\mathrm{J}}(\boldsymbol{\theta}, \mathbf{z}_{1:T}|\mathbf{y}_{1:T}) = \prod_{t=1}^{T} g(y_t|z_t, \boldsymbol{\theta}_o) f(z_t|z_{t-1}, \boldsymbol{\theta}_p), \quad (5)$$

where $T$ is the length of our time series and $\boldsymbol{\theta}$ is a vector of (unknown) model parameters that contains the parameters for the process equation, $\boldsymbol{\theta}_p$, and the observation equation, $\boldsymbol{\theta}_o$, and in this example the initial state, $z_0$.

Maximizing the joint likelihood with respect to both parameters and the states is challenging, and instead a variety of two-step methods are used. In general, one step involves estimating the parameters by maximizing the marginal likelihood:

$$L_{\mathrm{M}}(\boldsymbol{\theta}|\mathbf{y}_{1:T}) = \int L_{\mathrm{J}}(\boldsymbol{\theta}, \mathbf{z}_{1:T}|\mathbf{y}_{1:T}) \mathrm{d}\mathbf{z}_{1:T}. \quad (6)$$

The other step involves estimating the states, often through the use of the conditional distributions of the states given the observations and the estimated parameter values. See main text for detail.

The different frequentist methods discussed in the main text are different ways to handle the high-dimensional integral of Eq. 6. We discuss in more detail three of these here. Before doing so, we will introduce briefly the concept of filtering, which is used in many of the fitting methods for SSMs.

### S2 1.1.1 Filtering

Filtering methods, such as the Kalman filter and sequential Mote Carlo methods, factorize the likelihood into a sequence of calculations (de Valpine, 2012). The sequential factorization of the marginal likelihood (Eq. 6) is:

$$L_{\mathrm{M}}(\boldsymbol{\theta}|\mathbf{y}_{1:T}) = p(\mathbf{y}_{1:T}|\boldsymbol{\theta}) = p(y_1|\boldsymbol{\theta}) \times p(y_2|y_1, \boldsymbol{\theta}) \times p(y_3|\mathbf{y}_{1:2}, \boldsymbol{\theta}) \times \ldots \times p(y_T|\mathbf{y}_{1:T-1}, \boldsymbol{\theta}). \quad (7)$$

In essence, this equation states that the probability of the data time series is the probability of the first observation multiplied by the probability of the second observation given the first multiple by the probability of the third observation given the previous two observations, and so on (de Valpine, 2012). This factorization allows one to calculate the likelihood recursively, where, each factor is a simpler integral:

$$p(y_t|\mathbf{y}_{1:t-1}, \boldsymbol{\theta}) = \int p(y_t|z_t, \boldsymbol{\theta}) p(z_t|\mathbf{y}_{1:t-1}, \boldsymbol{\theta}) \mathrm{d}\mathbf{z}_t. \quad (8)$$

Unlike the overall marginal likelihood (Eq. 6) where we integrate over the states from the entire time series, here we integrate out the possible state values for a single time step. For each time step, the various filtering methods calculate (or approximate) sequentially the probability of the state value $z_t$ given the previous observations $\mathbf{y}_{1:t-1}$ (referred as the one-step-ahead predictive distribution of the state) and the probability of the observation $y_t$ given the state $z_t$ and integrate over these (i.e., sum). Eq. 8 is sometimes referred as the one-step ahead predictive distribution of the observation. See de Valpine (2012) and Michaud et al. (2020) for more detail.

### S2 1.1.2 Kalman filter

Using the toy model described in the main text, we can describe the Kalman filter as follows. To initialize the Kalman filter recursions, one needs to either specify the initial state distribution as $z_0 \sim \text{N}(m_0, C_0)$ or consider $z_0$ to be an additional fixed unknown parameter (equivalent to setting $m_0 = z_0$ and $C_0 = 0$). For all other time steps, $t = 1, \ldots, T$, the Kalman filter sequentially calculates the following distributions. First, the prior distribution of $z_t$ given observations up to time $t-1$, also known as the one-step-ahead predictive distribution of the state, is calculated as:

$$z_{t|1:t-1} \sim \text{N}(a_t, R_t), \tag{9}$$

where $a_t = \beta m_{t-1}$, $R_t = \beta^2 C_{t-1} + \sigma_p^2$, and $\beta$ is the autocorrelation parameter and $\sigma_p^2$ is the variance in the process equation (Eq. 1) and $m_{t-1}$ and $C_{t-1}$ are defined below. Second, the predictive distribution of $y_t$ given observations up to time $t-1$, also known as the one-step-ahead predictive distribution of the observation, is calculated as:

$$y_{t|1:t-1} \sim \text{N}(f_t, Q_t), \tag{10}$$

where $f_t = \alpha a_t$, $Q_t = \alpha^2 R_t + \sigma_o^2$, and $\alpha$ is the bias parameter and $\sigma_o^2$ is the variance in the observation equation (Eq. 2). Finally, the posterior distribution of $z_t$ given observations up to time $t$, also known as the filtered distribution of the state, can be calculated as:

$$z_{t|1:t} \sim \text{N}(m_t, C_t), \tag{11}$$

where $m_t = a_t + \alpha R_t(y_t - f_t)/Q_t$ and $C_t = R_t - \alpha^2 R_t^2/Q_t$. In the main text, we refer $\text{N}(m_t, C_t)$ as the filtering distribution or density. The mean of each filtered distribution, $m_t$, provides a good point estimate of the state value at that time and the variance, $C_t$, quantifies the uncertainty around this estimate. We can view $m_t$ (the mean of the filtered distribution, i.e., $E[z_t|y_{1:t}]$), as a correction of $a_t$ (the mean of the one-step-ahead predictive distribution of the state, i.e., $E[z_t|y_{1:t-1}]$). The correction is based on the one-step-ahead prediction residual $(y_t - f_t)$, namely the difference between the observed value, $y_t$, and the mean of the one-step-ahead predictive distribution of the observation, $f_t$ (i.e., $E[y_t|y_{1:t-1}]$). The mean and variance of each smoothing distribution (i.e., distribution of $z_{t|1:T}$) can be obtained with a backward recursion in time, using an algorithm analogous to the Kalman filter called the Kalman smoother (Durbin and Koopman, 2012; Harvey, 1990).

The Kalman filter output can also be used to evaluate the marginal likelihood and thus to find the maximum likelihood estimates (MLEs). We can define the marginal likelihood as:

$$L_M(\boldsymbol{\theta}|\mathbf{y}_{1:T}) = \prod_{t=1}^{T} p(y_t|\mathbf{y}_{1:t-1}). \tag{12}$$

Because the one-step-ahead predictive distribution of the observation, $p(y_t|\mathbf{y}_{1:t-1})$ is defined as $\mathrm{N}(f_t, Q_t)$ in the Kalman filter (Eq. 10), we can easily calculate the marginal likelihood as:

$$L_M(\boldsymbol{\theta}|\mathbf{y}_{1:T}) = \prod_{t=1}^{T} (2\pi Q_t)^{-1/2} \exp\left\{-\frac{1}{2Q_t}(y_t - f_t)^2\right\}. \tag{13}$$

#### S2 1.1.3 Laplace approximation methods

The Laplace approximation of the marginal likelihood is derived by first approximating the natural logarithm of the joint likelihood ($\log L_{\mathrm{J}}$, Eq. 5), denoted $\ell_{\mathrm{J}}(\boldsymbol{\theta}, \mathbf{z}_{1:T}|\mathbf{y}_{1:T})$. The approximation uses a second order Taylor polynomial with respect to the states evaluated at $\hat{\mathbf{z}}_{1:T}$ (the value of $\mathbf{z}_{1:T}$ that maximizes $\ell_{\mathrm{J}}$):

$$\begin{aligned}\ell_{\mathrm{J}}(\boldsymbol{\theta}, \mathbf{z}_{1:T}|\mathbf{y}_{1:T}) \approx\ & \ell_{\mathrm{J}}(\boldsymbol{\theta}, \hat{\mathbf{z}}_{1:T}|\mathbf{y}_{1:T}) + \ell'_{\mathrm{J}}(\boldsymbol{\theta}, \hat{\mathbf{z}}_{1:T}|\mathbf{y}_{1:T})(\mathbf{z}_{1:T} - \hat{\mathbf{z}}_{1:T}) \\ & + \frac{1}{2}(\mathbf{z}_{1:T} - \hat{\mathbf{z}}_{1:T})^{\mathrm{tr}} \ell''_{\mathrm{J}}(\boldsymbol{\theta}, \hat{\mathbf{z}}_{1:T}|\mathbf{y}_{1:T})(\mathbf{z}_{1:T} - \hat{\mathbf{z}}_{1:T}),\end{aligned} \tag{14}$$

where $\ell'_{\mathrm{J}}(\boldsymbol{\theta}, \hat{\mathbf{z}}_{1:T}|\mathbf{y}_{1:T})$ and $\ell''_{\mathrm{J}}(\boldsymbol{\theta}, \hat{\mathbf{z}}_{1:T}|\mathbf{y}_{1:T})$ are the first and second derivatives of the joint log likelihood evaluated at points $\hat{\mathbf{z}}_{1:T}$, and $(\mathbf{z}_{1:T} - \hat{\mathbf{z}}_{1:T})^{\mathrm{tr}}$ is the transpose of $(\mathbf{z}_{1:T} - \hat{\mathbf{z}}_{1:T})$. Because $\hat{\mathbf{z}}_{1:T}$ maximizes $\ell_{\mathrm{J}}$, the first derivative evaluated at $\hat{\mathbf{z}}_{1:T}$ equals zero and the approximation simplifies to:

$$\ell_{\mathrm{J}}(\boldsymbol{\theta}, \mathbf{z}_{1:T}|\mathbf{y}_{1:T}) \approx \ell_{\mathrm{J}}(\boldsymbol{\theta}, \hat{\mathbf{z}}_{1:T}|\mathbf{y}_{1:T}) + \frac{1}{2}(\mathbf{z}_{1:T} - \hat{\mathbf{z}}_{1:T})^{\mathrm{tr}} \ell''_{\mathrm{J}}(\boldsymbol{\theta}, \hat{\mathbf{z}}_{1:T}|\mathbf{y}_{1:T})(\mathbf{z}_{1:T} - \hat{\mathbf{z}}_{1:T}). \tag{15}$$

The marginal likelihood can be approximated by exponentiating the approximation of the log joint likelihood and then integrating over the states. Noting that the joint likelihood evaluated at $\hat{\mathbf{z}}_{1:T}$, $L_{\mathrm{J}}(\boldsymbol{\theta}, \hat{\mathbf{z}}_{1:T}|\mathbf{y}_{1:T})$, is a constant term with respect to $\mathbf{z}_{1:T}$, we have the following:

$$L_{\mathrm{M}} \approx L_{\mathrm{J}}(\boldsymbol{\theta}, \hat{\mathbf{z}}_{1:T}|\mathbf{y}_{1:T}) \int \exp\left(\frac{1}{2}(\mathbf{z}_{1:T} - \hat{\mathbf{z}}_{1:T})^{\mathrm{tr}} \ell''_{\mathrm{J}}(\boldsymbol{\theta}, \hat{\mathbf{z}}_{1:T}|\mathbf{y}_{1:T})(\mathbf{z}_{1:T} - \hat{\mathbf{z}}_{1:T})\right) \mathrm{d}\mathbf{z}_{1:T} \tag{16}$$

The integrand is as a quantity proportional to the density function of a multivariate Gaussian known as the kernel. Thus, the integral will be the normalizing constant (i.e., the constant with which we divide the unnormalized function) of this multivariate Gaussian distribution:

$$L_{\mathrm{M}} \approx L_{\mathrm{J}}(\boldsymbol{\theta}, \hat{\mathbf{z}}_{1:T}|\mathbf{y}_{1:T}) \sqrt{\frac{(2\pi)^T}{\det(-\ell''_{\mathrm{J}}(\boldsymbol{\theta}, \hat{\mathbf{z}}_{1:T}|\mathbf{y}_{1:T}))}}. \tag{17}$$

As it is clear from Eq. 14, the Laplace approximation requires to maximize the joint log likelihood with respect to the state $\hat{\mathbf{z}}_{1:T}$. As such, maximizing the marginal likelihood with the Laplace approximation requires a recursive inner and outer maximization procedure. The parameters are explored via the outer maximization, while for each given set of parameter values explored the states are estimated via the inner maximization. Thus, even though the states and parameters are estimated differently (see main text), the state estimates are returned at the same time as the parameter estimates.

### S2 1.1.4 Sequential Monte Carlo methods

Monte Carlo methods are sampling procedures that generate random samples from specific probability distributions, which can then be used to evaluate integrals. For example, if $X$ is a continuous random variable with a probability density function $f(x)$, the expected value of $X$ is $E[X] = \int x f(x)dx$. A Monte Carlo solution is to generate a random sample $x_{1:N}$ from $f(x)$ and the estimate $E[X]$ with $\frac{1}{N}\sum_{i=1}^{N} x_i$.

Sequential importance sampling (SIS; Doucet et al., 2001) can be used to numerically approximate one of the important integrations associated with fitting SSMs to data. To estimate the smoothed state at time $t$, $\hat{z}_{t|1:T}$, one needs to perform the following high-dimensional integration:

$$E[z_t|y_{1:T}, \boldsymbol{\theta}] = \int z_t p(\mathbf{z}_{1:T}|\mathbf{y}_{1:T}, \boldsymbol{\theta})\mathrm{d}\mathbf{z}_{1:T}. \tag{18}$$

SIS is a procedure that uses an importance function to sequentially generate $N$ samples of the state for each time step $t$, $z_t^i$, $i$=1,..., $N$. In the context of SSMs, the importance function is often the probability density function of the state at time $t$: $f(z_t|z_{t-1}, \boldsymbol{\theta}_p)$. Each sequence or sample trajectory $z_{1:t}^i$ is referred to as a particle. SIS also keeps track of the importance weights, $w_t^i$, of each sample $i$ at time $t$ in order to approximate an overall importance value for each sample trajectory, $w_T^{*,i}$. In the context of SSMs, the importance weights at time $t$ are functions of the probability density function of the observations, $g(y_t|z_t^i, \boldsymbol{\theta}_o)$, and are updated sequentially as follows:

$$w_t^i \propto w_{t-1}^i g(y_t|z_t^i, \boldsymbol{\theta}_o). \tag{19}$$

For example, for our toy model (Eqs. 1-2), the $i^{th}$ sample of the state at time $t$, $z_t^i$, would be sampled from $\mathrm{N}(\beta z_{t-1}^i, \sigma_p^2)$ and the weights are calculated as:

$$w_t^i \propto w_{t-1}^i \frac{1}{\sqrt{2\pi\sigma_o^2}} \exp\left(-\frac{1}{2\sigma_o^2}(y_t - \alpha z_t^i)^2\right). \tag{20}$$

A smoothed estimate of the state at time $t$ is the weighted average of the $N$ simulated states for that time point:

$$\hat{z}_{t|1:T} = \sum_{i=1}^{N} w_T^{*,i} z_t^i, \tag{21}$$

where $w_T^{*,i} = \frac{w_T^i}{\sum_{j=1}^N w_T^j}$. The final normalized importance weight, $w_T^{*,i}$, represents how likely the $i^{th}$ particle is compared to the other particles.

SIS is impractical for even moderately long time series (e.g., $T$=20). The problem is that the weights of particles become increasingly uneven, with only a small proportion of the particles typically having the majority of the weight. This leads to state estimates with unacceptably large variances. The gradual erosion of support for many of the particles, known as particle depletion, is a serious problem with sequential importance sampling and other particle filters.

The bootstrap filter (Gordon et al., 1993) is a procedure designed to remedy particle depletion. The bootstrap filter assesses the weight of a particle through time and iteratively removes particles with low weights and replaces them with duplicates of particles with higher weights. There are various algorithms for the bootstrap filter. The one described below, and implemented in Appendix S1, is the simplest and involves resampling the particles after each iteration. At iteration $t$:

1. Generate a state value at time $t$ for each particle $i$, $\tilde{z}_t^i$, with the probability density function of the state (i.e., with the process equation), $f(z_t|z_{t-1}^i, \boldsymbol{\theta}_p)$.
2. Set $\tilde{z}_{1:t}^i = (z_{1:t-1}^i, \tilde{z}_t^i)$.
3. Calculate the normalized importance weights of each proposed state $\tilde{z}_t^i$, $w_t^{*,i}$, using the observation equation, $g(y_t|z_t, \boldsymbol{\theta}_o)$.
4. Randomly sample $N$ times (with replacement) from the $N$ particle vectors with probabilities, $w_t^{*,i}$, and denote the selected vectors $z_{1:t}^i$, $i$=1,. . .,$N$. Set the unnormalized weights $w_t^i$ equal to 1.

Because the simulated particles are resampled after each iteration, the simple average of the simulated states based on the selected particles at time $t$ is the filtered state estimate, $\hat{z}_{t|1:t}$, while the simple average based on the final set of particles at time $T$ is the smoothed state estimate, $\hat{z}_{t|1:T}$. While the bootstrap filter can reduce particle depletion, it does not completely solve the problem particularly for long time series.

While one can use SIS or the bootstrap filter (or any of the broader class of related algorithms known as 'particle filters') to estimate the likelihood, in order to perform frequentist inference, one must be able to maximize the likelihood. This presents a number of difficulties. First, the likelihood estimates given by the particle filter algorithms are noisy due to their Monte Carlo nature. As the variance in these estimates grows, the utility of the estimates is diminished. Second, these algorithms can be computationally expensive, because each likelihood calculation requires simulation of $N$ realizations of the latent state process, where $N$ must be large enough to yield precise likelihood estimates. Finally, to maximize the likelihood, one must explore what is in many cases a complicated likelihood surface, marked by features such as multiple local maxima, narrow, curved ridges, and precipitous

cliffs. Exploring this surface in search of its highest peaks will necessarily involve numerous likelihood evaluations. Thus, while it is in principle possible to use a general-purpose optimization algorithm such as Nelder-Mead to maximize the likelihood computed by a particle filter, in practice this is typically prohibitively expensive. Iterated filtering is an attractive alternative.

As its name implies, iterated filtering (IF) involves repeatedly applying a particle filter as a means of maximizing the likelihood. Repeated application of a particle filter at a single parameter value merely results in multiple estimates of the likelihood. To explore the likelihood surface, IF effectively modifies the model by turning parameters into state variables. In particular, the fixed parameters of the model of interest are perturbed, at each observation time, by a random amount. This random perturbations forestall particle depletion by continually re-injecting random variability into the filter. This reduces the Monte Carlo noise of the likelihood estimates. Thus, paradoxically, it is frequently possible when using IF to maximize the likelihood using a much smaller $N$ than is needed to precisely estimate the likelihood itself. Finally, the random perturbations of the parameters act to harvest information from a local neighborhood; IF exploits this information to increase the likelihood at each iteration, on average. However, despite all of these performance enhancements, because it applies artificial perturbations to parameters, IF is learning not about the model of interest (i.e., model with fixed parameters), but only about a modified model (i.e., model where fixed parameters have been transformed into state variables). Therefore, as filtering iterations proceed, one gradually cools (i.e., reduces the magnitude of) the artificial perturbations, so that the modified model approaches the model of interest as the iterations proceed. In theory, if the cooling is sufficiently slow, and the number of iterations sufficiently large, the algorithm will converge to some local likelihood maximum. In practice, as with related algorithms such as simulated annealing or Markov Chain Monte Carlo, the number of iterations required by the theory can be prohibitively large. Moreover, because statistical inference hinges on identification of the global likelihood maximum and exploration of its neighborhood, a single IF computation is never sufficient. For these reasons, it is usually advisable to perform many independent, relatively short, IF computations, starting from widely dispersed starting points. In such a global search strategy, one relies on the ability of each independent IF computation to rapidly ascend the surface in the vicinity of its starting point. Because this strategy is easily parallelizable, one can efficiently exploit modern high-performance computing technology to search for the global maximum. IF can be easily implemented using the `R` package `pomp` (see Appendix S1, King et al., 2009).

## S2 1.2 Bayesian framework

As mentioned in the main text, the function of interest when we fit a SSM with a Bayesian approach is the posterior distribution for the states and parameters given the observations. For the toy model, the posterior distribution for states and parameters given the observations

is defined as:

$$p(\boldsymbol{\theta}, \mathbf{z}_{1:T}|\mathbf{y}_{1:T}, \boldsymbol{\lambda}) = \frac{L_{\text{J}}(\boldsymbol{\theta}, \mathbf{z}_{1:T}|\mathbf{y}_{1:T})\pi(\boldsymbol{\theta}|\boldsymbol{\lambda})}{\int\int L_{\text{J}}(\boldsymbol{\theta}, \mathbf{z}_{1:T}|\mathbf{y}_{1:T})\pi(\boldsymbol{\theta}|\boldsymbol{\lambda})\mathrm{d}\mathbf{z}_{1:T}\mathrm{d}\boldsymbol{\theta}}, \tag{22}$$

where $L_{\text{J}}(\boldsymbol{\theta}, \mathbf{z}_{1:T}|\mathbf{y}_{1:T})$ is the joint likelihood (i.e., $p(\mathbf{y}_{1:T}|\boldsymbol{\theta}, \mathbf{z}_{1:T})$, see for example Eq. 5), and $\pi(\boldsymbol{\theta}|\boldsymbol{\lambda})$ is the prior distribution(s) for the parameters with fixed hyperparameters, $\boldsymbol{\lambda}$.

Instead of calculating the posterior distribution explicitly, researchers generally approximate it by taking large samples of states and parameters from the posterior distribution. Simulating independent draws from the posterior distribution is typically impossible and researchers often use Markov Chain Monte Carlo (MCMC) methods to obtain samples from the posterior distribution. Here, we discuss in more details one of the main MCMC methods.

#### S2 1.2.1 Metropolis-Hastings samplers

Metropolis-Hastings samplers are at the base of most MCMC algorithms used to sample the posterior distribution in a Bayesian analysis. Metropolis-Hastings samplers are iterative algorithms that create an appropriate Markov chain to sample the target distribution. For demonstrative purposes, let's say we have a very simple model with one parameter, $\theta$, no latent states, and where the observations $y_i \overset{\text{i.i.d.}}{\sim} f(y|\theta)$. We denote the likelihood function with $L(\theta|\mathbf{y}_{1:N})$ and the prior with $\pi(\theta)$. A Metropolis-Hastings algorithm samples the values of the parameter at step $j$ of the chain, $\theta^j$, with the following iterative rules. For time step $j$ of the chain, first generate a candidate value, $\tilde{\theta}^j$, with a proposal distribution, $q(\tilde{\theta}^j|\theta^{j-1})$. For example, the proposal distribution for the candidate value could be a Gaussian distribution centered on the previous value of the chain (i.e., $\tilde{\theta}^j \sim \mathrm{N}(\theta^{j-1}, \sigma^2_{\mathrm{MH}})$). Second, accept the candidate value with probability $\alpha(\theta^{j-1}, \tilde{\theta}^j) = \min(1, p_\theta)$, where

$$p_\theta = \frac{L(\tilde{\theta}^j|\mathbf{y}_{1:N})\pi(\tilde{\theta}^j)}{L(\theta^{j-1}|\mathbf{y}_{1:N})\pi(\theta^{j-1})}\frac{q(\theta^{j-1}|\tilde{\theta}^j)}{q(\tilde{\theta}^j|\theta^{j-1})}. \tag{23}$$

If the proposed value is accepted $\theta^j = \tilde{\theta}^j$; if not, the previous value of the chain is used: $\theta^j = \theta^{j-1}$. The first value of the chain, $\theta^0$, will affect the chain and the convergence towards the target distribution (see main text for a discussion of convergence diagnostics).

In the context of SSMs, we have a multivariate posterior distribution for the states and the parameters. Using Metropolis-Hastings algorithms to sample for more than one random variables is more complex, but there are various implementation tools to do so. For example, for each iteration $j$ of the chain, one can first sample sequentially all parameter values, and then sequentially sample the state values (Newman et al., 2014). Let us denote the parameters of our toy example as $\boldsymbol{\theta} = (\boldsymbol{\theta}_p, \boldsymbol{\theta}_o, z_0) = (\beta, \sigma_p, \alpha, \sigma_o, z_0)$ and the elements of $\boldsymbol{\theta}$ with $r = 1, ..., 5$. For iteration $j$ and $r > 1$, we will have already updated some of the parameters. For example, when updating $r = 2$ we will have $\boldsymbol{\theta}^{j-1}_{[2]} = (\beta^j, \sigma^{j-1}_p, \alpha^{j-1}, \sigma^{j-1}_o, z^{j-1}_0)$ as

our current parameters and $\tilde{\boldsymbol{\theta}}^j_{[2]} = (\beta^j, \tilde{\sigma}^j_p, \alpha^{j-1}, \sigma_o^{j-1}, z_0^{j-1})$ as our candidate value. For each parameter $r$, we would accept the candidate value with probability $\alpha_r = \min(1, p_{\theta_r})$, where

$$p_{\theta_r} = \frac{\prod_{t=1}^T g(y_t|z_t, \tilde{\boldsymbol{\theta}}^j_{[r]}) f(z_t|z_{t-1}, \tilde{\boldsymbol{\theta}}^j_{[r]}) \pi(\tilde{\boldsymbol{\theta}}^j_{[r]}|\boldsymbol{\lambda})}{\prod_{t=1}^T g(y_t|z_t, \boldsymbol{\theta}^{j-1}_{[r]}) f(z_t|z_{t-1}, \boldsymbol{\theta}^{j-1}_{[r]}) \pi(\boldsymbol{\theta}^{j-1}_{[r]}|\boldsymbol{\lambda})} \frac{q(\boldsymbol{\theta}^{j-1}_{[r]}|\tilde{\boldsymbol{\theta}}^j_{[r]})}{q(\tilde{\boldsymbol{\theta}}^j_{[r]}|\boldsymbol{\theta}^{j-1}_{[r]})}, \tag{24}$$

Once all $r$ parameters have been sampled, we would sequentially sample the states for iteration $j$. We would sequentially accept a candidate state value with probability $\alpha_t = \min(1, p_{z_t})$, where

$$p_{z_t} = \frac{g(y_t|\tilde{z}^j_t, \boldsymbol{\theta}^j) f(\tilde{z}^j_t|z^j_{t-1}, \boldsymbol{\theta}^j) f(z^{j-1}_{t+1}|\tilde{z}^j_t, \boldsymbol{\theta}^j)}{g(y_t|z^{j-1}_t, \boldsymbol{\theta}^j) f(z^{j-1}_t|z^j_{t-1}, \boldsymbol{\theta}^j) f(z^{j-1}_t|z^{j-1}_{t-1}, \boldsymbol{\theta}^j)} \frac{q(z^{j-1}_t|\tilde{z}^j_t)}{q(\tilde{z}^j_t|z^{j-1}_t)}. \tag{25}$$

Note that all other terms of the posterior cancel out, since they use the same previously sampled values (e.g., $\pi(\boldsymbol{\theta}^j)$ and $f(y_{t-1}|z^j_{t-1})$). Note that if groups of variables are related they can be sampled simultaneously from a multivariate distribution rather than sequentially. In practice, states and parameters are often correlated, and thus it may be difficult to implement an efficient MCMC sampler that does not require very long simulations before convergence (Newman et al., 2014).

Gibbs samplers are commonly-used Metropolis-Hastings samplers for multivariate distributions, where the proposal distributions are conditional distributions of the target distribution and thus the candidate values are always accepted (Geyer, 2011). Deriving these conditional distributions is facilitated by the fact that they are proportional to the target distribution and that functions that do not include the variable of interest will be cancelled out. For example, the full conditional distribution of the state $z_t$ for a general SSM is:

$$q(z_t|z_{t-1}, z_{t+1}, \boldsymbol{\theta}^j, y_t) \propto g(y_t|z_t, \boldsymbol{\theta}^j) f(z_t|z_{t-1}, \boldsymbol{\theta}^j) f(z_{t+1}|z_t, \boldsymbol{\theta}^j), \tag{26}$$

which is a much simpler expression than Eq. 22 and have some of the same components as Eq. 25. When the conditional distribution is available in closed form, it is easy to sample from it exactly. For the toy model, the full conditional distribution of $z_t$ is Normal, with mean

$$\mu_c = \left(\frac{\alpha^2}{\sigma_o^2} + \frac{1+\beta^2}{\sigma_p^2}\right)^{-1} \left(\frac{\alpha y_t}{\sigma_o^2} + \frac{\beta(z_{t-1} + z_{t+1})}{\sigma_p^2}\right), \tag{27}$$

and variance

$$\sigma_c^2 = \left(\frac{\alpha^2}{\sigma_o^2} + \frac{1+\beta^2}{\sigma_p^2}\right)^{-1}. \tag{28}$$

In this case, simulating from this normal distribution is straightforward and it allows us to forego the acceptance step of other Metropolis-Hastings algorithms. For NDLMs, the entire sequence $\mathbf{z}_{0:T}$ can be simulated at once from its conditional distribution, given the data $\mathbf{y}_{1:T}$ and the time-invariant parameter $\boldsymbol{\theta}$, using the Forward Filtering Backward Sampling

(FFBS) algorithm described in Carter and Kohn (1994). Note that the FFBS algorithm can also be used to conduct inference for the SSMs that are conditionally linear and Gaussian. However, Gibbs samplers for nonlinear and non Gaussian models often require sampling from each conditional distribution sequentially (see chapter 4.5 of Prado and West, 2010, for an overview). A drawback of this particular Gibbs sampler design is that consecutive draws of $z_{0:T}^{j}$ and $z_{0:T}^{j-1}$ tend to be highly correlated, slowing the convergence of sample averages to their theoretical expected values, thus deteriorating the quality of the Monte Carlo approximations.

# Literature Cited


Carter, C. K. and Kohn, R. (1994). On Gibbs sampling for state space models. *Biometrika*, 81:541–553.

de Valpine, P. (2012). Frequentist analysis of hierarchical models for population dynamics and demographic data. *Journal of Ornithology*, 152:S393–S408.

Doucet, A., De Freitas, N., and Gordon, N. (2001). An introduction to sequential Monte Carlo methods. In *Sequential Monte Carlo methods in practice*, pages 3–14. Springer.

Durbin, J. and Koopman, S. J. (2012). *Time series analysis by state space methods.* Oxford University Press, Oxford, UK, 2nd edition.

Geyer, C. (2011). Introduction to Markov Chain Monte Carlo. In Brooks, S., Gelman, A., Jones, G., and Meng, X.-L., editors, *Handbook of Markov Chain Monte Carlo*, chapter 1, pages 3–48. Chapman and Hall/CRC, New York, NY.

Gordon, N. J., Salmond, D. J., and Smith, A. F. M. (1993). Novel approach to nonlinear/non-gaussian bayesian state estimation. *IEE Proceedings F - Radar and Signal Processing*, 140:107–113.

Harvey, A. C. (1990). *Forecasting, structural time series models and the Kalman filter.* Cambridge university press, Cambridge, UK.

King, A. A., Ionides, E. L., Bretó, C. M., Ellner, S., Kendall, B., Wearing, H., Ferrari, M. J., Lavine, M., and Reuman, D. C. (2009). pomp: Statistical inference for partially observed markov processes. *URL http://pomp. r-forge. r-rproject. org.*

Michaud, N., de Valpine, P., Turek, D., Paciorek, C. J., and Nguyen, D. (2020). Sequential Monte Carlo methods in the nimble R package. *arXiv e-prints*, page arXiv:1703.06206.

Newman, K. B., Buckland, S. T., Morgan, B. J. T., King, R., Borchers, D. L., Cole, D. J., Besbeas, P., Gimenez, O., and Thomas, L. (2014). *Modelling population dynamics: model formulation, fitting and assessment using state-space methods.* Springer, New York, NY.

Prado, R. and West, M. (2010). *Time series: modeling, computation, and inference.* Chapman & Hall/CRC, Boca Raton, FL.
