# Supplementary material for: A guide to state-space modeling of ecological time series
Source: arXiv:2002.02001 ancillary file (2021-03-12)
Supplement: Supplementary file 2 [file Appendix_S3.pdf]

**Supporting Information.** Auger-Méthé, M., K. Newman, D. Cole, F. Empacher, R. Gryba, A.A. King, V. Leos-Barajas, J. Mills Flemming, A. Nielsen, G. Petris, L. Thomas. 2021. A guide to state-space modeling of ecological time series.

# Appendix S3: Symbolic method

As discussed in the main text, it is not necessarily possible to estimate every parameter and it is important to assess whether the model is identifiable. In Appendix S1, we demonstrate how to use the Hessian method to assess identifiability. As with other numerical methods, the Hessian method can be inaccurate and may not be able to distinguish between estimability, practical identifiability, and structural identifiability. In this Appendix, we demonstrate how to use the symbolic method with `Maple`. The symbolic method is an accurate way to assess structural identifiability, but is more complicated to use as it involves using a symbolic algebra package.

## S3 1 The symbolic method

As mentioned in the main text, identifiability refers to whether there is a unique representation of the SSM or multiple representations. Suppose that a particular SSM is represented by $M(\boldsymbol{\theta})$ with parameters $\boldsymbol{\theta}$. A model is globally identifiable if $M(\boldsymbol{\theta}_1) = M(\boldsymbol{\theta}_2)$ implies that $\boldsymbol{\theta}_1 = \boldsymbol{\theta}_2$. A model is locally identifiable if there exists a neighborhood of $\boldsymbol{\theta}$ where this is true. Otherwise a model is non-identifiable (e.g., Cole et al., 2010; Rothenberg, 1971).

As discussed in the main text, the symbolic method is based on the idea that a model can be represented by a vector of parameter combinations that uniquely define the model. This vector is referred to as an exhaustive summary. To investigate non-identifiability a derivative matrix is formed by differentiating each term of the vector with respect to each parameter and the rank of the derivative matrix is found. If the rank is less than the number of parameters, the model is non-identifiable or parameter redundant (Catchpole and Morgan, 1997; Cole et al., 2010). The rank is also the number of estimable parameters. In

non-identifiable models, estimable parameter combinations can be found by solving a set of partial differential equations (Catchpole et al., 1998; Cole et al., 2010). For state-space models (SSMs), suitable exhaustive summaries are given in Cole and McCrea (2016). Here, we use the expansion exhaustive summary, based on expanding the expectation and variance of the observation. This method can be used to investigate practical identifiability as well as structural identifiability by choosing an exhaustive summary that includes the specific data set (e.g., Cole et al., 2012).

In some more complex models the computer can run out of memory calculating the rank of the derivative matrix. Cole et al. (2010) and Cole and McCrea (2016) provide symbolic algebra methods for overcoming this issue. The alternative is a the hybrid symbolic-numerical method, which involves finding the derivative matrix using symbolic algebra, but then finding the rank at five random points in the parameter space (Choquet and Cole, 2012).

# S3 2 Implementation in `Maple`: example 1

Let us take the simple toy SSM of the main text, where the process equation is:

$$z_t = \beta z_{t-1} + \epsilon_t, \quad \epsilon_t \sim \mathrm{N}(0, \sigma_\epsilon), \tag{1}$$

and the observation equation is:

$$y_t = \alpha z_t + \eta_t, \quad \eta_t \sim \mathrm{N}(0, \sigma_\eta), \tag{2}$$

for $t = 1, ..., T$. Now, let us change the process equation to:

$$z_t = \beta_1 \beta_2 z_{t-1} + \epsilon_t, \quad \epsilon_t \sim \mathrm{N}(0, \sigma_\epsilon), \tag{3}$$

but keep the observation equation the same. The parameters in this new model are $\alpha, \beta_1, \beta_2$. We fix the parameters $\sigma_\eta = 0.1$ and $\sigma_\epsilon = 0.1$. If we reparametrize this new model so that $\beta = \beta_1\beta_2$, we can see that the original toy model is just a simpler version of this new model.

It would be impossible to find unique estimates for parameters $\beta_1$ and $\beta_2$, whereas a unique estimate of $\beta$ could theoretically be found. We will use this example to show how we can use the symbolic method to assess identifiability in `Maple`.

## Step 1: Load the procedures in `Maple`

The first line loads the internal package for linear algebra. The procedure `Dmat` finds the derivative matrix, the procedure `Estpar` finds the estimable parameter combinations and the procedure `Expannonlin` finds the expansion exhaustive summary. Note that the code has

been created to use $x$ rather than $z$ to represent the state equation following the notation used in Cole and McCrea (2016).

```
> with(LinearAlgebra) :
> Dmat := proc(se, pars)
  local DD1, i, j;
  description "Forms the derivative matrix";
  with(LinearAlgebra) :
  DD1 := Matrix(1 ..Dimension(pars), 1 ..Dimension(se)) :
  for i from 1 to Dimension(pars) do
     for j from 1 to Dimension(se) do
       DD1[i, j] := diff(se[j], pars[i])
     end do
   end do;
  DD1;
   end proc:
> Estpar := proc(DD1, pars, ret)
  local r, d, alphapre, alpha, PDE, FF, i, ans;
  description "Finds the estimable set of parameters for derivative matrix DD1. If ret = 1 returns
       alpha, PDEs, estimable parameter combinations. Otherwise returns estimable parameter
       combinations";
  with(LinearAlgebra) :
  r := Rank(DD1); d := Dimension(pars) - r :
  alphapre := NullSpace(Transpose(DD1)) : α := Matrix(d, Dimension(pars)) : PDE :=
       Vector(d) :
  FF := f(seq(pars[i], i = 1 ..Dimension(pars))) :
  for i from 1 to d do
       α[i, 1 ..Dimension(pars)] := alphapre[i] :
       PDE[i] := add(diff(FF, pars[j]) · α[i, j], j = 1 ..Dimension(pars)) :
  end do:
   if ret = 1 then
         ans := ⟨pdsolve({seq(PDE[i] = 0, i = 1 ..d)}), {alpha}, {PDE}⟩ :
   else
        ans := pdsolve({seq(PDE[i] = 0, i = 1 ..d)}) :
   end if:
   ans :
  end proc:

> Expannonlin := proc(xt, yt, x0, n)
   local i, kappa, xx, yy;
  description "Finds the exhaustive summary for a non-linear expansion method with n terms.
       (Limited to a single variable)";
  xx := Vector(n) ;
   yy := Vector(n);
   xx[1] := eval(eval(xt, t = 1), x[0] = x0);
   yy[1] := eval(eval(yt, t = 1), x[1] = xx[1]);
   kappa := ⟨yy[1]⟩ :
    for i from 2 to n do
       xx[i] := eval(eval(xt, t = i), x[i − 1] = xx[i − 1]);
       yy[i] := eval(eval(yt, t = i), x[i] = xx[i]);
       kappa := ⟨kappa, yy[i]⟩;
   end do:
   kappa := convert(kappa, Vector);
   end proc:
```

## Step 2: Enter the expectation of the state equation and the observation equation

```
> Ex := beta[1]·beta[2]·x[t − 1];
```

$$Ex := \beta_1 \beta_2 x_{t-1}$$

```
> Ey := alpha·x[t];
```

$$Ey := \alpha x_t$$

## Step 3: Create the expansion exhaustive summary

x0 represents the initial value of $z(t)$, which here is a fixed generic value. We expand to 3 terms as there are 3 parameters. (If there are parameters in the error terms, we also need to expand the variance, which we demonstrate in the next example.)

```
> kappa := Expannonlin(Ex, Ey, x0, 3);
```

$$\kappa := \begin{bmatrix} \alpha \beta_1 \beta_2 x0 \\ \alpha \beta_1^2 \beta_2^2 x0 \\ \alpha \beta_1^3 \beta_2^3 x0 \end{bmatrix}$$

## Step 4: Create a vector of the parameters

```
> pars := ⟨alpha|beta[1]|beta[2]⟩;
```

$$pars := \begin{bmatrix} \alpha & \beta_1 & \beta_2 \end{bmatrix}$$

## Step 5: Find the derivative matrix and its rank

```
> D1 := Dmat(kappa, pars);
```

$$D1 := \begin{bmatrix} \beta_1 \beta_2 x0 & \beta_1^2 \beta_2^2 x0 & \beta_1^3 \beta_2^3 x0 \\ \alpha \beta_2 x0 & 2 \alpha \beta_1 \beta_2^2 x0 & 3 \alpha \beta_1^2 \beta_2^3 x0 \\ \alpha \beta_1 x0 & 2 \alpha \beta_1^2 \beta_2 x0 & 3 \alpha \beta_1^3 \beta_2^2 x0 \end{bmatrix}$$

```
> r := Rank(D1);
```

$$r := 2$$

In this case, the rank is 2, but there are 3 parameters. This again confirms that the model is non-identifiable.

### Step 6: Find combination of estimable parameters

If the model is non-identifiable we can then also find the estimable parameter combinations. This is a reparameterization of the parameters that are identifiable.

```
> Estpar(D1, pars, 0);
                    {f(α, β1, β2) = _F1(α, β1 β2)}
```

In this case, the estimable parameter combinations are $\alpha$, $\beta_1\beta_2$. This means that in this model we could theoretically find a unique maximum likelihood estimate for $\alpha$, but not for $\beta_1$ and $\beta_2$ individually. We could however find a unique maximum likelihood estimate for $\beta = \beta_1\beta_2$.

## S3 3 Implementation in `Maple`: example 2

Below we show how to check identifiability for the original toy model used in the main text and described above. Here, we are interested in estimating parameters $\alpha$, $\beta$, $\sigma_\eta$ and $\sigma_\epsilon$. In the code we use $\sigma_1 = \sigma_\eta$ and $\sigma_2 = \sigma_\epsilon$. Here we assume that the initial state value is $z_0 = 0$. This exhaustive summary involves expanding the expectation and variance.

```
> Ex := beta·x[t − 1] : Ey := alpha·x[t] :
> Vx := beta^2·x[t − 1] + sigma[1]^2 : Vy := alpha^2·x[t] + sigma[2]^2 :
> kappa := convert(⟨Expannonlin(Ex, Ey, 0, 5), Expannonlin(Vx, Vy, 0, 5)⟩, Vector) :
> pars := ⟨alpha, beta, sigma[1], sigma[2]⟩ :
> D1 := Dmat(kappa, pars) :
> r := Rank(D1);
                    r := 3
> Estpar(D1, pars, 0);
                    {f(α, β, σ1, σ2) = _F1(β, σ1 α, σ2)}
```

The rank is 3, but there are 4 parameters so the model is non-identifiable. The estimable parameter combinations are $\beta$, $\alpha\sigma_\eta$ and $\sigma_\epsilon$.

If the initial state value is non-zero then we use the code below. Since we are using $x$ instead of $z$, the initial state value, $x_0$, in this case is not set to 0. Notice, how the value in the `Expannonlin` for $x_0$ is not 0 anymore, but simply $x_0$.

```
> Ex := beta·x[t − 1] : Ey := alpha·x[t] :
> Vx := beta^2·x[t − 1] + sigma[1]^2 : Vy := alpha^2·x[t] + sigma[2]^2 :
> kappa := convert(⟨Expannonlin(Ex, Ey, x0, 5), Expannonlin(Vx, Vy, 0, 5)⟩, Vector) :
> pars := ⟨alpha, beta, sigma[1], sigma[2]⟩ :
> D1 := Dmat(kappa, pars) :
> r := Rank(D1);
                                        r := 4
```

Now the rank is 4. Thus, the model is identifiable. This identifiable model has a nested submodel ($x_0 = 0$), which is non-identifiable. Caution is needed when using this model as it maybe near redundant, especially if $x_0$ is close to zero.

As mentioned above, for some complex models, it may be too hard to compute and one can use an hybrid symbolic-numerical method. The `Maple` code for the hybrid method for the example when $z_0 = 0$ is:

```
> Hybrid :=proc(D1, pars, ret)
  local results, j, numpars, D1rand, ans :

    description "This procedure finds the rank and alpha for the hybrid-symbolic-numeric
    method. If ret = 1 returns full results. Otherwise returns model rank.";
  results := Matrix(5, 2) :
  for j from 1 to 5 do
    numpars := seq(pars[i] = evalf(rand( )/1000000000000), i = 1 ..Dimension(pars)) :
    D1rand := eval(D1, {numpars});
    results[j, 1] := Rank( D1rand);
    results[j, 2] := NullSpace(Transpose(D1rand)) :
  end do:
  if ret = 1 then
      ans := results :
  else
      ans := max(results[1 ..5, 1]) :
  end if:
  ans :
  end proc:
> Hybrid(D1, pars, 0)
                              3
```

This also shows the model has rank 3 and is non-identifiable.

# Literature Cited


Catchpole, E. A. and Morgan, B. J. T. (1997). Detecting parameter redundancy. *Biometrika*, 84:187–196.

Catchpole, E. A., Morgan, B. J. T., and Freeman, S. N. (1998). Estimation in parameter-redundant models. *Biometrika*, 85:462–468.

Choquet, R. and Cole, D. J. (2012). A hybrid symbolic-numerical method for determining model structure. *Mathematical Biosciences*, 236:117–125.

Cole, D. J. and McCrea, R. S. (2016). Parameter redundancy in discrete state-space and integrated models. *Biometrical Journal*, 58:1071–1090.

Cole, D. J., Morgan, B. J. T., Catchpole, E. A., and Hubbard, B. A. (2012). Parameter redundancy in mark-reovery models. *Biometrical Journal*, 54:507–523.

Cole, D. J., Morgan, B. J. T., and Titterington, D. M. (2010). Determining the parametric structure of models. *Mathematical Biosciences*, 228:16–30.

Rothenberg, T. J. (1971). Identification in parametric models. *Econometrica*, 39:577–591.
