# Supplementary material for: A guide to state-space modeling of ecological time series
Source: arXiv:2002.02001 ancillary file (2021-03-12)
Supplement: Supplementary file 3 [file Appendix_S4.pdf]

**Supporting Information.** Auger-Méthé, M., K. Newman, D. Cole, F. Empacher, R. Gryba, A.A. King, V. Leos-Barajas, J. Mills Flemming, A. Nielsen, G. Petris, L. Thomas. 2021. A guide to state-space modeling of ecological time series.

# Appendix S4: Bayesian information criteria

## S4 1 Deviance Information Criterion

The Deviance Information Criterion (DIC) uses a formulation similar to the Akaike Information Criterion (AIC) (Gelman et al., 2014; Hooten and Hobbs, 2015):

$$\text{DIC} = -2 \log L(\hat{\boldsymbol{\theta}}_{\text{POST}}|\mathbf{y}) + 2p_{\text{DIC}}. \tag{1}$$

Here, the measure of fit, $L(\hat{\boldsymbol{\theta}}_{\text{POST}}|\mathbf{y})$, is the likelihood of the model at the mean of the posterior distribution of the parameters rather than at the MLE. There are alternatives for how to calculate the effective number of parameters (Gelman et al., 2014), $p_{\text{DIC}}$, but a common one is $-2$ times the difference between the posterior mean log likelihood and the log likelihood evaluated at the posterior mean of the parameter:

$$p_{\text{DIC}} = -2 \left( \int \log L(\boldsymbol{\theta}|\mathbf{y}) p(\boldsymbol{\theta}|\mathbf{y}) \mathrm{d}\boldsymbol{\theta} - \log L(\hat{\boldsymbol{\theta}}_{\text{POST}}|\mathbf{y}) \right). \tag{2}$$

In practice, this would be calculated as: $p_{\text{DIC}} = -2(\frac{1}{S}\sum_{s=1}^{S} \log p(\mathbf{y}|\boldsymbol{\theta}^s) - \log L(\hat{\boldsymbol{\theta}}_{\text{POST}}|\mathbf{y}))$, where $\boldsymbol{\theta}^s$ are samples from the posterior distribution. As for the Watanabe-Akaike Information Criterion (WAIC), to highlight the link to the predictive ability of the model, many Bayesians prefer to use a version of DIC without the $-2$ multiplier: $\text{DIC} = \log L(\hat{\boldsymbol{\theta}}_{\text{POST}}|\mathbf{y}) - p_{\text{DIC}}$ (e.g., Vehtari and Ojanen, 2012).

# S4 2 Watanabe-Akaike Information criterion

WAIC is defined as:

$$\text{WAIC} = -2\sum_{i=1}^{T} \log \int p(y_i|\boldsymbol{\theta})p(\boldsymbol{\theta}|\mathbf{y})\mathrm{d}\boldsymbol{\theta} + 2p_{\text{WAIC}}. \tag{3}$$

In practice, the log pointwise predictive density, $\sum_{i=1}^{T} \log \int p(y_i|\boldsymbol{\theta})p(\boldsymbol{\theta}|\mathbf{y})\mathrm{d}\boldsymbol{\theta}$, is calculated using $S$ samples from the posteriors: $\sum_{i=1}^{T} \log(\frac{1}{S}\sum_{s=1}^{S} p(y_i|\boldsymbol{\theta}^s))$. There are different ways to estimate the effective number of parameters, $p_{\text{WAIC}}$. Gelman et al. (2014) recommend using $\sum_{i=1}^{T} \text{Var}_{\text{POST}}(\log p(y_i|\boldsymbol{\theta}))$ as it gives results closer to the leave-one-out cross validation. In practice, it can be computed as $\sum_{i=1}^{T}(\frac{1}{S-1}\sum_{s=1}^{S}(\log p(y_i|\boldsymbol{\theta}^s) - \overline{\log p(y_i|\boldsymbol{\theta}^*)})^2)$, where $\overline{\log p(y_i|\boldsymbol{\theta}^*)}$ is the mean log probability of data point $y_i$ across all $S$ parameter samples.

A potential solution to the dependence issues mentioned in the main text could be to write $\log p(y_i|\boldsymbol{\theta}^s)$ so that only observations up to the previous time step are used: $\log p(y_1|\boldsymbol{\theta}^s) + \sum_{t=2}^{i} \log p(y_t|\mathbf{y}_{1:t-1}, \boldsymbol{\theta}^s)$. This should be further explored.

# Literature Cited


Gelman, A., Hwang, J., and Vehtari, A. (2014). Understanding predictive information criteria for Bayesian models. *Statistics and Computing*, 24:997–1016.

Hooten, M. B. and Hobbs, N. T. (2015). A guide to bayesian model selection for ecologists. *Ecological Monographs*, 85:3–28.

Vehtari, A. and Ojanen, J. (2012). A survey of Bayesian predictive methods for model assessment, selection and comparison. *Statistics Surveys*, 6:142–228.
