# Supplementary material for: A guide to state-space modeling of ecological time series
Source: arXiv:2002.02001 ancillary file (2021-03-12)
Supplement: Supplementary file 4 [file Appendix_S1.pdf]

**Supporting Information.** Auger-Méthé, M., K. Newman, D. Cole, F. Empacher, R. Gryba, A.A. King, V. Leos-Barajas, J. Mills Flemming, A. Nielsen, G. Petris, L. Thomas. 2021. A guide to state-space modeling of ecological time series.

## Appendix S1: Fitting and evaluating state-space models in R

The goal of this appendix is to demonstrate multiple ways in which state-space models (SSMs) can be fitted and validated in R. This appendix contains two chapters. The first chapter uses the toy model presented in the main text to demonstrate a wide range of tools and packages that can be used to fit SSMs. This first chapter is the most substantial part of the appendix. In particular, section S1 1.3 introduce the reader to a variety of different packages that can be used to fit SSMs. Each of the subsections of section S1 1.3 introduces one package and can be looked at more-or-less independently. However, to be able to jump to one of these subsections, one should read section S1 1.1 and run the code in section S1 1.2 first. The second chapter presents a few ways in which a more complex movement SSM can be fitted in R. The goal of this second chapter is to show how to handle some of the complexities absent in the toy model. These two chapters will provide a starting point for any researcher interested in fitting SSMs to their data.

Note on object notation. We tried to be as consistent as possible with the notation for R objects. In addition, we tried to create names that were not overly long. Our general structure for object names is: object type, followed by model name, followed by the main tool explored in the section. For example, `m0pD1m` is the model object (hence `m`), for the toy model with fixed parameters and thus no parameters to estimate (hence `0p`), for the package `d1m`. The most recurrent object labels are: `m` for model object, `f` for fitted model (e.g. the object returned by an optimizer), `zf` filtered state estimates, and `zs` smoothed state estimates. The main models explored are:

- `0p`: toy model with the parameters fixed to their true values,
- `2p`: toy model with  $\alpha$  and  $\beta$  fixed to their true values and the two standard deviations estimated,
- `4p`: toy model with all four parameters estimated,
- `Mis`: toy model with misspecified parameters, and
- `pb`: model for polar bear movement data.

# Chapter 1

## Introducing the tools with simple univariate linear Gaussian state-space models

The goal of this first section is to introduce most of the tools we will use in this Appendix with a set of very simple, nested SSMs. These models are univariate linear Gaussian SSMs, also known as normal dynamic linear models. They differ in the number of parameters to estimate, and one of them is the toy model used in the main text. We purposely start with simplistic models that we will fit to simulated data to present the basic concepts of the methods, the R packages, and the languages we will use. These simple models are not linked to an ecological example; they are just teaching tools.

### S1 1.1 The toy model

While SSMs can be quite complex, the simplest and original SSMs are linear and have Gaussian distributions. For a univariate time series, a simple linear Gaussian SSM consists of two equations for two time series. For example, the toy model described in the main text has the two following equations.

The process equation (or state equation) is:

$$z_t = \beta z_{t-1} + \epsilon_t, \quad \epsilon_t \sim N(0, \sigma_p^2), \quad (1.1)$$

where  $z_t$  is the state value at time  $t$ , for  $t = 1, \dots, T$  and  $\beta$  represents the autocorrelation in the state values. The states are generally unknown, i.e., cannot be observed directly, and are sometimes referred to as latent states or hidden states. This equation represents the evolution of the hidden state as a correlated random walk. The equation implies that there is some stochasticity in the process. This stochasticity is often referred as process variation and is here described by a Normal (Gaussian) distribution with standard deviation  $\sigma_p$ . For simplicity, we set the initial state value to be 0, i.e.,  $z_0 = 0$ .

The observation equation (or measurement equation) is:

$$y_t = \alpha z_t + \eta_t, \quad \eta_t \sim N(0, \sigma_o^2), \quad (1.2)$$

where  $y_t$  is the observation at time  $t$ , for  $t = 1, \dots, T$  and  $\alpha$  is a constant of proportionality that represents any systematic discrepancy between the observations and the states (e.g., the average detection rate). This equation links the observation at time  $t$  to the underlying state at that time. The equation implies that we are observing the process with error. This error term is often referred as the observation error and, here, is described by a Normal distribution with standard deviation  $\sigma_o$ .

This model has four parameters:  $\alpha, \beta, \sigma_o, \sigma_p$ . It is sometimes difficult to accurately estimate all four parameters, something we will demonstrate in the sections below. It is useful to explore a simpler model, where we fix two of the parameters and only have two parameters to estimate. In the simpler model, we fix both  $\alpha$  and  $\beta$  to 1, resulting in the following.

The process equation is now:

$$z_t = z_{t-1} + \epsilon_t, \quad \epsilon_t \sim N(0, \sigma_p^2), \quad (1.3)$$

and represents the evolution of the hidden state as a simple random walk. The observation equation is now:

$$y_t = z_t + \eta_t, \quad \eta_t \sim N(0, \sigma_o^2), \quad (1.4)$$

where we assume that there is no systematic bias in the observation (i.e. we observed the state with some error but the observations are not systematically smaller or larger than the states).

## S1 1.2 Simulated data

Here, we simulate data using the linear Gaussian SSM described in Eqs. 1.3-1.4 from section S1 1.1 above. This is the simpler model where two of the parameters are fixed ( $\alpha = \beta = 1$ ).

First, let us simulate the process for a time series of length 200 ( $T = 200$ ), with an additional time step for the state at  $t = 0$ . To be consistent with the model description, we set to  $z_0 = 0$ . We choose the standard deviation of the process variation,  $\sigma_p$ , to be 0.1.

```
# Create a vector that will keep track of the states
# It's of length T + 1 (+1 for t=0)
# T is not a good name in R, because of T/F, so we use TT
TT <- 200
z <- numeric(TT + 1)
# Standard deviation of the process variation
sdp <- 0.1
# Set the seed, so we can reproduce the results
set.seed(553)
# For-loop that simulates the state through time, using i instead of t,
for(i in 1:TT){
  # This is the process equation
  z[i+1] <- z[i] + rnorm(1, 0, sdp)
  # Note that this index is shifted compared to equation in text,
  # because we assume the first value to be at time 0
}
```

Let us plot the time series we have created.

```
plot(0:TT, z,  
     pch = 19, cex = 0.7, col="red", ty = "o",  
     xlab = "t", ylab = expression(z[t]), las=1)
```

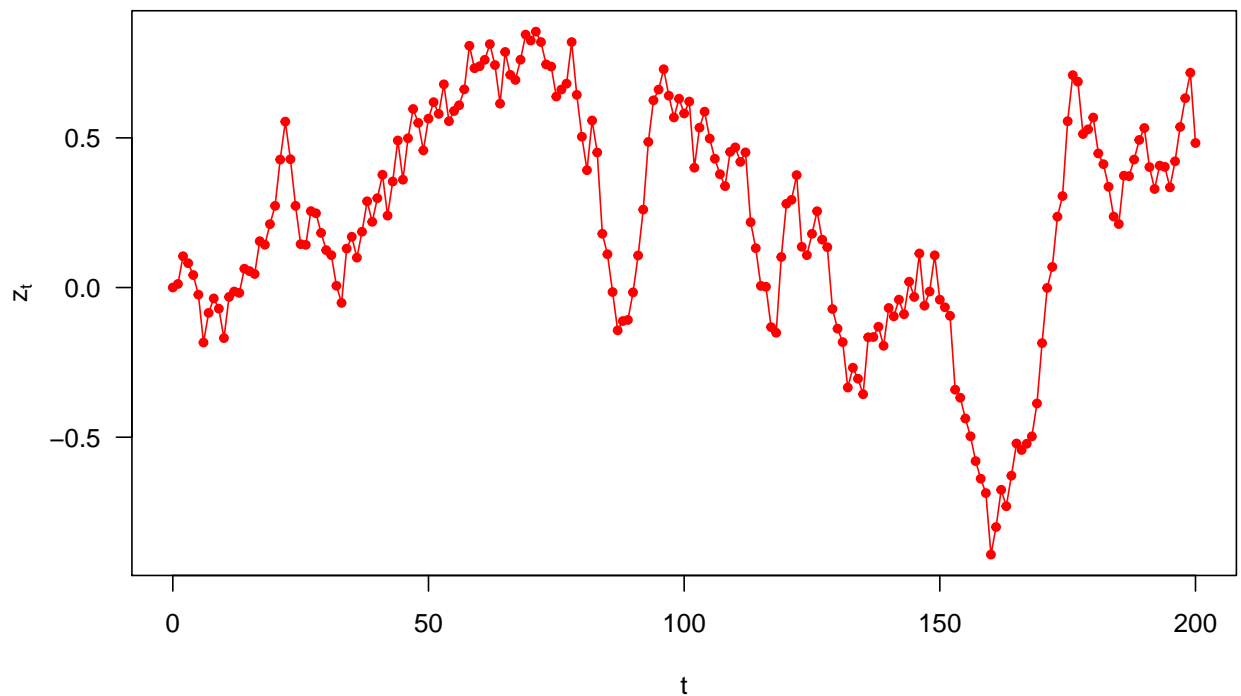

Figure S1.1: Simulated states.

Second, let us simulate the observations. We set the standard deviation of the observation error  $\sigma_o$  to 0.1.

```
# Create a vector that will keep track of the observations  
# It's of length T  
y <- numeric(TT)  
# Standard deviation of the observation error  
sdo <- 0.1  
# For t=1, ... T, add measurement error  
# Remember that z[1] is t=0  
y <- z[2:(TT+1)] + rnorm(TT, 0, sdo)
```

Let us plot both the observations and the states. From now on, we are adding extra space on the y-axis to leave space for the legend. Note that the space we assigned may not work for all figure sizes.

```

plot(1:TT, y,
     pch=3, cex = 0.8, col="blue", ty="o", lty = 3,
     xlab = "t", ylab = expression(z[t]),
     xlim = c(0,TT), ylim = c(min(y), max(y)+max(y)/5),
     las = 1)
points(0:TT, z,
       pch = 19, cex = 0.7, col="red", ty = "o")
legend("top",
       legend = c("Obs.", "True states"),
       pch = c(3, 19),
       col = c("blue", "red"),
       lty = c(3, 1),
       horiz=TRUE, bty="n", cex=0.9)

```

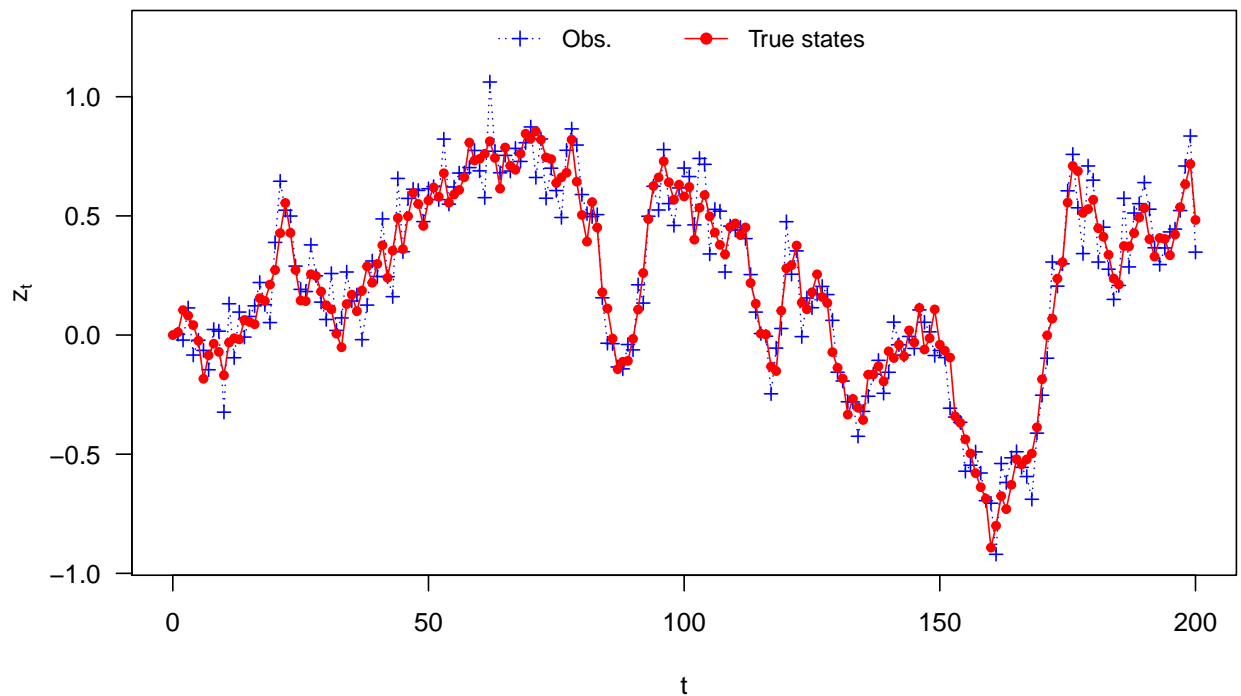

Figure S1.2: Simulated states and observations.

With real data, we usually only have the observations,  $y_t$ , and do not know the true states,  $z_t$ . However, simulated data allow us to see the discrepancies between the observed values and the values for the process they represent.

## S1 1.3 Fitting the model and checking your model fit

Each subsection of this section introduces the reader to a package that can be used to fit SSMs. While some concepts are explained incrementally through these subsections, they can be read more-or-less independently. However, before jumping to a subsection, section S1 1.1 should be read first. In addition, for the code in each subsection to work, one needs to first run the code in section S1 1.2.

### S1 1.3.1 DLM

We will start by fitting the model with the package `d1m` (Petrís, 2010). This package provides functions to apply the Kalman filter and smoother. For linear models such as our toy, the Kalman filter gives exact results and is thus particularly appropriate. `d1m` can be installed easily from CRAN.

```
library(d1m)
```

#### S1 1.3.1.1 Estimating state values when we know the parameter values

SSMs were originally developed to estimate state values with known parameter values. As such, we will first demonstrate filtering and smoothing of states with known parameters.

As a first step, we need to create a `d1m` object using the function `d1m`. This object will define the model, including defining the process and observation equations, and will contain the known parameter values. `d1m` defines the models as follow. Though our models involve only one equation each for the state and observation processes, `d1m` can accommodate multivariate models and data. Accordingly, we write the following in matrix form, though this is more generality than we presently require. The process equation is  $\mathbf{z}[t] = \mathbf{GG} * \mathbf{z}[t-1] + \mathbf{epsilon}[t]$ , where  $\mathbf{GG}$  is the matrix multiplier. In our more general toy model (Eq. 1.1),  $\mathbf{GG}$  corresponds to  $\beta$ , the autocorrelation in the state. In our simpler model (Eq. 1.3) and in the simulation,  $\mathbf{GG}$  is set to 1. The observation equation is  $y[t] = \mathbf{FF} * \mathbf{z}[t] + \mathbf{eta}[t]$ . Here,  $\mathbf{FF}$  is the matrix multiplier. In our more general toy model (Eq. 1.2), it corresponds to  $\alpha$ . In our simpler model (Eq. 1.4), and in the simulation,  $\mathbf{FF}$  is set to 1. In addition, as in our model description and simulation, we will define the initial state value as  $z_0 = 0$ . The mean value of the initial state is specified by `m0` in the `d1m` object and we will set it equal to 0. To fix the initial state to its mean value, we will the variance of the initial state, represented by `C0`, equal to 0. Finally, we will set the standard deviations of the process and observation equations,  $\sigma_p$  and  $\sigma_o$  to the values we used in the simulation (found in `sdp` and `sdo`). In `d1m`, we define the variance for these two equations with the arguments `W` for the process variation and `V` for the observation error. By definition, `d1m` assumes that the two stochastic components have Gaussian distributions.

```
# Create the d1m object
# The essential arguments to define the model are:
# m0 = initial value of the state, z[0]
# C0 = variance of the initial value
# GG = matrix multiplier in the State Eq: z[t] = GG*z[t-1] + epsilon[t]
# W = state process variance
```

```
# FF = matrix multiplier in the Obs. Eq:  $y[t] = FF*z[t] + eta[t]$ 
# V = observation error variance
mOpDlm <- dlm(m0=0, C0=0, GG=1, W=sdp^2, FF=1, V=sdo^2)
```

Now that we have a `dlm` object with known set parameter values, it is easy to estimate state values.

As discussed in the main text, there are three ways to estimate the state value at time  $t$ ,  $z_t$ . Here, we will explore two of them. The first is filtering, which means that we use the observations up to, and including, time  $t$ ,  $y_{1:t}$ . To do so, we use the function `dlmFilter`. This function requires as input the time series of observations in argument `y` and the `dlm` object defining the model in argument `mod`.

```
filterOpDlm <- dlmFilter(y=y, mod=mOpDlm)
```

The output from `dlmFilter` includes the filtered state values in component `m`. Because the time series includes the initial value, it has `TT+1` values. `dlmFilter` returns many other components, including variances. The variances are returned in terms of their singular value decomposition, see help file (`?dlmFilter`) for more information. One can reconstruct the filtering variances using the function `dlmSvd2var`.

```
fvarOpDlm <- unlist(dlmSvd2var(filterOpDlm$U.C,
                              filterOpDlm$D.C))
head(fvarOpDlm)

## [1] 0.000000000 0.005000000 0.006000000 0.006153846 0.006176471 0.006179775
```

We can use these estimated variances to create confidence intervals.

```
zfCIlOpDlm <- filterOpDlm$m + qnorm(0.025, sd = sqrt(fvarOpDlm))
zfCIuOpDlm <- filterOpDlm$m + qnorm(0.975, sd = sqrt(fvarOpDlm))
```

Let us plot the filtered values, with their confidence intervals, on the plot of true states and observations.

```
plot(1:TT, y,
     pch=3, cex = 0.8, col="blue", ty="o", lty = 3,
     xlab = "t", ylab = expression(z[t]),
     xlim = c(0,TT), ylim = c(min(y), max(y)+max(y)/5),
     las = 1)
points(0:TT, z,
       pch = 19, cex = 0.7, col="red", ty="o")
polygon(c(0:TT, TT:0),
        c(zfCIlOpDlm, rev(zfCIuOpDlm)),
        col=rgb(0,0,0,0.2), border=FALSE)
```

```

lines(0:TT, filterOpDlm$m,
      lwd=2)
legend("top",
      legend = c("Obs.", "True states", "Filter. states"),
      pch = c(3, 19, NA),
      col = c("blue", "red", "black"),
      lwd = c(1, 1, 2), lty = c(3, 1, 1),
      horiz=TRUE, bty="n", cex=0.9)

```

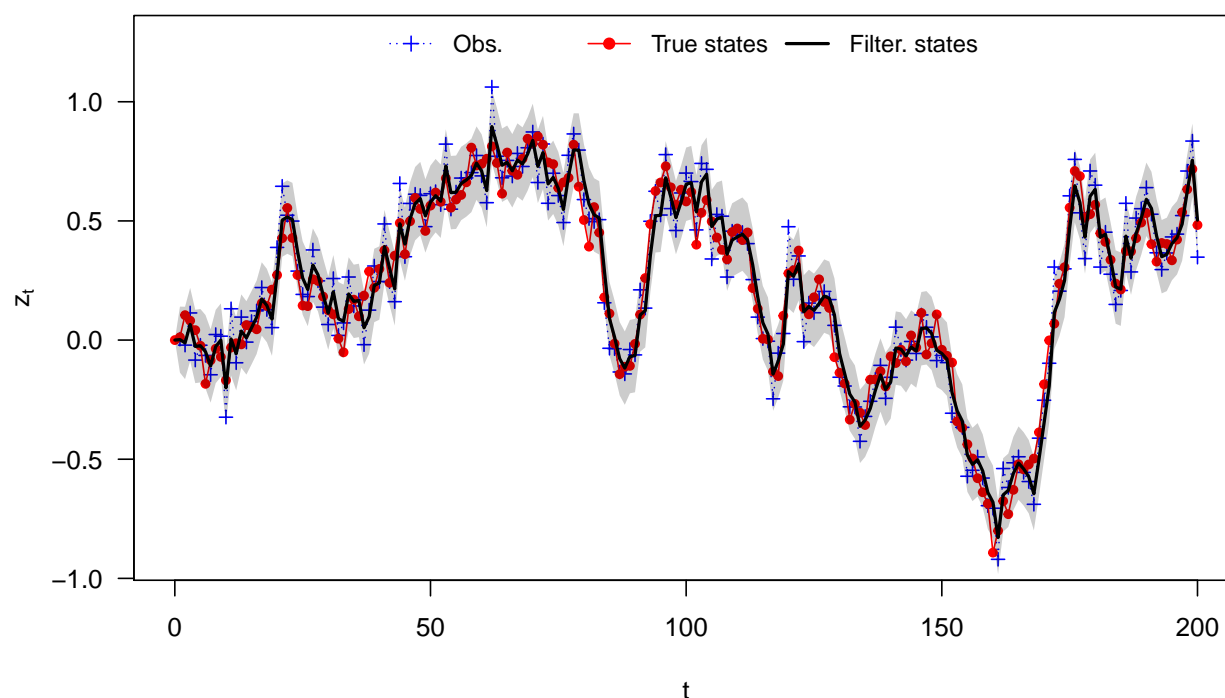

Figure S1.3: Estimates from the Kalman filter. The gray shaded region represents the confidence interval.

`d1m` also allows us to estimate state values using smoothing, in which case all observations  $y_{1:T}$  are used to estimate the state values at each time step,  $z_t$ . Here we use the function `d1mSmooth`. Again, we only need to provide the function the observations in argument `y` and the `d1m` object that defines the model in argument `mod`.

```
smoothOpD1m <- d1mSmooth(y=y, mod=mOpD1m)
```

The output from `d1mSmooth` includes the smoothed values in component `s`. Just like the filtered values, it includes the initial value. Just like for the filtering, we can create confidence intervals from the two variance components (U.S and D.S) returned by `d1mSmooth`.



```

svarOpDlm <- unlist(dlmSvd2var(smoothOpDlm$U.S,
                             smoothOpDlm$D.S))
zsCIlOpDlm <- smoothOpDlm$s + qnorm(0.025, sd = sqrt(svarOpDlm))
zsCIuOpDlm <- smoothOpDlm$s + qnorm(0.975, sd = sqrt(svarOpDlm))

```

For comparison, let us plot together both the filtered and smoothed values.

```

plot(1:TT, y,
     pch=3, cex = 0.8, col="blue", ty="o", lty = 3,
     xlab = "t", ylab = expression(z[t]),
     xlim = c(0,TT), ylim = c(min(y), max(y)+max(y)/5),
     las = 1)
points(0:TT, z, pch = 19, cex = 0.7, ty = "o", col="red")
polygon(c(0:TT, TT:0),
        c(zfCIlOpDlm, rev(zfCIuOpDlm)),
        col=rgb(0,0,0,0.2), border=FALSE)
lines(0:TT, filterOpDlm$m,
      lwd=2)
polygon(c(0:TT, TT:0),
        c(zsCIlOpDlm, rev(zsCIuOpDlm)),
        col=rgb(1,0.7,0.4,0.3), border=FALSE)
lines(0:TT, smoothOpDlm$s,
      col="darkgoldenrod1")
legend("top",
      legend = c("Obs.", "True states", "Filter. states", "Smooth. states"),
      pch = c(3, 19, NA, NA),
      col = c("blue", "red", "black", "darkgoldenrod1"),
      lwd = c(1, 1, 2, 1.5), lty = c(3, 1, 1, 1),
      horiz=TRUE, bty="n", cex=0.9)

```

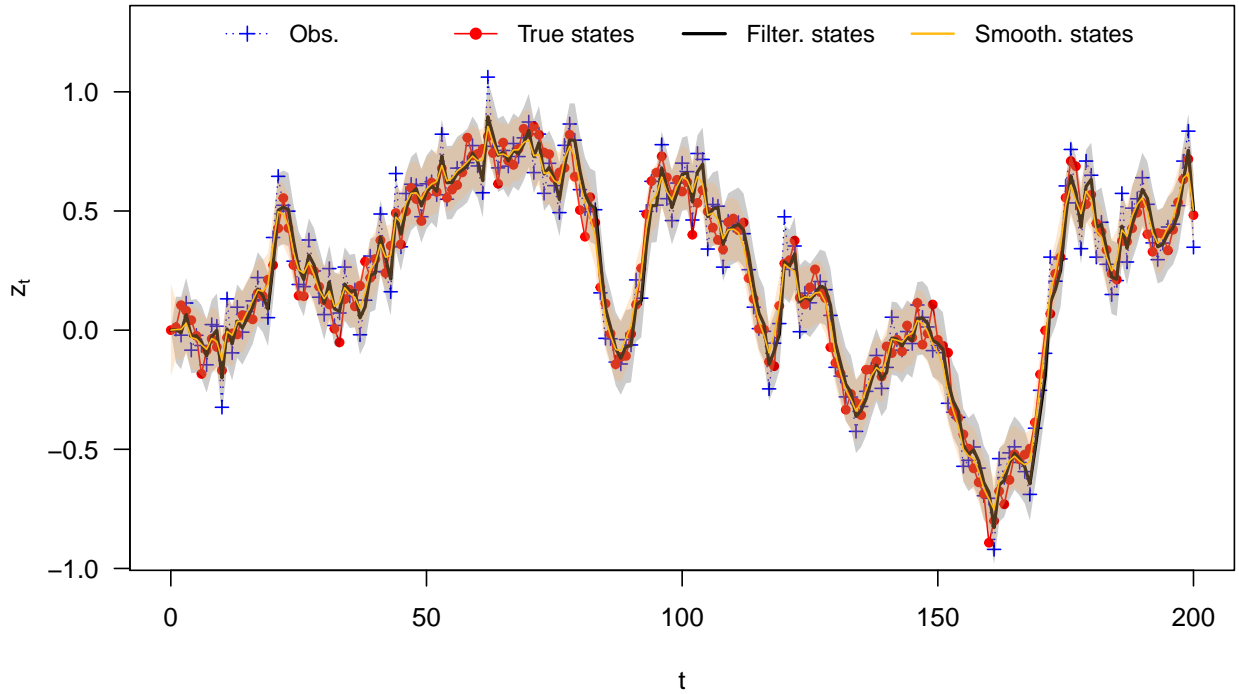

Figure S1.4: Estimates from the Kalman filter and smoother. The gray shaded region represents the confidence interval for the filtered states, while the orange shaded region represents the confidence interval for the smoothed states.

Note that the filtered and smoothed values differ and that the confidence intervals of the smoothed values are narrower than that of the filtered values.

#### S1 1.3.1.2 Estimating parameter and state values

In ecology, in most cases, we do not know the parameter values of our model, at least not all of them. As such, we need to estimate them. To do so with `d1m` requires 2 steps.

Step 1: Create a function that defines the model as a function of the parameter values to estimate.

So here, instead of creating a `d1m` object with fixed parameters, we write a function which has as sole argument a vector containing the parameter values. Furnished with a vector of parameters, this function constructs a `d1m` object with the given parameter values. Because we are estimating only the variances of the process variation and observation error, we re-use the model defined above, modified only in that  $W$  and  $V$  depend on the furnished parameter values. Note that we exponentiate the input values because we want the variance values to be positive and because in the next step we are not specifying bounds to the values that can be explored by the optimizer.

```
m2pDlm <- function(theta) {
  dlm(m0=0, C0=0, GG=1, W=exp(theta[1]), FF=1, V=exp(theta[2]))
}
```

As a note, we could have used one of `dlm` wrapper functions to write this model with less code. In the code chunk above, we could have replaced `dlm(m0=0, C0=0, GG=1, W=exp(theta[1]), FF=1, V=exp(theta[2]))` with `dlmModPoly(order=1, dW=exp(theta[1]), dV=exp(theta[2]))`. But to keep the introduction as general as possible we continue using the base `dlm` object function.

Step 2: Fit the model by maximizing the likelihood.

Here, we use the function `dlmMLE`, which uses the R function `optim` to maximize the likelihood. All we have to do is provide: the observations in argument `y`, the starting values for the parameters to estimate in argument `parm`, and the function to build the `dlm` object we just created.

Here, we used the parameter values used in the simulation as the starting values. Thus, we are potentially significantly helping the estimation process. With real data, we would not know the real value of the parameters and we may start very far from the maximum likelihood estimate (MLE). In some cases, the choice of starting values can affect the results. It is often recommended to call `dlmMLE` a few times with different starting value to increase the chance that `optim` finds the global maximum rather than a local maximum of the likelihood function.

```
f2pDlm <- dlmMLE(y=y, parm=c(log(sdp^2), log(sdo^2)),
  build=m2pDlm)
```

As `dlmMLE` will return values even if the optimizer had convergence problems, we need to check convergence. The value should be 0.

```
# Did it converged? i.e. does it has a value of 0?
f2pDlm$convergence

## [1] 0
```

It has converged.

We can now extract the parameter estimates. Because we exponentiated the values and `dlm` defines variance rather than standard deviation, we need to transform the values contained in `f2pDlm` to obtain the standard deviations.

```
sqrt(exp(f2pDlm$par))

## [1] 0.1174192 0.0914208
```

These estimates are close to their true values of 0.1.

Now to estimate the state values based on our model with the estimated parameter values, we will use the same methods as described in the section above. As a first step we need to define a `d1m` model object that contains the estimated parameter values. To do so, we just use the function we optimized.

```
# Create the d1m model object with the estimated parameters
mM1e2pD1m <- m2pD1m(f2pD1m$par)
```

Then, we can get filtered and smoothed state estimates.

```
# Use filtering to get state estimates
filter2pD1m <- d1mFilter(y=y, mod=mM1e2pD1m)

# Use smoothing to get state estimates
smooth2pD1m <- d1mSmooth(y=y, mod=mM1e2pD1m)
```

We can again get the confidence intervals for these state estimates.

```
# Variance of filtered values
fvar2pD1m <- unlist(d1mSvd2var(filter2pD1m$U.C,
                              filter2pD1m$D.C))

# CI of filtered estimates
zfCI12pD1m <- filter2pD1m$m + qnorm(0.025, sd = sqrt(fvar2pD1m))
zfCIu2pD1m <- filter2pD1m$m + qnorm(0.975, sd = sqrt(fvar2pD1m))

# Variance of smoothed values
svar2pD1m <- unlist(d1mSvd2var(smooth2pD1m$U.S,
                              smooth2pD1m$D.S))

# CI of smoothed estimates
zsCI12pD1m <- smooth2pD1m$s + qnorm(0.025, sd = sqrt(svar2pD1m))
zsCIu2pD1m <- smooth2pD1m$s + qnorm(0.975, sd = sqrt(svar2pD1m))
```

Now let us plot the results.

```
plot(1:TT, y,
     pch=3, cex = 0.8, col="blue", ty="o", lty = 3,
     xlab = "t", ylab = expression(z[t]),
     xlim = c(0,TT), ylim = c(min(y), max(y)+max(y)/5),
     las = 1)
points(0:TT, z,
```

```

    pch = 19, cex = 0.7, col = "red", ty = "o")
polygon(c(0:TT, TT:0),
        c(zfCIl2pDlm, rev(zfCIu2pDlm)),
        col=rgb(0,0,0,0.2), border=FALSE)
lines(0:TT, filter2pDlm$m,
      lwd=2)
polygon(c(0:TT, TT:0),
        c(zsCIl2pDlm, rev(zsCIu2pDlm)),
        col=rgb(1,0.7,0.4,0.3), border=FALSE)
lines(0:TT, smooth2pDlm$s,
      col="darkgoldenrod1")
legend("top",
      legend = c("Obs.", "True states", "Filter. states", "Smooth. states"),
      pch = c(3, 19, NA, NA),
      col = c("blue", "red", "black", "darkgoldenrod1"),
      lwd = c(1, 1, 2, 1.5), lty = c(3, 1, 1, 1),
      horiz=TRUE, bty="n", cex=0.9)

```

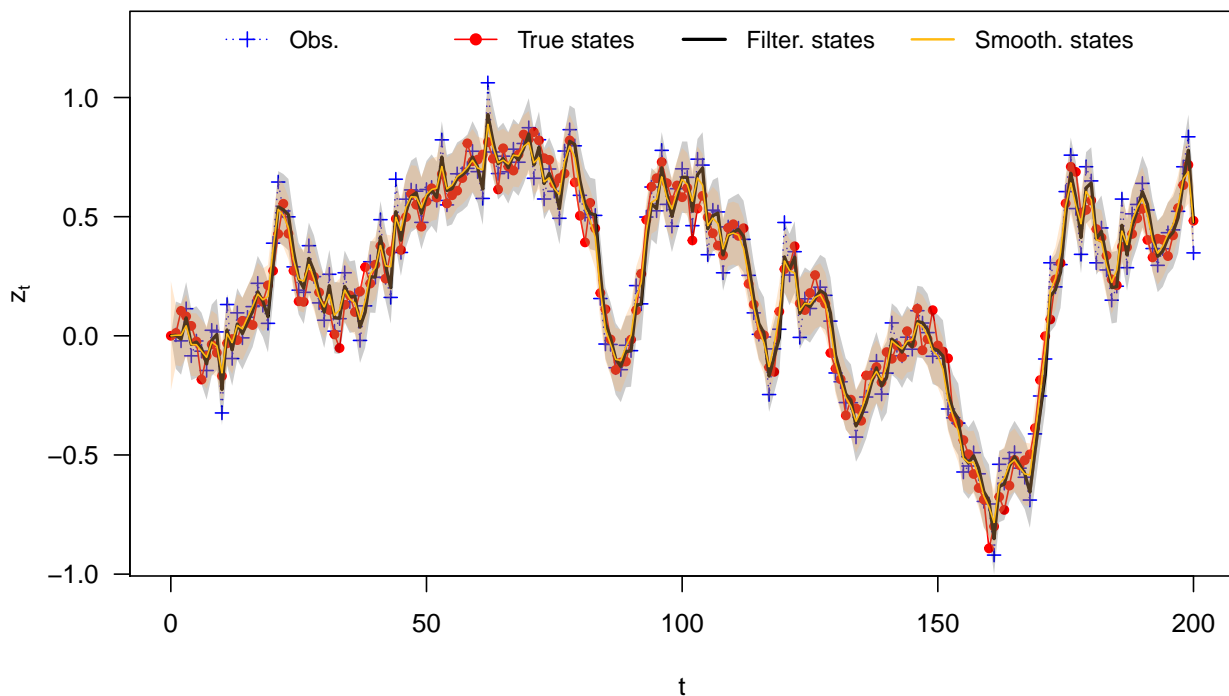

Figure S1.5: Estimates from the Kalman filter and smoother when the parameters are estimated.

### S1 1.3.1.3 Model comparison

Above we used the exact model we used to simulate the data, but in most cases there may be multiple ways to describe the data and we may want to explore different models and see which fits the data best.

Here, we will explore a slightly more complex model as an alternative. Instead of using the simplified model described in Eqs. 1.3-1.4, we will use the more general version (Eqs. 1.1-1.2). In this case, the two matrix multipliers (**FF** for  $\alpha$  and **GG** for  $\beta$ ) will be estimated. Since our simulations implicitly set these to 1, we hope for estimate values around 1.

Again, we will create the function that creates the **d1m** object, which will then be used to maximize the likelihood. The difference here is that we now also estimate  $\alpha$  and  $\beta$ .

```
# Create function to make a d1m object
m4pD1m <- function(theta) {
  d1m(GG=theta[1], W=exp(theta[2]), FF=theta[3], V=exp(theta[4]),
      m0=0, C0=0)
}
# Fit the model using maximum likelihood
f4pD1m <- d1mMLE(y=y, parm=c(1, log(sdp^2), 1, log(sdo^2)),
                build=m4pD1m)
# Did it converge? i.e. does it has a value of 0?
f4pD1m$convergence

## [1] 0
```

To compare the fit of this model to the fit of the previous model we can use AIC. The function **d1mMLE** returns the negative log likelihood and we can thus easily calculate the AIC value for each model ( $AIC = -2\ln(L) + k$ , where  $k$  is the number of estimated parameters and  $\ln(L)$  is the log-likelihood value). Our first model has two parameters to estimate, the two standard deviations. The second model, has two additional parameters to estimate:  $\alpha$  and  $\beta$ . As discussed in the main text other metrics could be used.

```
# AIC for simpler model (2 parameters to estimate)
aic2pD1m <- 2*f2pD1m$value + 2*2
# AIC for the more flexible model (4 parameters to estimate)
aic4pD1m <- 2*f4pD1m$value + 2*4
c(Original = aic2pD1m, Flexible = aic4pD1m,
  Difference = aic4pD1m - aic2pD1m)

##      Original      Flexible      Difference
## -511.3080550 -510.3661338      0.9419212
```

We can see that the best model according to AIC is the original model, the simple model we used to simulate the data, but only slightly so.

#### S1 1.3.1.4 Checking estimability and model fit with simulations

The first check one should do to assess whether the parameters and states of the model are estimable is to simulate the model and see whether the parameter and state values can be recovered (i.e., estimated accurately). Here, because we started with simulated data, most of the work is done.

We saw above that the parameter and state estimates were close to the simulated values, at least visually.

Now let us explore whether this is true with the more flexible model we have created. This model has the same structure as the one used to simulate data, but two additional parameters are estimated (rather than fixed) compared to the simpler model.

Let us look at the parameter values. Here because we have a combination of parameters with different transformations, we will first create a new `d1m` object and extract the values from it using the functions `GG`, `W`, `FF`, and `V`.

```
mM1e4pD1m <- m4pD1m(f4pD1m$par)
round(cbind("True" = c("beta"=1,"alpha"=1,
                      "sd Pro."=sdp, "sd Obs."=sdo),
          "Est" = c(GG(mM1e4pD1m),
                   FF(mM1e4pD1m),
                   sqrt(W(mM1e4pD1m)),
                   sqrt(V(mM1e4pD1m))))),3)

##           True    Est
## beta       1.0 0.966
## alpha      1.0 1.157
## sd Pro.    0.1 0.104
## sd Obs.    0.1 0.089
```

These parameter estimates are quite good, although the fact that we do not recover  $\alpha$  and  $\beta$  exactly may be explaining the slight AIC difference above.

As a note, this is a case where the starting values can really affect the parameter estimates. As an exercise, try to estimate this more complex model with the following starting values `c(1,0.1,1,0.1)` and see how this strikingly changes the parameter estimates.

To see how using the estimated values for  $\alpha$  and  $\beta$  affect the state estimates, we again use the filtering and smoothing functions from `d1m` but plug in the model with all four parameters estimated.

```
# Filter, using the d1m object created above
filter4pD1m <- d1mFilter(y=y, mod=mM1e4pD1m)
# Smooth, using the d1m object created above
smooth4pD1m <- d1mSmooth(y=y, mod=mM1e4pD1m)
# Plot the results
```

```

plot(1:TT, y,
     pch=3, cex = 0.8, col="blue", ty="o", lty = 3,
     xlab = "t", ylab = expression(z[t]),
     xlim = c(0,TT), ylim = c(min(y), max(y)+max(y)/5),
     las = 1)
points(0:TT, z,
       pch = 19, cex = 0.7, col = "red", ty = "o")
lines(0:TT, filter4pDlm$m,
      lwd=2)
lines(0:TT, smooth4pDlm$s,
      col="darkgoldenrod1")
legend("top",
      legend = c("Obs.", "True states", "Filter. states", "Smooth. states"),
      pch = c(3, 19, NA, NA),
      col = c("blue", "red", "black", "darkgoldenrod1"),
      lwd = c(1, 1, 2, 1.5), lty = c(3, 1, 1, 1),
      horiz=TRUE, bty="n", cex=0.9)

```

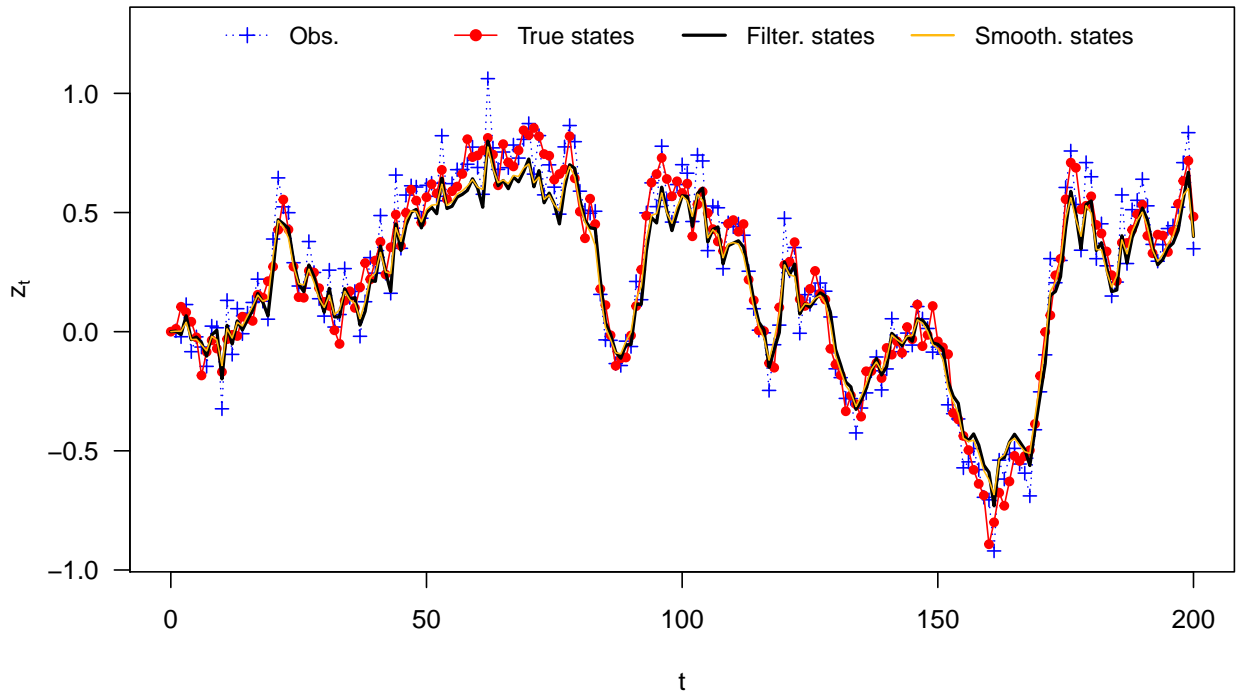

Figure S1.6: Estimates of the states from the Kalman filter and smoother when we use the estimated parameters from the more complex model (with 4 parameters).



At least visually, the more flexible model is capable of generally recovering the states. However, because the estimated value for  $\alpha$  is 1.157 when it should be 1, the state estimates are slightly biased.

To look at this bias more formally, we examine estimated vs simulated values using root mean square prediction error (RMSPE). Here, we will compare the state estimates when we: a) know all four parameter values, b) use the original model and only estimate the two standard deviations, and c) use the more flexible model with four parameters to estimate. We will do this for both filtering and smoothing results.

```
# Create two functions
# 1) To calculate the RMSPE
# 2) To plot estimated vs simulated state values

# Function to calculate RMSPE
rmspe <- function(zhat){
  sqrt(sum((z[-1]-zhat[-1])^2))
}

# Function to plot z vs zhat
pzz <- function(zhat,tx,cc="black"){
  plot(z[-1], zhat[-1],
       xlab=expression(z[t]), ylab=expression(hat(z)[t]), las=1,
       pch=19, col=cc, cex=0.5)
  abline(0,1)
  mtext(paste(tx, " RMSPE=",
              round(rmspe(zhat),2)), line=-1, cex=0.7)
}

# Known parameters - filtering
pzz(filterOpDlm$m, "Filter., Known par.", "black")

# Known parameters - smoothing
pzz(smoothOpDlm$s, "Smooth., Known par.", "darkgoldenrod1")

# Unknown variances only - filtering
pzz(filter2pDlm$m, "Filter., Unknown sd.", "black")

# Unknown variances only - smoothing
pzz(smooth2pDlm$s, "Smooth., Unknown sd.", "darkgoldenrod1")

# All unknown parameters - filtering
pzz(filter4pDlm$m, "Filter., Unknown all", "black")
```

```
# All unknown parameters - smoothing
pzz(smooth4pDlm$s, "Smooth., Unknown all", "darkgoldenrod1")
```

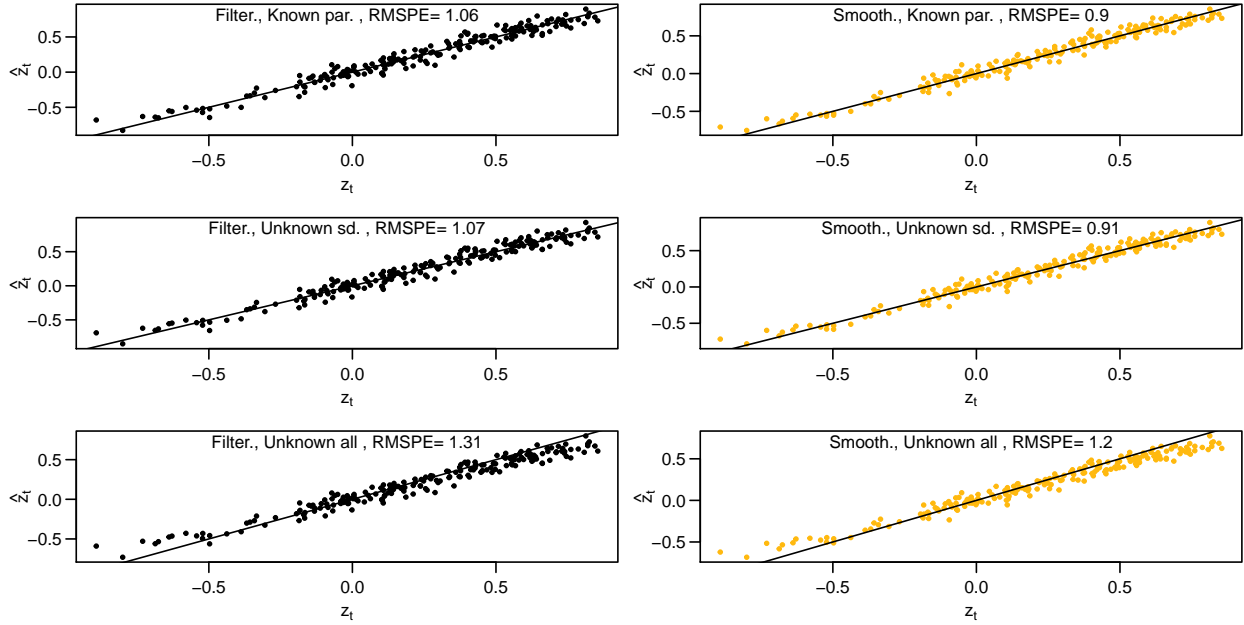

Figure S1.7: RMSPE for the Kalman filter and smoother estimates of three different models.

We can see a few things here. First the smoothing estimates are generally better in terms of RMSPE. That is because all of the data is used to estimate each states. We can also see that adding parameters to estimates decreases the accuracy of the state estimates. This drop in accuracy is particularly noticeable when we use the more flexible model, where all parameters are unknown. This is partly because the estimated  $\alpha$  parameter indicates the observations are 1.157 the size of the states. Thus, for negative observations, we generally estimate larger state values. For positive observations, we generally estimate smaller state values than we would if  $\alpha$  was 1 as in the simulation. That is why the points in the last row do not fall on 1:1 line.

#### S1 1.3.1.5 Looking at model assumptions with residuals

As discussed in the main text, assessing model fit with real data often involves looking at residuals. This is more complicated with SSMs, because we have time-series data. As discussed in the main text, we do not recommend using conventional residuals (sometime referred as response residuals) . Instead we recommend to use the one-step-ahead residuals. However, for demonstrative purposes, we will start by demonstrating the problem with these conventional residuals, which are defined as:

$$e_{t|1:T} = y_t - \hat{y}_{t|1:T}, \quad (1.5)$$

where  $\hat{y}_{t|1:T}$  is the predicted observation value at time  $t$ . In our toy example (Eqs. 1.1 - 1.2),

$$\hat{y}_{t|1:T} = \hat{\alpha} \hat{z}_{t|1:T}, \quad (1.6)$$

where  $\hat{z}_{t|1:T}$  is the smoothed estimate of the state value at time  $t$  and  $\hat{\alpha}$  is the estimated constant of proportionality. For our simplified model (Eqs. 1.3 - 1.4), we set  $\alpha = 1$ . As such, the predicted observation value is simply:

$$\hat{y}_{t|1:T} = \hat{z}_{t|1:T}. \quad (1.7)$$

Below we calculate the conventional residuals.

```
# Conventional residuals based on smoothed state values
resR2pDlm <- y - smooth2pDlm$s[-1]
```

Since this is the model we used to simulate the data, thus the true model, there should be no pattern in the residuals.

```
# Plot residuals vs time
plot(resR2pDlm,
     ylab="Conventional residuals", xlab="t",
     pch=19, cex=0.8, las=1)
abline(h=0, col="hotpink")
```

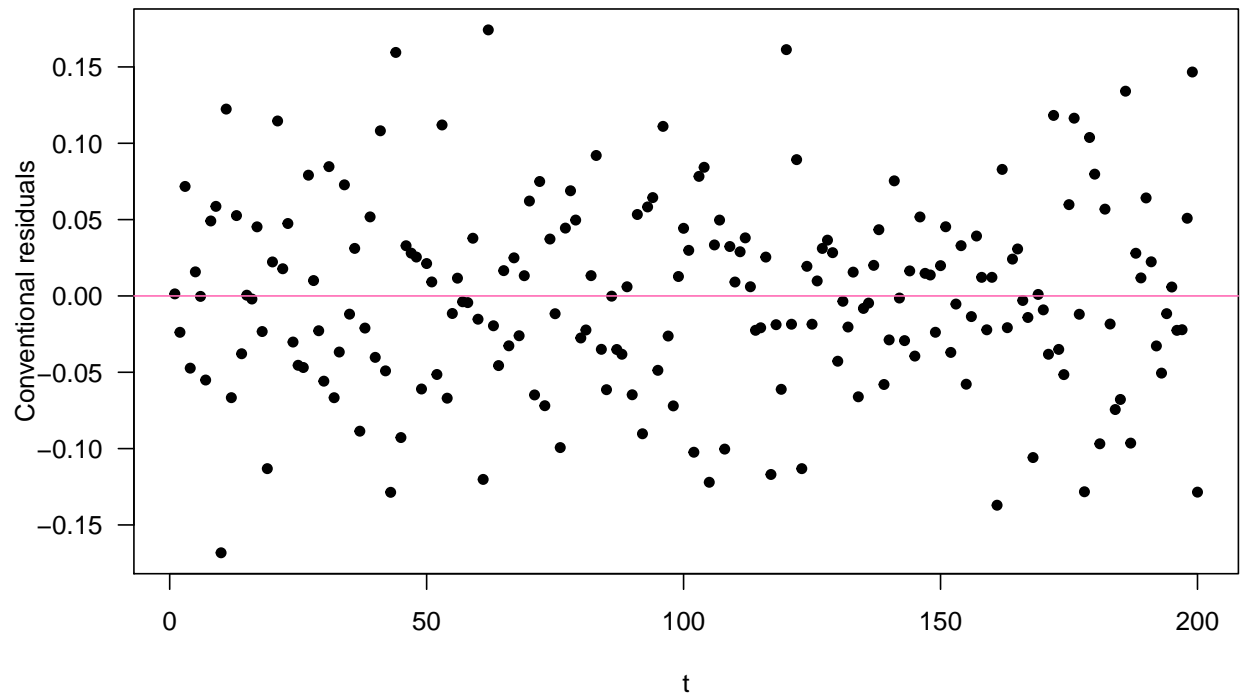

Figure S1.8: Conventional residuals.

As mentioned in the main text, it is common to standardize residuals by dividing the residuals by their standard deviation. As `dlmSmooth` returns the variance of the smoothing errors for the states,  $S_t$ , but not of the observations, we need calculate the observation variance as:  $Q_t = \alpha^2 S_t + \sigma_o^2$ . Here,  $\alpha$  is set to 1 and we use the estimated observation error variance.

```
# Standardizing the residuals
sdRespRes2pDlm <- sqrt(unlist(dlmSvd2var(smooth2pDlm$U.S,
                                         smooth2pDlm$D.S))[-1] +
                        exp(f2pDlm$par[2])))
resRS2pDlm <- resR2pDlm/sdRespRes2pDlm
```

For linear Gaussian models, we expect the standardized residuals to come from a standard normal distribution. We can then use deviations from this standard normal to assess whether the data are violating assumptions of the model

```
hist(resRS2pDlm, breaks=50, freq=FALSE,
     main="", ylab="Prob.", xlab=expression(e[t]),
     las=1, col="darkgrey")
box()
curve(dnorm, -3, 3, add=TRUE, col="hotpink", lwd=3)
qqnorm(y=resRS2pDlm,
      main="", pch=16, cex=0.8, las=1)
qqline(y=resRS2pDlm, col="hotpink", lwd=2)
```

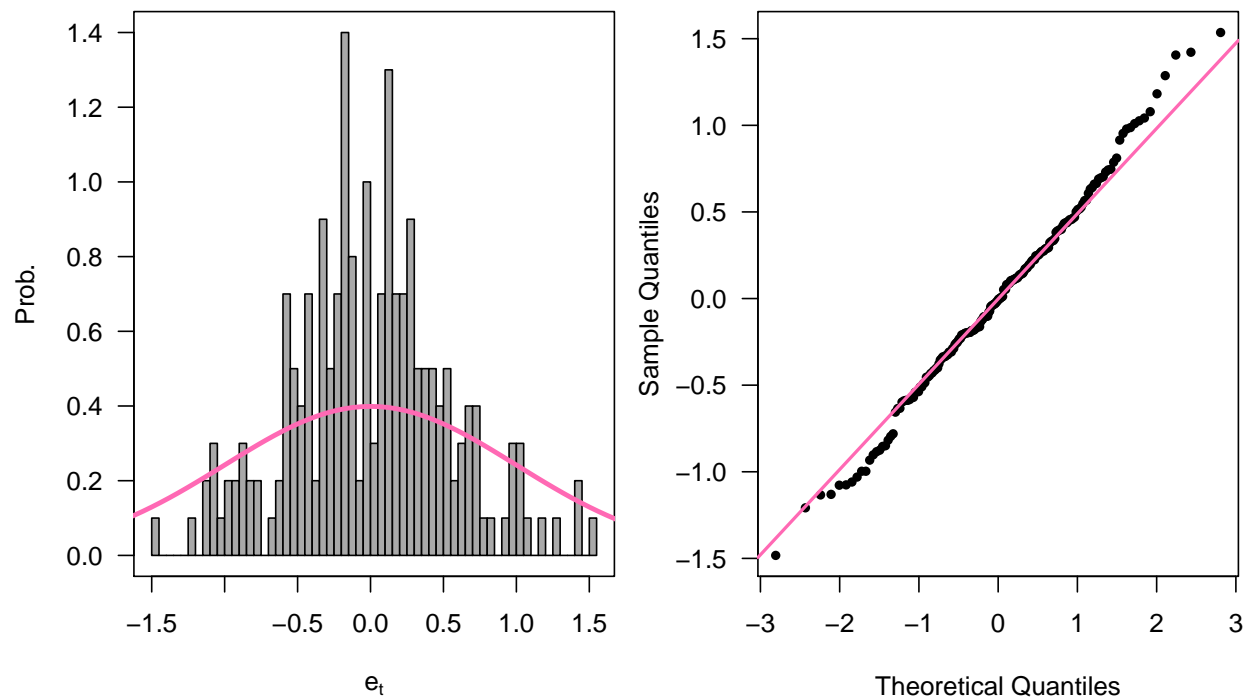

Figure S1.9: Comparison of the standardized conventional residuals and standard normal distribution.

Not terrible, but not perfect. It looks like we are having smaller residuals than expected by a standard normal. Is there any serial correlation?

```
acf(resRS2pDlm, las=1, main="")
```

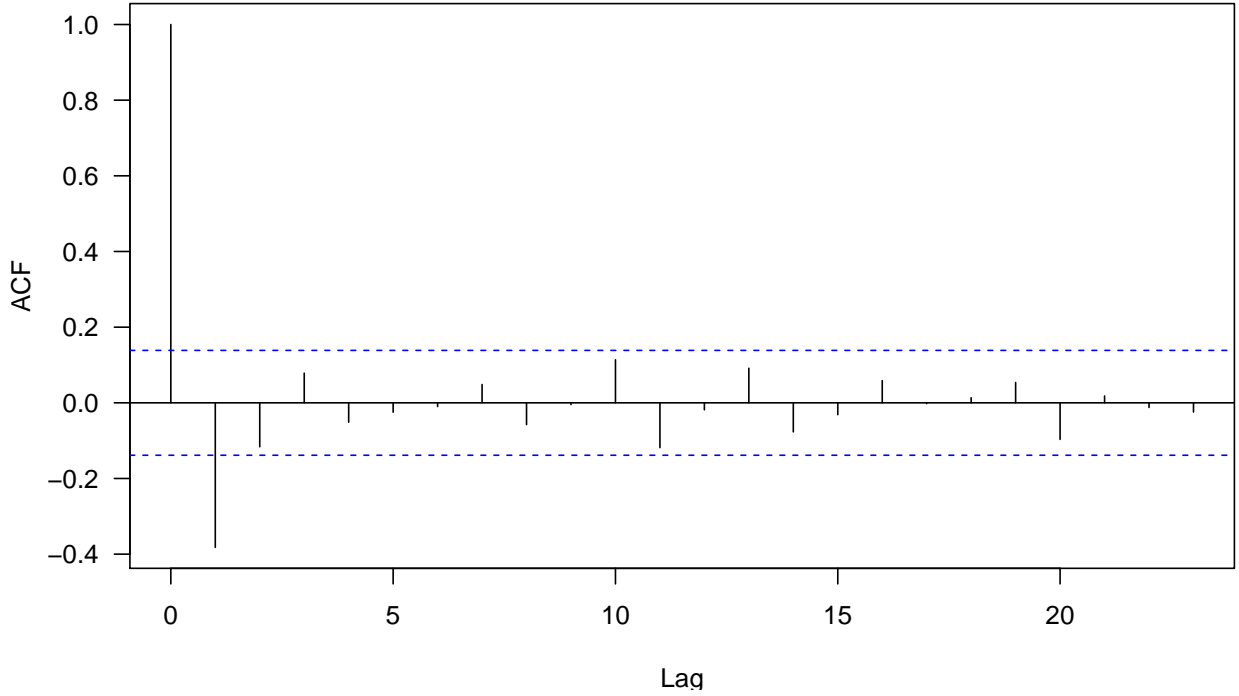

Figure S1.10: Autocorrelation function of the standardized conventional residuals.

As for all time series, using these simple residuals are not useful as they do not account for the autocorrelation in the data. Here, we can see negative autocorrelation in the residuals for the first time lag.

Instead, one-step-ahead (or prediction error) residuals are recommended. These one-step-ahead residuals account for the autocorrelation in the data that is explicitly modeled in the process equation. The one-step-ahead residuals are defined as:

$$e_{t|1:t-1} = y_t - \hat{y}_{t|1:t-1}, \quad (1.8)$$

where the subscript  $t|1:t-1$  indicates that we predict the value of  $y_t$  based on observation up to  $t-1$ . In the case of our simplified model (Eqs. 1.3 - 1.4), where  $\alpha = 1$ , the predicted observation value is simply:

$$\hat{y}_{t|1:t-1} = \hat{z}_{t|1:t-1}. \quad (1.9)$$

Because the filtering process in the Kalman filter requires the computation of the one-step-ahead predictive (or forecast) distribution of the observation at time  $t$ ,  $y_{t|1:t-1}$  (see main text), `d1mFilter` conveniently keeps track and returns the mean of the one-step-ahead predictive distribution. This mean can be considered the one-step-ahead prediction of the observation at time  $t$  and thus can be used to calculate the one-step-ahead residuals. These values are contained in the element `f` (for forecast) from the object returned by the `d1mFilter` function and we could use these to calculate the one-step-ahead residuals. Conveniently, `d1m` has a `residuals` function that calculates the one-step-ahead residuals and gives one the option to choose between the raw or the standardized version of the residuals.

Let us start with the unstandardized version of the one-step-ahead residuals.

```
res2pDlm <- residuals(filter2pDlm, type= "raw")
```

The function `residuals` returns both the residuals found in `res` and their standard deviation found in `sd`.

Again, we used the simple, true model and we do not expect to find patterns in the residuals. Now let us determine whether this is the case.

```
plot(res2pDlm$res, ylab="One-step-ahead residuals", xlab="t",  
     pch=19, cex=0.8, las=1)  
abline(h=0, col="hotpink")
```

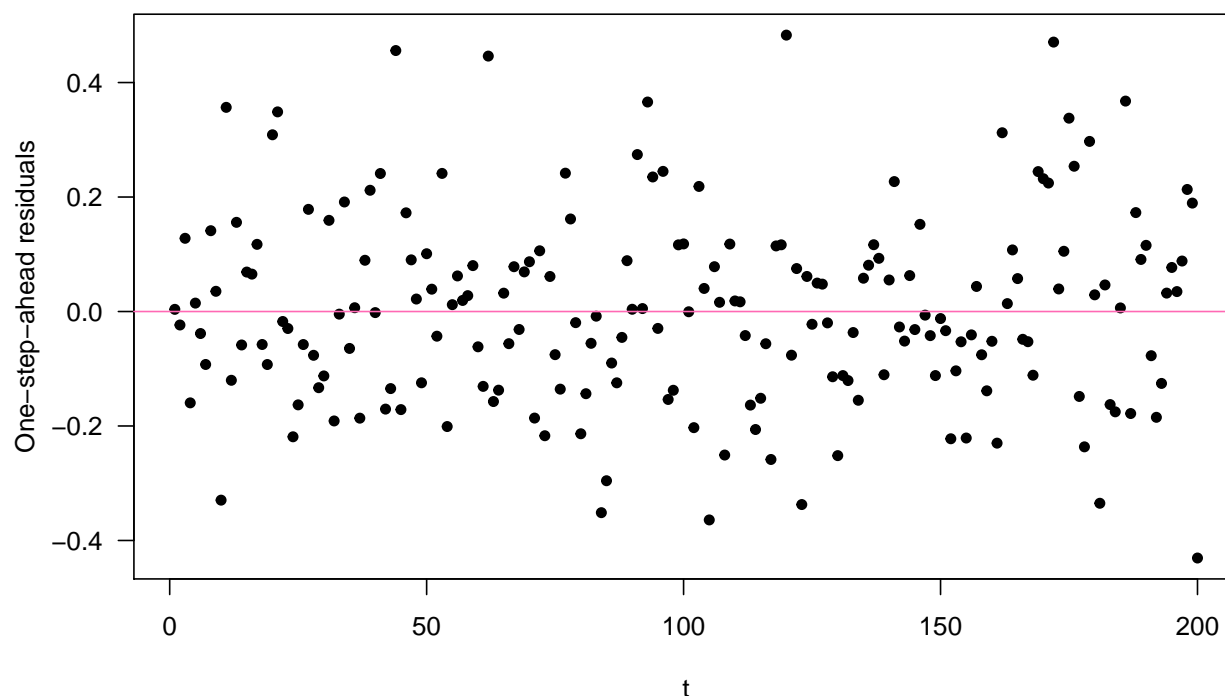

Figure S1.11: One-step-ahead residuals.

Just as for the conventional residuals, there are no obvious patterns in the residuals. There is, however, a marked difference in the magnitude of the residuals, with the magnitude of the one-step-ahead residuals being larger than that of the conventional residuals. This difference makes sense since, unlike for the conventional residuals, the predicted value used in the one-step-ahead residuals only uses the information from the observation up to time  $t - 1$  to predict the value at time  $t$ .

The one-step-ahead residuals can be standardized by dividing by their standard deviations or by using the function `residuals` but setting the argument `type="standardized"`.

```
resS2pDlm <- residuals(filter2pDlm, type= "standardized")
```

We then plot these standardized prediction residuals.

```
hist(resS2pDlm$res, breaks=50, freq=FALSE,
     main="", ylab="Prob.", xlab=expression(e[t]),
     las=1, col="darkgrey")
box()
curve(dnorm, -3, 3, add=TRUE, col="hotpink", lwd=3)
qqnorm(y=resS2pDlm$res,
      main="", pch=16, cex=0.8)
qqline(y=resS2pDlm$res, col="hotpink", lwd=2)
```

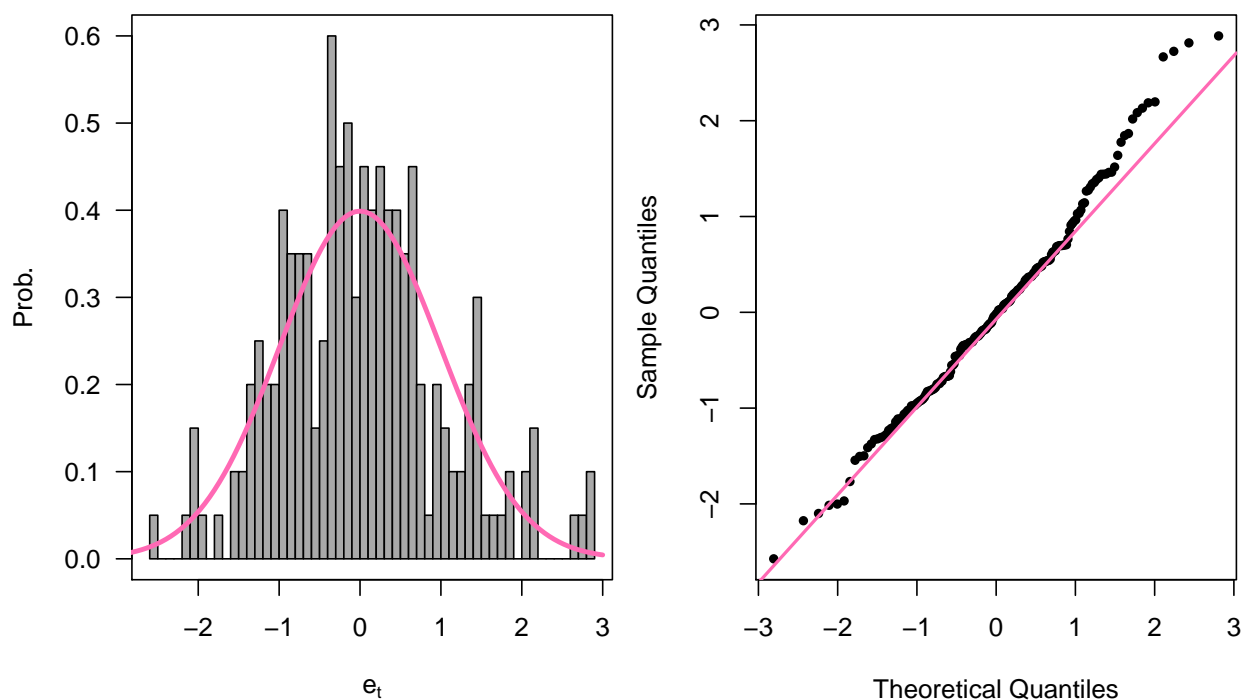

Figure S1.12: Comparison of the standardized one-step-ahead residuals and standard normal distribution.

Now, did using the one-step-ahead prediction reduce the autocorrelation?

```
acf(resS2pDlm$res, las=1, main="")
```



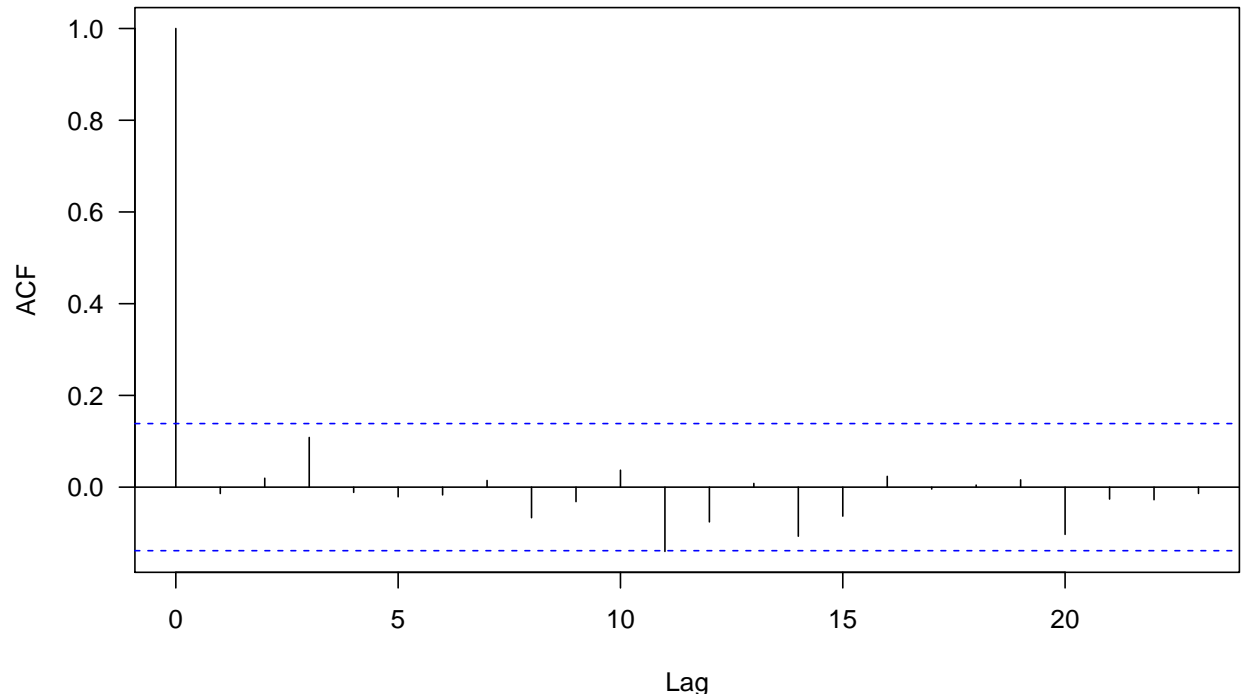

Yes, it did.

In addition to the qqplots and autocorrelation function shown above, we can look at various other features of the standardized one-step-ahead residuals. For example, as discussed in Newman et al. (2014), indices, such as bias index and dispersion index, can be used to assess various aspects of the residuals.

```
# These indices rely on moments of residuals
m1 <- sum(resS2pDlm$res)/TT
m2 <- sum((resS2pDlm$res - m1)^2)/TT
# Bias index
sqrt(TT)*m1

## [1] 0.2871715

# Dispersion index
(TT*m2-TT+1)/sqrt(2*(TT-1))

## [1] 0.04598917
```

Values outside  $[-2, 2]$  can be considered model misfit. Here, the values do not point to obvious problems.

As a note, when we calculate the one-step-ahead observation predictions,  $\hat{y}_{t|1:t-1}$ , even if we use only the observations up to time  $t - 1$  to predict the state and observation at time  $t$ , we use the whole time series

to estimate the parameter values, here the process variation standard deviation and the measurement error standard deviation. Thus, despite using varying time series length, these residuals are residuals for the final model with the MLE parameter values.

### S1 1.3.1.6 Model fit of a misspecified model

It is useful to look at a misspecified model, to further explore the diagnostics we just presented. Here, we will simply create a model were we wrongly assumed that the observations are just a small fraction of the states. Specifically, we will wrongly assume that  $\alpha = 0.2$ , despite the fact that our simulations set  $\alpha = 1$ . So we will use almost the same `d1m` model as above, but will set `FF=0.2`.

```
# Create the d1m object for mispecified model
# Remember
# m0 = initial value of the state, z[0]
# C0 = variance of the initial value
# GG = matrix multiplier in the State Eq: z[t] = GG*z[t-1] + epsilon[t]
# W = state process variance
# FF = matrix multiplier in the Obs. Eq: y[t] = FF*z[t] + eta[t]
# V = observation error variance
mMisD1m <- d1m(m0=0, C0=0, GG=1, W=sdp^2, FF=0.2, V=sdo^2)
```

As before, let us use the Kalman filter to get the one-step-ahead predictions.

```
filterMisD1m <- d1mFilter(y=y, mod=mMisD1m)
```

Now let us calculate the one-step-ahead residuals. Again, the forecast predictions of the observations are kept in the component `f` returned by `d1m` and we can get the variance of the predictions with the function `d1mSvd2var`.

```
resSMisD1m <- residuals(filterMisD1m, type="standardized")$res
```

Let us look at the diagnostic plots again.

```
plot(resSMisD1m, ylab="One-step-ahead residuals", xlab="t",
     pch=19, cex=0.8, las=1)
abline(h=0, col="hotpink")
acf(resSMisD1m, las=1, main="")
hist(resSMisD1m, breaks=50, freq=FALSE,
     main="", ylab="Prob.", xlab=expression(e[t]),
     las=1, col="darkgrey")
box()
```

```

curve(dnorm, -3, 3, add=TRUE, col="hotpink", lwd=3)
qqnorm(y=resSMisDlm,
       main="", pch=16, cex=0.8)
qqline(y=resSMisDlm, col="hotpink", lwd=2)

```

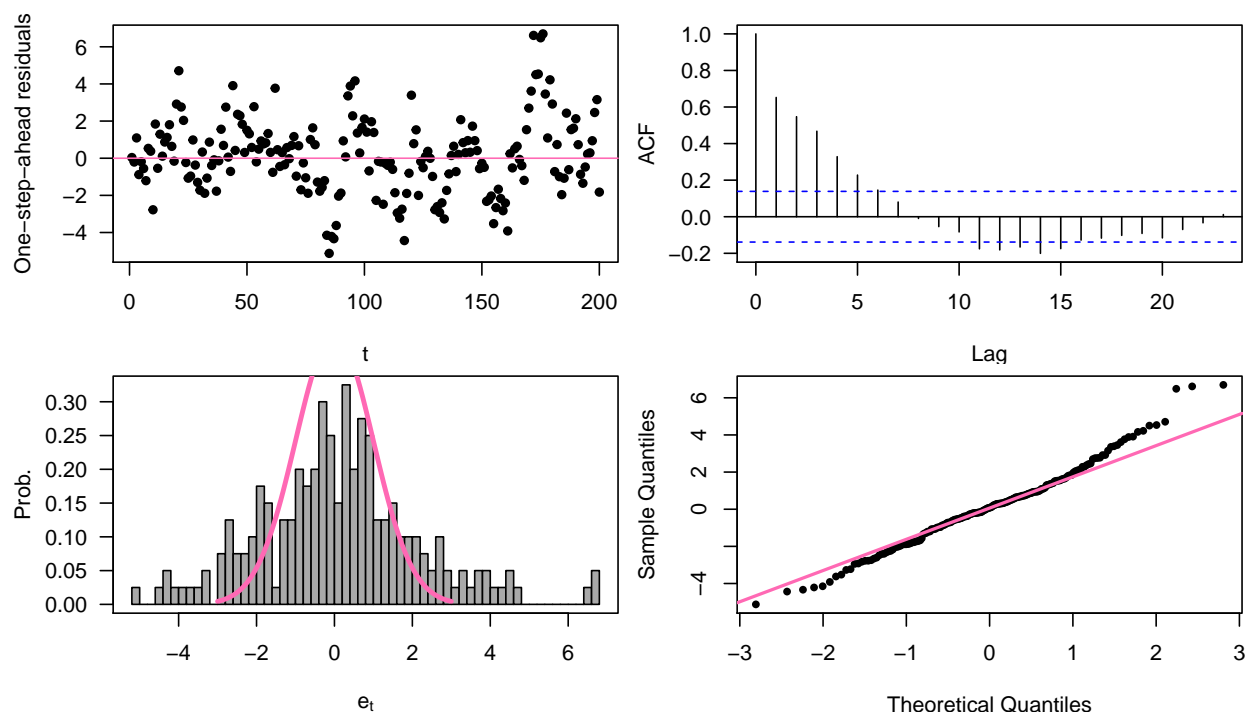

Figure S1.13: Diagnostic plots for a misspecified model.

We can see here the strong cyclical patterns in the residuals and the strong autocorrelation. If we plot it against our known simulated values, we can see that our state predictions would be extremely wrong.

```

plot(1:TT, y,
     pch=3, cex = 0.8, col="blue", ty="o", lty = 3,
     xlab = "t", ylab = expression(z[t]),
     xlim = c(0,TT),
     ylim = c(min(filterMisDlm$m), max(filterMisDlm$m)+max(filterMisDlm$m)/8),
     las = 1)
points(0:TT, z,
      pch = 19, cex = 0.7, col = "red", ty = "o")
lines(0:TT, filterMisDlm$m,
     lwd=2)

```

```

legend("top",
  legend = c("Obs.", "True states", "Filter. states"),
  pch = c(3, 19, NA),
  col = c("blue", "red", "black"),
  lwd = c(1, 1, 2), lty = c(3, 1, 1),
  horiz=TRUE, bty="n", cex=0.9)

```

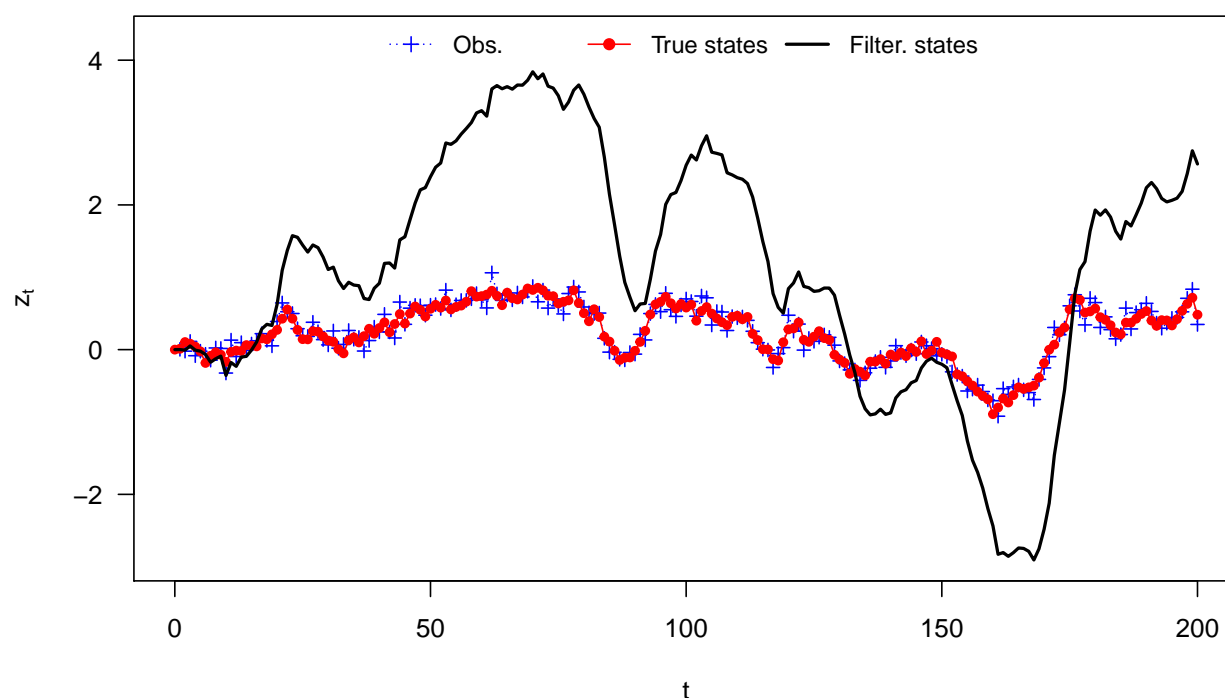

Figure S1.14: Estimates from the Kalman filter for our misspecified model.

This is an artificial example, that may not be realistic in many cases, but it demonstrates how one-step-ahead residuals can help check model fit.

## S1 1.3.2 TMB

### S1 1.3.2.1 Fitting the model

In TMB you need to create a C++ file that computes the value of the negative log likelihood for your data and for a given set of parameter values. Then, you compile the C++ code using TMB and use that function in one of R's optimizers to find the minimum negative log likelihood. The beauty of TMB is that it uses the Laplace approximation to integrate over the states and computes the gradient efficiently, which speeds up the optimizing process.

Because TMB use C++ code, the installation of the package requires additional steps. The package is available on CRAN <https://cran.r-project.org/web/packages/TMB/index.html>, however your computer needs to be set up so you can compile the C++ code. You can find installation information at: <https://github.com/kaskr/adcomp/wiki/Download>. Briefly, if you are Mac user, you will need to install the Xcode developer tools (freely available via the App store). With older versions of Mac OS, you may run into problems with the Fortran compiler. For solutions, see the link above and this link <https://mac.r-project.org/tools/>. If you are a Windows user, you will need to install Rtools and you can find guidelines on how to install properly TMB on a Windows machine here: <https://github.com/kaskr/adcomp/wiki/Windows-installation>. You can find information on the latest version of Rtools here: <https://cran.r-project.org/bin/windows/Rtools/>.

Assuming you have properly installed TMB, let's load it.

```
library(TMB)
```

Now, let us create the negative log-likelihood function that we will minimize (equivalent of maximizing the likelihood). We write this function in a special TMB C++ language. The code for the function needs to be save in a text file. We usually give it the extension .cpp. You can do this directly in R Studio. You write the code just as you would write an R script, but you save it as a .cpp file by giving it the .cpp extension.

We name the file *toy2p.cpp* and it will contain the following code. Note that in C++, comments are preceded by // or contained within /\* \*/. Also, as explained below, here the code is a little bit more complex than strictly necessary. We have included code that allow us to compute the one-step-ahead residuals and simulate from the model. While these features are not always necessary, they are key to model checking and thus we believe they should be part of all model fitting workflow.

```
/*----- SECTION A -----*/
// Link to the TMB package
#include <TMB.hpp>

/*----- SECTION B -----*/
// Define main function
template<class Type>
Type objective_function<Type>::operator() ()
{

    /*----- SECTION C -----*/
    // Specify the input data
    DATA_VECTOR(y);

    // For one-step-ahead residuals
    DATA_VECTOR_INDICATOR(keep, y);

    // Specify the parameters
```

```

PARAMETER(logSdP); // Log of st. dev. for the process variation
PARAMETER(logSd0); // Log of st. dev. for the observation error

// Specify the random effect/states
PARAMETER_VECTOR(z);

/*----- SECTION D -----*/
// Transform standard deviations
// exp(par) is a trick to make sure that the estimated sd > 0
Type sdp = exp(logSdP);
Type sdo = exp(logSd0);

/*----- SECTION E -----*/
// Define the variable that will keep track of
// the negative log-likelihood (nll)
Type nll = 0.0;

/*----- SECTION F -----*/
// Calculate the contribution to the negative log-likelihood
// of the process equation for t=1,...,T
// Remember that we fixed z_0 = 0
for(int i = 1; i < z.size(); ++i){
    nll -= dnorm(z(i), z(i-1), sdp, true);

    /*----- SECTION G -----*/
    // Simulation block for process equation
    SIMULATE {
        z(i) = rnorm(z(i-1), sdp);
    }
}

/*----- SECTION H -----*/
// Calculate the contribution to the negative log-likelihood
// of the observation equation for t=1,...,T
// Remember, the first element of z is at t=0,
// while the first element of y is at t=1
for(int i = 0; i < y.size(); ++i){
    nll -= keep(i)*dnorm(y(i), z(i+1), sdo, true);

    /*----- SECTION I -----*/

```

```

// Simulation block for observation equation
SIMULATE {
  y(i) = rnorm(z(i+1), sdo);
}
}

/*----- SECTION J -----*/
// State the transformed parameters to report
// Using ADREPORT will return the point values and the standard errors
// Note that we only need to specify this for parameters
// we transformed, see section D above
// The other parameters, including the random effects (states),
// will be returned automatically
ADREPORT(sdp);
ADREPORT(sdo);

/*----- SECTION K -----*/
// Report simulated values
SIMULATE{
  REPORT(z);
  REPORT(y);
}

/*----- SECTION L -----*/
// State that we want the negative log-likelihood to be returned
// This is what the optimizer in R will minimize
return nll;
}

```

A course on how to code in C++ is beyond the scope of this tutorial, but here are a few things to note.

- C++ uses round brackets for both objects and functions, unlike R that uses square brackets for the former.
- An important difference between R and C++ is that the index of an object in C++ starts at 0, not 1. For example, to get the first element of a vector called `x`, you write `x(0)`. This is why the for-loops in sections F and H end before the length of the index, which is specified by `.size()`. If R crashes when you compile the code (see below for compiling instruction), the most likely culprit is an index problem, so check your for-loops.

- In C++, lines end with ;
- Like R, C++ is a case sensitive language, e.g., `var1` and `VAR1` are not synonymous.
- In R, we often want to use functions that can be applied to vectors or matrices and avoid for-loops when possible. However, C++ is much more efficient and there is no concern with using for-loops.
- If we want to use an unconstrained optimizer in R, we have to specify in the negative log-likelihood function that we transform the values provided by the optimizer into values that are in the appropriate domain. For example, here in section D, we exponentiate the input log-transformed standard deviations (`logSdP` and `logSdO`) to ensure that the standard deviations have positive values. We do this so that we can use an unconstrained optimizer, yet only have positive estimated values for the standard deviations. By default, TMB will only return the estimated values in the same form as given in the function (e.g., `logSdP` rather than `sdp`). To be able to retrieve the estimate values of interest, we need to specify that we want them returned. This is done in section J.
- Many of the density functions available in R are available in C++, at least when using the TMB package. These usually have the same names and arguments as those in R. For example, in sections F and H we use `dnorm` just like we would in R.
- Note that we have included simulation blocks (sections G, I, and K), even though these blocks are not necessary to fit the model to data. These blocks are extremely useful for model validation, see the model validation section below for details.
- Similarly, while it is not necessary to fit the model, we have added an indicator variable (`keep`) in both sections C and H. This indicator variable is necessary to calculate the one-step-ahead residuals that we will discuss in the model validation section.

Now that a few things are defined, it may be easier to go back to the function and see what it means. Section A loads the packages needed. Section B indicates that we are defining the main function that will calculate the negative log likelihood. Section C defines the data and parameters. The values of both data and parameters will be put in through R. Section D transforms the parameters so that they are constrained appropriately (here, that the standard deviation are  $> 0$ ). Section E creates the object that will keep track of the negative log likelihood. Section F has a for-loop that calculates the contribution to the negative log likelihood of the process equation. Section G allows to simulate the process equation. Section H calculates the contribution to the negative log likelihood of the observation equation. Note that using `keep` tells TMB that this is where we would remove the data for the one-step ahead residuals. Section I allows to simulate the observation equation. Section J indicates that we want the parameters in their untransformed form to be returned with their standard errors. Section K indicates what to report when we simulate the model. Section L indicates that the main item the function returns is the negative log likelihood.

Now that we have the negative log likelihood C++ file saved, we go back to R.

The first thing we want to do is compile the C++ code and load it so we can use it to calculate the negative log likelihood of our model. Here, our `toy2p.cpp` file is found in the working directory.

```
compile("toy2p.cpp")
dyn.load(dynlib("toy2p"))
```



Some users get a warning stating that `warning: pragma diagnostic pop could not pop, no matching push`. In most cases, this warning can be ignored.

Now let us prepare the model for fitting. First, we need to prepare the data. This is going to be a list with all the items found in the .cpp files that are of the type `DATA`, e.g., `DATA_VECTOR`. Here, we only have `y` which is the time series of observed values.

```
dataTmb <- list(y = y)
```

Second, we need a list with the parameters. Again the names need to match those in the .cpp file. These are the starting values for the parameters. Note that this includes both the parameters and the states.

```
par2pTmb <- list(logSdP = 0, logSd0 = 0,  
                 z=rep(0,length(dataTmb$y)+1))
```

Here, we assume that we know the value of the state at time 0,  $z_0 = 0$ . This does not need to be the case, but it reflects how we created the model in the previous section. To provide this information to `TMB`, we can create a named list that we will input for the argument `map` of the function `MakeADFun`. For `TMB` to be able to connect `map` to the `par2pTmb`, the elements of `map` should have the same name and size as those in `par2pTmb`. Here, we only need to specify the elements that we want to manipulate. By default all values of `par2pTmb` will be estimated, but we want to fix the first value of the state vector `par2pTmb$z`. To fix a value, we set that value to `NA`. The values that are estimated should have a different entry and all values should be factors. See help file of `MakeADFun` for more details and options.

```
mapTmb <- list(z=as.factor(c(NA,1:length(dataTmb$y))))
```

Before we can fit the model, we need to create the `TMB` object with the function `MakeADFun`. This object will combine the data, the parameters, and the model and will create a function that calculates the negative log likelihood and the gradients. Here, because we fix the first state value, we also use the `map` argument. To identify our random effects, namely the states,  $z_t$ , we set the argument `random` to equal the name of the parameters that are random effects. The argument `DLL` identify the compile C++ function to be linked.

```
m2pTmb <- MakeADFun(data=dataTmb, parameters=par2pTmb, map=mapTmb, random= "z",  
                   DLL= "toy2p")
```

`TMB` is an unusual package in that as we will see below, the object `m2pTmb` gets changed by functions. This object is the most important object of `TMB` and it is useful to see the output from the `MakeADFun` call.

```
names(m2pTmb)  
  
## [1] "par"      "fn"      "gr"      "he"      "hessian" "method"  
## [7] "retape"   "env"     "report"  "simulate"
```

For example, we can see that we can access things like the function that calculates the negative log likelihood with the element `fn` or the function that simulate the data with the element `simulate`.

Now, we can fit the model. We do this using `nlminb`, which is a basic optimizer from R, but we input the object returned by TMB.

```
f2pTmb <- nlminb(m2pTmb$par, m2pTmb$fn, m2pTmb$gr)

## iter: 1  value: 368.6555 mgc: 1.061776 ustep: 1
## iter: 2  mgc: 4.440892e-16
## iter: 1  mgc: 4.440892e-16
## Matching hessian patterns... Done
## outer mgc: 109.3254
## iter: 1  value: 90.69158 mgc: 0.2514893 ustep: 1
## iter: 2  mgc: 8.881784e-16
## iter: 1  value: -477.3156 mgc: 55.54479 ustep: 1
## iter: 2  mgc: 6.039613e-14
## iter: 1  mgc: 6.039613e-14
## outer mgc: 225.3194
## iter: 1  value: -205.0396 mgc: 557.3927 ustep: 1
## iter: 2  mgc: 5.451958e-13
## iter: 1  value: -375.5514 mgc: 10.14496 ustep: 1
## iter: 2  mgc: 1.154632e-14
## iter: 1  mgc: 1.154632e-14
## outer mgc: 95.11226
## iter: 1  value: -342.4495 mgc: 48.33261 ustep: 1
## iter: 2  mgc: 1.561945e-14
## iter: 1  value: -401.7492 mgc: 19.08992 ustep: 1
## iter: 2  mgc: 1.332268e-14
## iter: 1  mgc: 1.332268e-14
## outer mgc: 35.79675
## iter: 1  value: -467.4255 mgc: 9.503653 ustep: 1
## iter: 2  mgc: 2.4869e-14
## iter: 1  value: -437.8951 mgc: 2.972293 ustep: 1
## iter: 2  mgc: 1.953993e-14
## iter: 1  mgc: 1.953993e-14
## outer mgc: 3.120246
## iter: 1  value: -432.2481 mgc: 12.88012 ustep: 1
## iter: 2  mgc: 1.998401e-14
## iter: 1  value: -439.9835 mgc: 0.9733806 ustep: 1
## iter: 2  mgc: 1.598721e-14
## iter: 1  mgc: 1.598721e-14
```

```

## outer mgc: 0.7726568
## iter: 1 value: -438.2002 mgc: 1.182135 ustep: 1
## iter: 2 mgc: 1.665335e-14
## iter: 1 value: -438.7687 mgc: 0.3016119 ustep: 1
## iter: 2 mgc: 1.865175e-14
## iter: 1 mgc: 1.865175e-14
## outer mgc: 0.8233773
## iter: 1 value: -439.3465 mgc: 0.4941537 ustep: 1
## iter: 2 mgc: 1.865175e-14
## iter: 1 mgc: 1.865175e-14
## outer mgc: 0.3128115
## iter: 1 value: -439.5828 mgc: 0.4580236 ustep: 1
## iter: 2 mgc: 1.776357e-14
## iter: 1 value: -439.3929 mgc: 0.2216172 ustep: 1
## iter: 2 mgc: 1.953993e-14
## iter: 1 mgc: 1.953993e-14
## outer mgc: 0.133623
## iter: 1 value: -439.1178 mgc: 0.005532313 ustep: 1
## iter: 2 mgc: 1.709743e-14
## iter: 1 value: -439.2795 mgc: 0.007224241 ustep: 1
## iter: 2 mgc: 1.687539e-14
## iter: 1 mgc: 1.687539e-14
## outer mgc: 0.003828423
## iter: 1 value: -439.2822 mgc: 0.006147352 ustep: 1
## iter: 2 mgc: 1.598721e-14
## iter: 1 mgc: 1.598721e-14
## outer mgc: 0.0002551507
## iter: 1 value: -439.2821 mgc: 0.0003670934 ustep: 1
## iter: 2 mgc: 1.865175e-14
## iter: 1 mgc: 1.865175e-14
## outer mgc: 6.507887e-08
## iter: 1 mgc: 1.865175e-14

```

This function will print some of the inner and outer optimization results. These values can be useful in understanding optimization issues, but can also be silenced using the argument `silent = TRUE` in the function `MakeADFun`.

It is good to check convergence.

```
f2pTmb$message
```

```
## [1] "relative convergence (4)"
```

Looks like it converged. A message stating "both X-convergence and relative convergence (5)" would also indicate convergence.

To look at the parameter estimates, you can use the function `sdreport`. Note that as mentioned above, TMB is unusual in that when we use `nlminb` with a TMB model object (here, `m2pTmb`), the TMB object itself is modified. While `nlminb` returns an object (here, `f2pTmb`), we still heavily rely on the altered TMB object `m2pTmb` to access many of the interesting results. Here, for example, to get the estimates of the untransformed process variation and observation error and their standard errors, we use the function `sdreport` on `m2pTmb`.

```
sdr2pTmb <- summary(sdreport(m2pTmb))

## iter: 1  mgc: 1.865175e-14
## outer mgc: 6.507887e-08
## iter: 1  value: -439.1902 mgc: 0.04165698 ustep: 1
## iter: 2  mgc: 1.831868e-14
## outer mgc: 0.1427246
## iter: 1  value: -439.3738 mgc: 0.04174038 ustep: 1
## iter: 2  mgc: 2.04281e-14
## outer mgc: 0.1427344
## iter: 1  value: -439.1738 mgc: 0.04165698 ustep: 1
## iter: 2  mgc: 1.798561e-14
## outer mgc: 0.1099994
## iter: 1  value: -439.3902 mgc: 0.04174038 ustep: 1
## iter: 2  mgc: 1.865175e-14
## outer mgc: 0.1098888
## outer mgc: 0.1174192

# This will have the parameters and states
# So we can just print the parameters
sdr2pTmb[c("sdp", "sdo"),]

##      Estimate Std. Error
## sdp 0.1174192 0.01215134
## sdo 0.0914208 0.01077956
```

We can see that the estimates for both the process variation and the observation error are close to their true value of 0.1, with relatively small standard errors (SEs).

We can get the smoothed state values with the `sdreport` function as above and this will give you the SEs for these states. If you are only interested in the state values, you can also extract them directly from the model object. When you have a more complex model fitted to a larger data set, the later option can come in handy as it does not require further optimization.

```

# To get the point estimate and the SE of the states
zsSe2pTmb <- sdr2pTmb[row.names(sdr2pTmb)=="z",]
head(zsSe2pTmb)

##           Estimate Std. Error
## z  0.002425299 0.06414118
## z  0.002627362 0.06694764
## z  0.042147684 0.06807862
## z -0.036653040 0.06740099
## z -0.037413169 0.06720760
## z -0.064181179 0.06723443

# To get only the point estimates of the states
zs2pTmb <- m2pTmb$env$parList()$z
head(zs2pTmb)

## [1] 0.000000000 0.002424767 0.002620967 0.042203573 -0.036679365
## [6] -0.037408983

```

Note that in this case, because we fixed the value of the state at time  $t = 0$ , the first method, which looks at the predicted values, only returns state values for  $t > 0$ .

As with `dlm`, we can use the SEs to calculate the 95% confidence intervals.

```

zsCI12pTmb <- zsSe2pTmb[,1] +
  qnorm(0.025, sd = zsSe2pTmb[,2])
zsCIu2pTmb <- zsSe2pTmb[,1] +
  qnorm(0.975, sd = zsSe2pTmb[,2])

```

We can now overlay the state estimates along with their confidence intervals on the plot of the simulated data.

```

plot(1:TT, y,
     pch=3, cex=0.8, col="blue", ty="o", lty = 3,
     xlab = "t", ylab = expression(z[t]),
     xlim = c(0,TT), ylim = c(min(y), max(y)+max(y)/5),
     las = 1)
points(0:TT, z,
      pch=19, cex=0.7, col = "red", ty="o")
polygon(c(1:TT, TT:1), c(zsCI12pTmb, rev(zsCIu2pTmb)),

```

```

col=rgb(1,0.7,0.4,0.3), border=FALSE)
lines(0:TT, zs2pTmb,
      col= "darkgoldenrod1", lwd = 2)
legend("top",
      legend = c("Obs.", "True states", "Smooth. states"),
      pch = c(3, 19, NA),
      col = c("blue", "red", "darkgoldenrod1"),
      lwd = c(1, 1, 2), lty = c(3, 1, 1),
      horiz=TRUE, bty="n", cex=0.9)

```

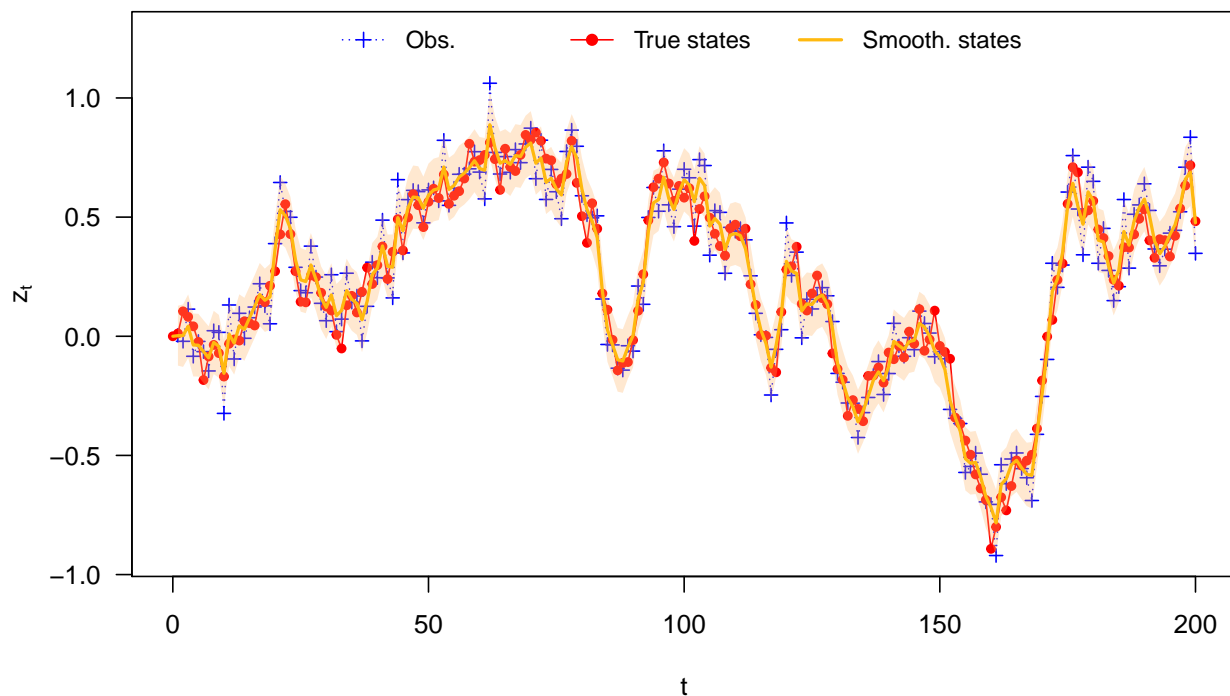

Figure S1.15: Comparing the state estimates from TMB with the true simulated values.

### S1 1.3.2.2 Model comparison

As we explore in the section S1 1.3.1.3, we could fit the more general and slightly more complex version of the model (Eqs. 1.1-1.2), where we are estimating in addition to the standard deviations,  $\alpha$  and  $\beta$ . In our simulation, both  $\alpha$  and  $\beta$  are implicitly set to 1. Here we estimate these values.

To fit this model in TMB, we will create a new file called *toy4p.cpp*. Note that this is exactly the same as *toy2p.cpp* except that we added the two new parameters in sections C, and F to I.

```

/*----- SECTION A -----*/
// State that we need the TMB package
#include <TMB.hpp>

/*----- SECTION B -----*/
// Define main function
template<class Type>
Type objective_function<Type>::operator() ()
{

    /*----- SECTION C -----*/
    // Specify the input data
    DATA_VECTOR(y);

    // For one-step-ahead residuals
    DATA_VECTOR_INDICATOR(keep, y);

    // Specify the parameters
    PARAMETER(logSdP); // Log of st. dev. for the process variation
    PARAMETER(logSd0); // Log of st. dev. for the observation error
    PARAMETER(alpha);
    PARAMETER(beta);

    // Specify the random effect/states
    PARAMETER_VECTOR(z);

    /*----- SECTION D -----*/
    // Transform standard deviations
    // exp(par) is a trick to make sure that the estimated sd > 0
    Type sdP = exp(logSdP);
    Type sdo = exp(logSd0);

    /*----- SECTION E -----*/
    // Define the variable that will keep track of
    // the negative log-likelihood (nll)
    Type nll = 0.0;

    /*----- SECTION F -----*/
    // Calculate the contribution to the negative log-likelihood
    // of the process equation for t=1,...,T

```

```

// Remember that we fixed z_0 = 0
for(int i = 1; i < z.size(); ++i){
    nll -= dnorm(z(i), beta*z(i-1), sdp, true);

    /*----- SECTION G -----*/
    // Simulation block for process equation
    SIMULATE {
        z(i) = rnorm(beta*z(i-1), sdp);
    }
}

/*----- SECTION H -----*/
// Calculate the contribution to the negative log-likelihood
// of the observation equation for t=1,...,T
// Remember, the first element of z is at t=0,
// while the first element of y is at t=1
for(int i = 0; i < y.size(); ++i){
    nll -= keep(i)*dnorm(y(i), alpha*z(i+1), sdo, true);

    /*----- SECTION I -----*/
    // Simulation block for observation equation
    SIMULATE {
        y(i) = rnorm(alpha*z(i+1), sdo);
    }
}

/*----- SECTION J -----*/
// State the transformed parameters to report
// Using ADREPORT will return the point values and the standard errors
// Note that we only need to specify this for parameters
// we transformed, see section D above
// The other parameters, including the random effects (states),
// will be returned automatically
ADREPORT(sdp);
ADREPORT(sdo);

/*----- SECTION K -----*/
// Report simulated values
SIMULATE{
    REPORT(z);
}

```



```

    REPORT(y);
  }

  /*----- SECTION L -----*/
  // State that we want the negative log-likelihood to be returned
  // This is what the optimizer in R will minimize
  return nll;
}

```

As before, we compile and load the function.

```

compile("toy4p.cpp")
dyn.load(dynlib("toy4p"))

```

We create the TMB object. We can use the same data and map objects as above, but we need to change the object containing the initial parameter values, because we have two new parameters to estimate. We then get the MLE. Note that while TMB can often use uninformative starting values (e.g., 0), we can run into estimation problems if we set all the starting values as 0s (see section S1 1.3.2.5 below for example of the results when we use all 0s as starting values). To avoid these problems, we use the true simulated values for the starting values. With real data, we could have started with sensible values rather than 0.

```

par4pTmb <- list(logSdP = log(0.1), logSd0 = log(0.1), alpha = 1, beta = 1,
                z=rep(0,length(dataTmb$y)+1))
m4pTmb <- MakeADFun(dataTmb, par4pTmb, map=mapTmb, random= "z",
                  DLL= "toy4p", silent=TRUE)
f4pTmb <- nlminb(m4pTmb$par, m4pTmb$fn, m4pTmb$gr)
f4pTmb$message

## [1] "relative convergence (4)"

```

We can see here that the optimizer has converged.

We can use again `sdreport` to get the parameter estimates and their SEs.

```

sdr4pTmb <- summary(sdreport(m4pTmb))
cbind(Simulated = c(sdp, sdo, 1, 1),
      sdr4pTmb[c("sdp", "sdo", "beta", "alpha"),])

```

```
##           Simulated   Estimate   Std. Error
## sdp           0.1 0.11071196   7.68255211
## sdo           0.1 0.08875577   0.01140797
## beta          1.0 0.96582525   0.02029411
## alpha          1.0 1.08587219  75.35103488
```

We can see here that compared to the estimates from the original model, the more complex and flexible model has much higher standard errors. As mentioned above, the optimization process is also quite sensitive to the starting values. Thus in a real analysis, where we would not know in advance the true values of the parameters, we may have found parameter estimates that are not the true MLE, but only local maximum values, see below.

In any case, just like in section on `d1m`, we can use AIC to compare these two models (see section S1 1.3.1.3 for more details). Since the C++ function calculates the negative log likelihood and is the objective of the optimization procedures, we can just use the returned value by `nlminb`.

```
aic2pTmb <- 2 * 2 + 2 * f2pTmb$objective
aic4pTmb <- 2 * 4 + 2 * f4pTmb$objective
c(Original = aic2pTmb, Flexible = aic4pTmb,
  Difference = aic4pTmb - aic2pTmb)

##           Original      Flexible   Difference
## -143.7326417 -142.7907205      0.9419212
```

We can see that just like when we used `d1m`, the original model has a lower AIC than the more flexible model. Thus the original model is considered better. If the two models were equivalent, we would expect a AIC difference of 4 ( $2k$ ), but here the difference is much smaller: 0.94. As we will see below, this may be because the more flexible model is overfitting the data.

### S1 1.3.2.3 Checking estimability and model fit with simulations

As mentioned above, while not necessary to fit the model to data, it is good practice to include simulation blocks within the C++ code because while it is often easy to simulate your model in R, it can be advantageous to use TMB simulation functions to simulate directly from TMB. This can speed up the process and, as we will see below, can help assess the model fit. TMB has various simulators that have the same naming convention as those in R, e.g.: `rnorm()`, `rpois()`, `rbinom()`, `rgamma()`. A few things to note. If you use, for example, `rnorm(n, mu, sd)`, `mu` and `sd` can only contain a single value each. However, if you use `rnorm(mu, sd)`, you can use vectors for `mu` or `sd`. Check however, that the length of these objects make sense because there is no re-cycling<sup>1</sup>.

The `SIMULATE` blocks identifies the simulation and is not executed by default (but we show how to execute this below). In the `toy2p.cpp` file we created above, we have three simulation blocks (sections G, I, and

<sup>1</sup>We have not presented the density objects yet, but note that they have their own `simulate()` method.

K). Sections G and I simulate respectively the process and observation equations. Section K identify the simulated values to return.

If we want to recreate the exact same simulation as we did in R in section S1 1.2, our first step is to create a TMB model object with `MakeADFun`. Just as before, we need to set up the parameter and data object. We could use the same data object as above or we can create a data object with 0s, which has the length of the time series we want to create. Let us use 0s. Instead of using 0 as parameter values for the two standard deviations, we will set these values to 0.1, the values used in the original simulations above. Remember that the parameters values are transformed within the C++ function, so here we have to reverse transform them. For the states, we will create a vector of 0 of the length of our state vector. We will use the same `map` object as above to tell TMB that the initial state value is  $z_0 = 0$ .

```
dataSimTmb <- list(y = numeric(TT))
parSimTmb <- list(logSdP = log(0.1), logSd0 = log(0.1),
                  z=rep(0,length(dataSimTmb$y)+1))
```

We will then create the TMB object using `MakeADFun` function, just as above.

```
mSimTmb <- MakeADFun(dataSimTmb, parSimTmb, map=mapTmb, random= "z",
                     DLL= "toy2p", silent=TRUE)
```

Finally, we will simulate the data using the created TMB object. To do so, we use the method `$simulate()`.

```
set.seed(553)
simTmb <- mSimTmb$simulate()
```

Note that we do not give parameter values. By default TMB use the last parameter values used, which can be identified with `obj$env$last.par` (here `mSimTmb$env$last.par`). In this case, it used the starting values. You can, however, use the argument `par` to specify parameter values <sup>2</sup>.

```
names(simTmb)

## [1] "y" "z"
```

Here, we can see that both the observations `y` and the states `z` are returned. This is because section K of the C++ code specifically states to return both.

Note that because we used the same random seed as for the original simulation, you will get the same results, despite inputting 0s as data to TMB.

---

<sup>2</sup>Note, however, that when you use `mSimTmb$simulate(par=yourPar)` you need to take into account the parameters that are fixed with the `map` argument and you need to input a numeric vector instead of a list. It is useful to use `mSimTmb$env$par` as basis for modification, as it will already have the good number of parameters and will be in the correct format.

```
tail(cbind("Orig. y" =y, "TMB y"=simTmb$y,
          "Orig. z"=z[-1], "TMB z"=simTmb$z[-1]))

##           Orig. y      TMB y   Orig. z      TMB z
## [195,] 0.4327629 0.4327629 0.3346828 0.3346828
## [196,] 0.4446149 0.4446149 0.4216397 0.4216397
## [197,] 0.5224154 0.5224154 0.5364825 0.5364825
## [198,] 0.7093278 0.7093278 0.6324794 0.6324794
## [199,] 0.8351053 0.8351053 0.7175746 0.7175746
## [200,] 0.3479429 0.3479429 0.4828078 0.4828078
```

How can these simulation blocks be useful for model verification?

As mentioned in the `d1m`, the first is to use the simulations to assess whether we can estimate the parameter and states. Here, once you have define you C++ code appropriately, you can simulate and check that your model can estimate the parameter and states in only a few lines of code (note some code is repeated from above).

```
# Simulate the data (same code as above)
set.seed(553)
dataSimTmb <- list(y = numeric(TT))
parSimTmb <- list(logSdP = log(0.1), logSd0 = log(0.1),
                 z=rep(0,length(dataSimTmb$y)+1))
mSimTmb <- MakeADFun(dataSimTmb,
                    parSimTmb, map=mapTmb, random= "z",
                    DLL= "toy2p", silent=TRUE)
simTmb <- mSimTmb$simulate()
# Fit the model to check estimation
mCheckTmb <- MakeADFun(list(y = simTmb$y), # Note difference in this argument
                      parSimTmb, map=mapTmb, random= "z",
                      DLL= "toy2p", silent=TRUE)
fCheckTmb <- nlminb(mCheckTmb$par, mCheckTmb$fn, mCheckTmb$gr)
fCheckTmb$message

## [1] "relative convergence (4)"

# Compare simulated and estimated parameters
cbind("True" = parSimTmb[1:2], "Est" = fCheckTmb$par)

##           True      Est
## logSdP -2.302585 -2.142005
## logSd0 -2.302585 -2.392283
```

```
# Compare simulated and estimated states - difference
summary(abs(simTmb$z - mCheckTmb$env$parList()$z))

##      Min. 1st Qu.  Median    Mean 3rd Qu.    Max.
## 0.00000 0.01925 0.04398 0.05080 0.07435 0.17557
```

As we can see, the parameter (here untransformed) and the state estimates are close to the simulated value. This is a quick check here, but one could look at the RMSPE and plot the results as in section S1 1.3.1.4.

#### S1 1.3.2.4 Assessing model fit with simulation-based methods similar to posterior predictive measures

As discussed in the main text, one simple, albeit often conservative, way to look at the model fit is to use the frequentist equivalent of posterior predictive measures. This is another way in which TMB's simulation features will come handy. The idea is to define a test statistic (e.g., the mean of  $\mathbf{y}$ ) and calculate how probable more extreme values of this test statistic would be if we were to sample from our model compared to the observed test statistic value. Here, we will look at two test statistics: the mean  $y_t$  and the standard deviation of  $y_t$ . We will simply simulate a time series of observations 200 times and, for each replicate, calculate the mean and standard deviation of that replicate. We will then be able to compare the simulated test statistics to the observed test statistics.

Note here we will use the parameter values we estimated for this simple model above.

```
nrep <- 200 # Number of replicates
set.seed(999) # Set the random seed to be able to reproduce the simulation
# Create matrix to keep track of replicate test statistic values
repsT <- matrix(NA, nrow=nrep, ncol=2)
colnames(repsT) <- c("Mean", "SD")
# Parameter to use to simulate
parSp <- m2pTmb$env$par
# Set to estimated values
parSp[1:2] <- f2pTmb$par
for(i in 1:nrep){ # For each replicate
  yrep <- mSimTmb$simulate(par=parSp)$y # simulate observations
  repsT[i, "Mean"] <- mean(yrep)
  repsT[i, "SD"] <- sd(yrep)
}
```

To estimate the what is akin to a p-value, we calculate the fraction of test statistic values calculated from the simulated data sets that are greater or equal to the test statistic value calculated from the observed data:

$$p_C = Pr(T(\mathbf{y}^i) \geq T(\mathbf{y}) | \hat{\boldsymbol{\theta}}_{\text{MLE}}), \quad (1.10)$$

where  $\hat{\theta}_{\text{MLE}}$  is the MLE value of  $\theta$ ,  $T(\mathbf{y}^i)$  is the test statistic value of a replicate and  $T(\mathbf{y})$  is the test statistic value for the observed data. Extreme values close to 0 or 1 could be indicative of discrepancies between the model and the data. As here we are looking at the true model with the parameters estimated values that were very close to the true values used to simulate the data, we would expect that the observed test statistics values are similar to that from the replicates.

```
# Calculate estimated pc
sum(repsT[, "Mean"] >= mean(y))/nrep

## [1] 0.385

sum(repsT[, "SD"] >= sd(y))/nrep

## [1] 0.83
```

Here, the values are by no means extreme and are quite central. As such, there is no evidence to suggest that the model is inadequate for the data. It is important to note that we are not accounting here for the fact that we are using the data twice: once to estimate the parameter values and once to assess the fit. Thus, as discussed in the main text, such tests tend to be conservative and often fail to detect lack of fit. Thus, one may not want to rely too heavily on values such as these. But in some cases, they are useful to find large discrepancies between the model and the data. In general, it may be better to stay away from the p-value itself and to look at histograms of the simulated test statistic values, and see where the observed test statistic fall.

```
hist(repsT[, "Mean"], breaks=30,
     main = "", las=1, col="darkgrey",
     xlab = expression(T(y^{i})))
box()
abline(v=mean(y), col="hotpink", lwd=4)
title("Mean Obs.", line=-1.5, adj=0.9)
hist(repsT[, "SD"], breaks=30,
     main="", las=1, col="darkgrey",
     xlab = expression(T(y^{i})))
box()
abline(v=sd(y), col="hotpink", lwd=4)
title("Sd Obs.", line=-1.5, adj=0.9)
```

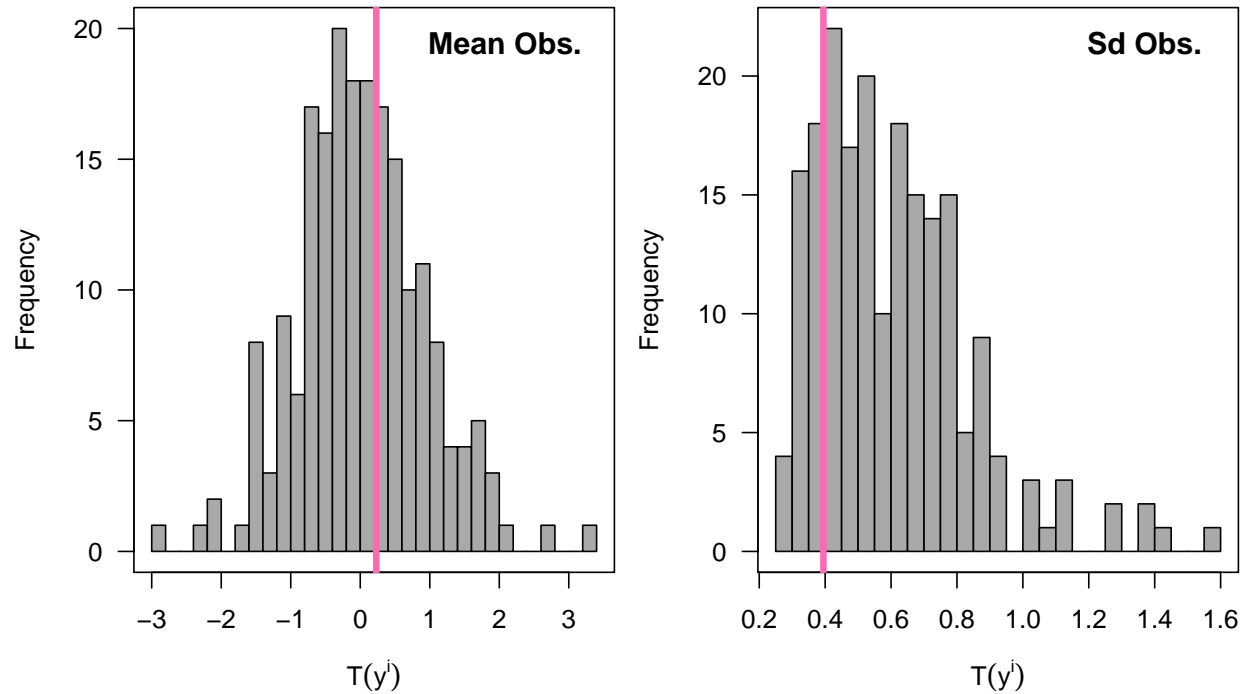

Figure S1.16: Histograms of the two set of simulated test statistics, with observed test statistics shown with the pink line.

We can see here that the observed test statistics are close to the main peaks from the histograms, which suggests that the observations are in line with the prediction of the model. But again, one needs to be careful, as these tests tend to be conservative.

### S1 1.3.2.5 Effects of starting values and diagnostics for a misspecified model

Now let us explore whether the method described above could detect the lack of fit of model with poor parameter estimates. We will use this opportunity to also look at the effect of the starting values on the parameter and state estimates. For this example, we will use again the full more flexible model. However, in this case instead of using the true parameter values as starting values for the optimizer, we will use the default starting values of 0.

```
# Set the starting values
# Here we use 0s everywhere instead of the true values
parMisTmb <- list(logSdP = 0, logSdO = 0, alpha = 0, beta = 0,
                  z=rep(0,length(dataSimTmb$y)+1))
# Make the TMB model function
# We use the original data and map (dataTmb, mapTmb)
mMisTmb <- MakeADFun(dataTmb, parMisTmb, map=mapTmb, random= "z",
```

```

DLL= "toy4p", silent=TRUE)
# Find the MLE - more like a local max
fMisTmb <- nlminb(mMisTmb$par, mMisTmb$fn, mMisTmb$gr)
# Converged
fMisTmb$message

## [1] "relative convergence (4)"

```

It looks like the optimizer converged to a solution, but as we can see below, the parameter estimates based on the previous set of initial values and those used above are quite different. The fact that the parameter values for  $\alpha$  and  $\beta$  are exactly the same as the input starting value should raise warning flags.

```

c(New = fMisTmb$objective, Old = f4pTmb$objective)

##          New          Old
## 126.66737 -75.39536

rbind(New = fMisTmb$par, Old = f4pTmb$par)

##          logSdP      logSd0      alpha      beta
## New   0.000000 -0.7856017 0.000000 0.000000
## Old  -2.200823 -2.4218668 1.085872 0.9658253

```

To see how this estimation problem could affect the model fit, let us use our frequentist version of the posterior predictive measures. We will use the same number of replicates as in section S1 1.3.2.4. Again, we will use the mean and the standard deviation of the observations as test statistics.

```

set.seed(999) # Set the random seed to be able to reproduce the simulation
# Create matrix to keep track of replicate test statistic values
repsB <- matrix(NA, nrow=nrep, ncol=2)
colnames(repsB) <- c("Mean", "SD")
# Parameter to use to simulate
parMisp <- mMisTmb$env$par
# Set to estimated values
parMisp[1:4] <- fMisTmb$par
for(i in 1:nrep){ # For each replicate
  yrep <- mMisTmb$simulate(par=parMisp)$y # simulate observations
  repsB[i, "Mean"] <- mean(yrep)
  repsB[i, "SD"] <- sd(yrep)
}

```



Now let us compare the simulated and observed test statistics visually.

```
# Simulated test statistics vs observed test statistics
hist(repsB[, "Mean"], breaks=30,
     main = "", las=1, col="darkgrey",
     xlab = expression(T(y^{i})),
     xlim = range(c(repsB[, "Mean"], c(0.9, 1.1)*mean(y))))
box()
abline(v=mean(y), col="hotpink", lwd=4)
title("Mean Obs.", line=-1.5, adj=0.9)
hist(repsB[, "SD"], breaks=30,
     main = "", las=1, col="darkgrey",
     xlab = expression(T(y^{i})),
     xlim = range(c(repsB[, "SD"], c(0.9, 1.1)*sd(y))))
box()
abline(v=sd(y), col="hotpink", lwd=4)
title("Sd Obs.", line=-1.5, adj=0.9)
```

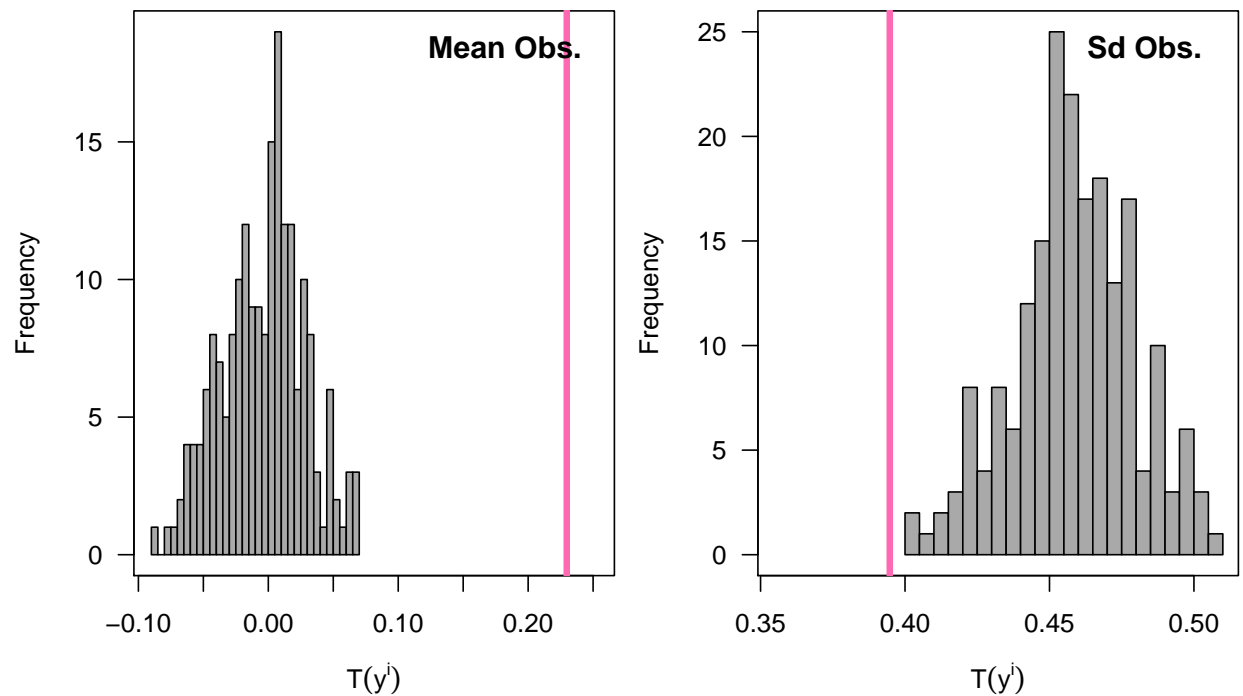

Figure S1.17: Simulated vs observed test statistics for a model with poor parameter estimates.

Clearly, the observations are quite different from those generated from the model with these parameter

estimates. Thus, while we want to be careful when we fail to find a difference between the observed and simulated test statistics, finding such discrepancies is a clear sign of problem.

### S1 1.3.2.6 Looking at model assumptions with residuals

As shown in section S1 1.3.1.5, it is useful to look at residuals to assess model fit. In section S1 1.3.1.5, we showed the problems with the conventional residuals, and the advantage of using the one-step-ahead residuals. The TMB function `oneStepPred` can be used to easily calculate the one-step-ahead residuals. Note that the function is in beta version, so could change. Let us apply it here to our simple toy model. Remember that objects returned by `MakeADFun` get changed by functions, in particular `nlminb` places the estimated parameter and state values in `obj$env$last.par`, which is used by the `oneStepPred` function. To be make sure that we are applying the function on the fitted model, let us rerun the functions `MakeADFun` and `nlminb`.

```
m2pTmb <- MakeADFun(data=dataTmb, parameters=par2pTmb, map=mapTmb, random= "z",
                    DLL= "toy2p", silent=TRUE)
f2pTmb <- nlminb(m2pTmb$par, m2pTmb$fn, m2pTmb$gr)
res2pTmb <- oneStepPredict(m2pTmb, observation.name = "y",
                           data.term.indicator="keep", trace=FALSE)
head(res2pTmb)
```

| ##   | observation  | nll        | grad       | mean          | residual    |
|------|--------------|------------|------------|---------------|-------------|
| ## 1 | 0.003773012  | -0.9858113 | 0.1703774  | 1.639314e-16  | 0.02535421  |
| ## 2 | -0.021207154 | -1.8562750 | -0.8613346 | 2.349038e-03  | -0.14244214 |
| ## 3 | 0.113873261  | -2.4334629 | 4.5755935  | -1.400832e-02 | 0.76494062  |
| ## 4 | -0.083960826 | -2.8474777 | -5.6990189 | 7.563154e-02  | -0.95368752 |
| ## 5 | -0.021647333 | -3.7123166 | 0.5242162  | -3.632978e-02 | 0.08773127  |
| ## 6 | -0.064486165 | -4.5545941 | -1.3730521 | -2.602861e-02 | -0.22979171 |

It returns a matrix with columns that have the predicted observation value (column `mean`) and a column with the residuals (column `residual`). These are one-step-ahead residuals where you use observation up to time  $t - 1$ , as such you cannot get residuals for the first observation. The method TMB uses to calculate the one-step-ahead residuals is general. As discussed in the main text these transformed p-scores can be used on non-normal SSMs as long as the Laplace approximation is adequate for the model. These one-step-ahead residuals should be distributed with a standard normal. Thus we can use the same type of diagnostics explored in section S1 1.3.1.5. For example, we can look at qqplots to check normality and use the autocorrelation function to look at unaccounted temporal correlation.

```
qqnorm(res2pTmb$residual,
       main="", pch=16, cex=0.8)
qqline(res2pTmb$residual, col="hotpink", lwd=2)
acf(res2pTmb$residual)
```

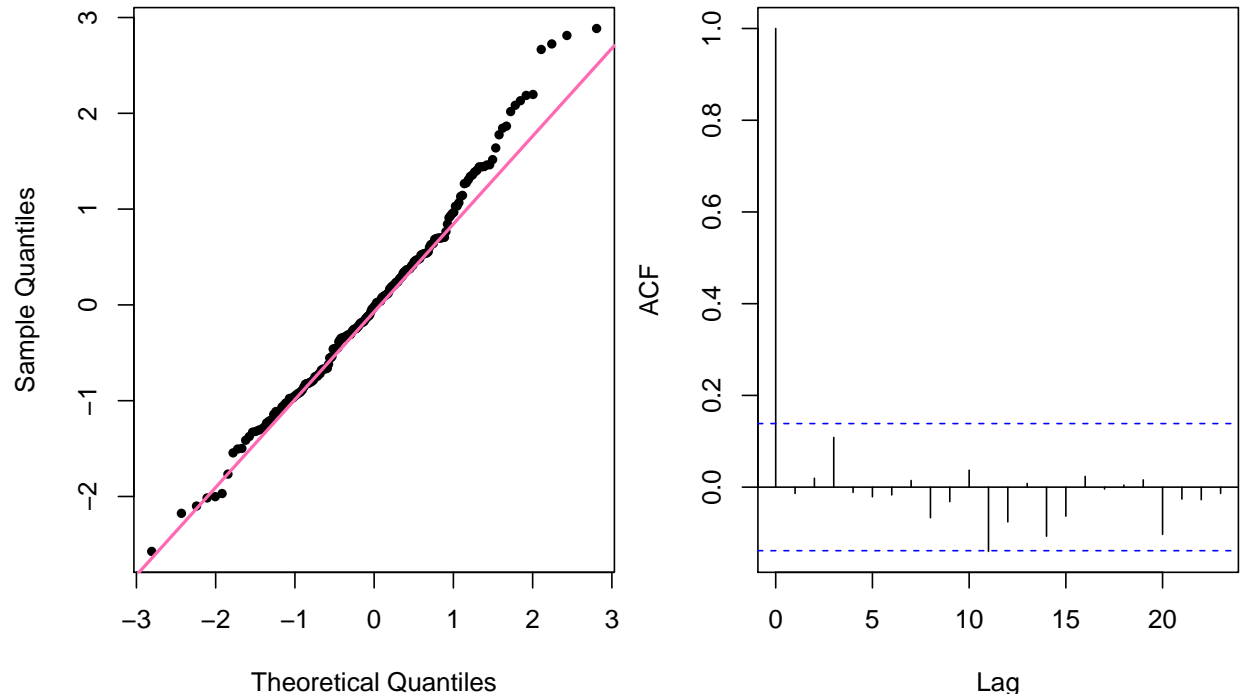

Figure S1.18: Diagnostics using TMB's one-step-ahead residuals.

When we use TMB, it is important to assess whether the Laplace approximation is adequate. To check the Laplace approximation and simulation consistency, we can use the function `checkConsistency`.

```
set.seed(12345)
checkConsistency(m2pTmb)

## Parameters used for simulation:
##   logSdP   logSd0
## -2.142005 -2.392282
##
## Test correct simulation (p.value):
## [1] 0.18758
## Simulation appears to be correct
##
## Estimated parameter bias:
##       logSdP       logSd0
## -0.0006559141 -0.0044785996
```

Here we can see that the p-value for the simulations is high, and above the 0.05 significance level, and thus we are confident that the simulation is consistent with the implemented negative log-likelihood function.

The size of the estimated biases for the parameters are both small, indicating that Laplace approximation is not inducing large biases<sup>3</sup>. See `?checkConsistency` for more details.

### S1 1.3.2.7 Using the likelihood profile to check parameter estimates

To assess whether you may have encountered parameter estimation problems, it is useful to look at the likelihood profile. We can use TMB's function `tmbprofile` to do this quickly. For example, let us look at the likelihood profile of the process variation parameter of the simple model.

```
profLikSdp2pTmb <- tmbprofile(m2pTmb, "logSdP", trace=FALSE)
plot(profLikSdp2pTmb, las=1)
```

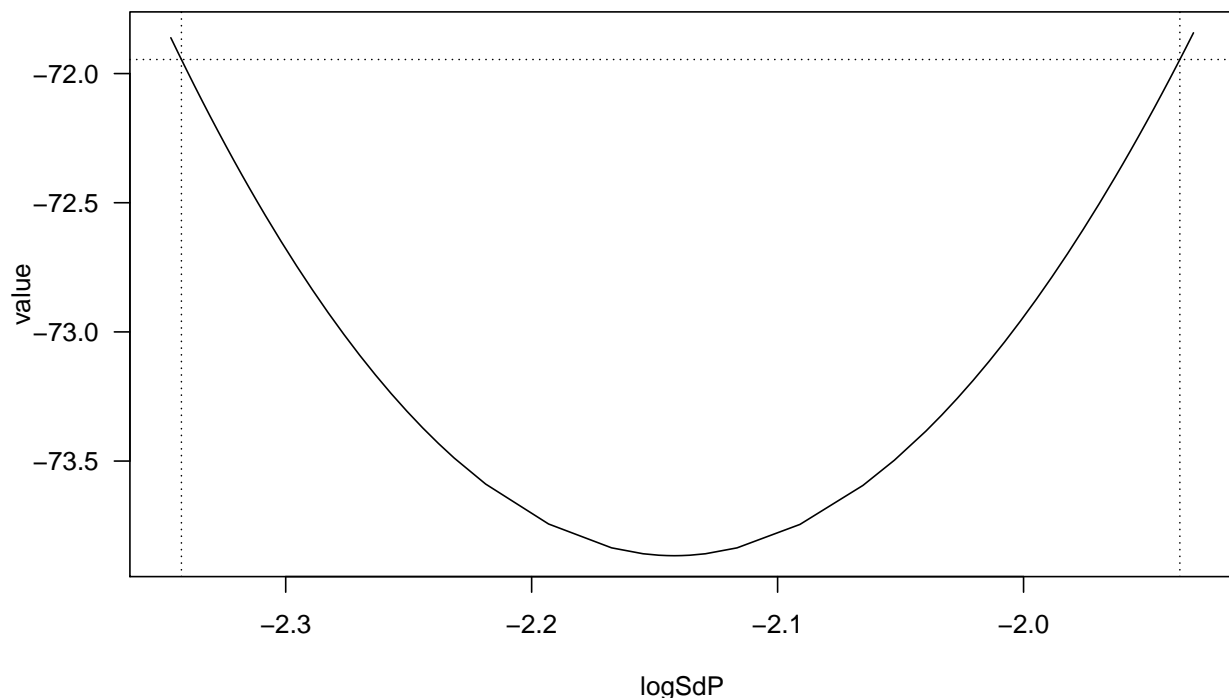

Figure S1.19: Profile of the negative log likelihood of the log process variation standard deviation.

Note that what is returned is a plot of the negative log likelihood. We can see here a single minimum peak, suggesting that there is no identifiability issue. One can use the `tmbprofile` argument `ytol` to widen the range of parameter values explored.

---

<sup>3</sup>If the function returns NA, install TMB from Github (<https://github.com/kaskr/adcomp/>) rather than from CRAN. If using a Mac, you may need to add `SHLIB_OPENMP_CFLAGS=` in the Makevars file.

```
profLikSdp2pTmb <- tmbprofile(m2pTmb, "logSdP", trace=FALSE, ytol=20)
plot(profLikSdp2pTmb, las=1)
```

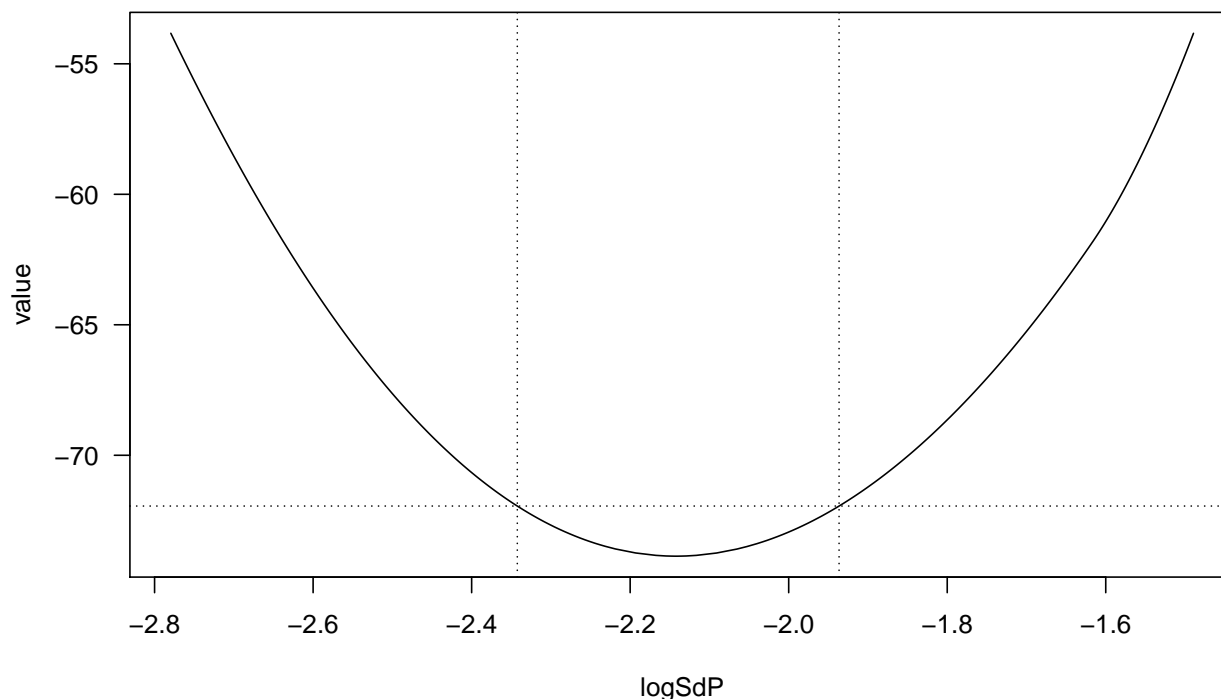

Figure S1.20: Expanded range of the profile of the negative log likelihood of the log process variation standard deviation.

Even with a wider parameter range, we still have one peak further suggesting that there is no obvious identifiability problems.

One additional perk of this function is that we can use it to calculate confidence intervals.

```
confint(profLikSdp2pTmb)

##           lower      upper
## logSdP -2.342395 -1.936447
```

Now let us look at the likelihood profile of the parameters of the more flexible model, where we estimate the two standard deviations as well as  $\alpha$  and  $\beta$ . This code may take a few minutes to run.

```

profLikSdp4pTmb <- tmbprofile(m4pTmb, "logSdP", trace=FALSE, ytol=20)
plot(profLikSdp4pTmb, las=1)
profLikBeta4pTmb <- tmbprofile(m4pTmb, "beta", trace=FALSE, ytol=20)
plot(profLikBeta4pTmb, las=1)
profLikSdo4pTmb <- tmbprofile(m4pTmb, "logSdO", trace=FALSE, ytol=20)
plot(profLikSdo4pTmb, las=1)
profLikAlpha4pTmb <- tmbprofile(m4pTmb, "alpha", trace=FALSE, ytol=20)
plot(profLikAlpha4pTmb, las=1)

```

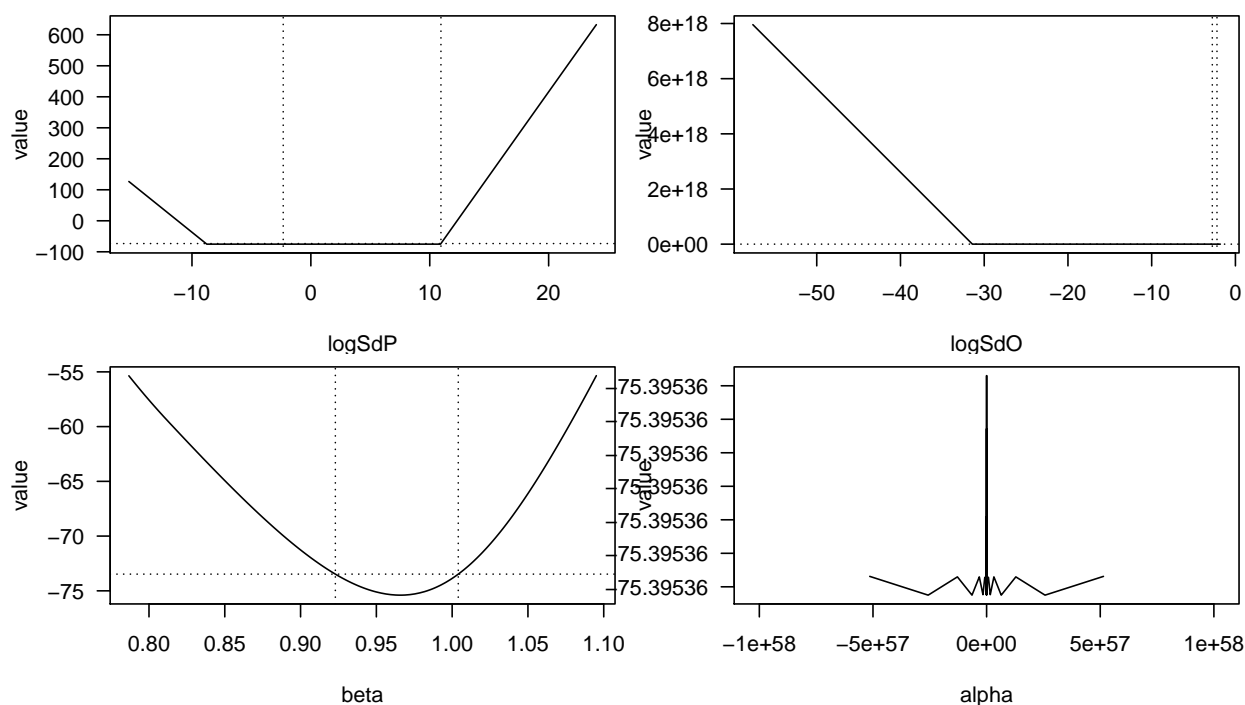

Figure S1.21: Profile of the negative log likelihood of the parameters of the more flexible model.

We can see that for this more complex model we have estimation problems. The likelihood profile is flat in many places, indicating that multiple parameter values will return the same likelihood value. We may even get warning messages. As mentioned in Appendix S3 this identifiability problem appears to be mostly occurring when  $z_0 = 0$ .

### S1 1.3.3 Sequential Monte Carlo method

To demonstrate the general approach of Particle Filtering (PF), we begin with Sequential Importance Sampling (SIS) and will next apply a better method, Bootstrap Filtering.

### S1 1.3.3.1 Sequential Importance Sampling.

We will use SIS to estimate the underlying states conditional on the entire vector of observation, in particular estimates of the conditional expected values, i.e., the smoothed state estimates:  $E[z_t|y_{1:T}]$ ,  $t=1, \dots, T$ . We are using here the simpler toy SSM (Eqs. 1.3-1.4). The SSM parameters are treated as known values, which in this model are the initial state value,  $z_0$ , and the process and observation standard deviations.

The output from SIS includes an  $N$  by  $T + 1$  matrix of simulated states ( $\mathbf{Z}^*$ ) and a length  $N$  vector of weights ( $\mathbf{w}$ ). Each row of the matrix is a single simulated time series realization of the states; i.e., row  $i$  has the values  $z_0^i, z_1^i, \dots, z_T^i$ , and each such row is referred to as a particle. Associated with each particle (time series) is a weight,  $w^i$  for particle  $i$ . A visual display of the matrix simulated states and the weight vector is shown below:

$$\mathbf{Z}^* = \begin{bmatrix} z_0^1 & z_1^1 & \dots & z_T^1 \\ z_0^2 & z_1^2 & \dots & z_T^2 \\ \vdots & \vdots & \dots & \vdots \\ z_0^N & z_1^N & \dots & z_T^N \end{bmatrix} \quad (1.11)$$

$$\mathbf{w}'_T = [w_T^1, w_T^2, \dots, w_T^N] \quad (1.12)$$

The vector of weights is subsequently scaled to sum to one,  $w_T^{*,i} = w_T^i / \sum_{j=1}^N w_T^j$ , and can be used to estimate the smoothed state value at time  $t$ ,  $\hat{z}_{t|1:T}$ , as a weighted average:  $\hat{E}[z_t|y_{1:T}] = \sum_{i=1}^N w_T^{*,i} z_t^i$ . As particles with higher weights are more likely to have produced the data, when we predict the states, we take the average value of the particles for each time step weighted by their overall likelihood.

The SIS algorithm for producing the matrix  $\mathbf{Z}^*$  and the vector  $\mathbf{w}_T$  is an iterative, “sequential”, procedure. Given a length  $N$  vector of the initial state,  $z_0$  (in this case set equal to 0, the true values), a second length  $N$  vector for state  $z_1$  is generated directly from the process equation (Eq. 1.3). A vector of  $z_2$  values is then generated from the just simulated  $z_1$  values, and the procedure is repeated till time  $T$ . The vector of weights is calculated by initially setting all values equal to 1.0. After the vector of  $z_1$  values is generated, the weight vector is multiplied by the observation equation (Eq. 1.4) for  $y_1$  evaluated at each of the simulated  $z_1$  values, i.e., at time  $t$  for particle  $i$ :

$$w_t^i = w_{t-1}^i g(y_t|z_t^i) \quad (1.13)$$

where  $g(y_t|z_t^i)$  is the probability density for  $y_t$ .

As a first step, let us set up the procedure, by setting the seed, defining the number of particles, and creating a matrix, `ziOpSis`, corresponding to  $\mathbf{Z}^*$  above, that will keep track of the values of all particles at each time step  $t$ ,  $z_t^i$ . As we assumed when we simulated the model, we set the initial state value,  $z_0$ , to be 0. As such, our matrix had `TT+1` columns and the first column has 0s.

```
set.seed(102) # To be able to reproduce the simulation
N <- 100000 # Number of particles
ziOpSis <- matrix(data=NA, nrow=N, ncol=TT+1) # To store all simulated states
ziOpSis[,1] <- 0 # Set z_0 = 0
```

Then, we need to create a matrix that will keep track of the weights of particles. The weight of a particle will change at each time step, but it starts at 1 for all particles, as they are all equal at first.

```
w0pSIS <- rep(1,N)
```

Now we can start the particle propagation, where at each time step we use the process equation to sample the particle value at the next time step. We also update the weight of the particle by multiplying the weight from the previous step to that of the probability density function associated with the observation equation. Note that because the state particle matrix starts at  $t = 0$  but the observations start at time  $t = 1$ , we compare  $y[t-1]$  to  $zi0pSis[,t]$ .

```
for(t in 2:(TT+1)){
  # Propagate the particles
  zi0pSis[,t] <- rnorm(n=N, mean=zi0pSis[,t-1], sd=sdp)
  # Update the weights
  w0pSIS <- w0pSIS*dnorm(y[t-1], mean=zi0pSis[,t], sd=sdo)
}
```

We can look at the first five time steps for six particles and look at their weight.

```
head(zi0pSis[,2:6])

##           [,1]           [,2]           [,3]           [,4]           [,5]
## [1,]  0.01805229 -0.05037868 -0.0902529 -0.2844048 -0.14609386
## [2,]  0.07847340  0.01871548  0.2086525  0.2938260  0.35144209
## [3,] -0.13531646 -0.06403487 -0.1661191 -0.1389578 -0.05778625
## [4,]  0.19832982  0.10369391  0.1002379  0.1240146  0.23186680
## [5,]  0.12384717  0.14913226  0.3147150  0.4545146  0.42472425
## [6,]  0.12006174  0.17189787  0.1770619  0.1851515  0.34122268

head(w0pSIS)

## [1] 0 0 0 0 0 0
```

We can see that the state values of the particles vary a fair bit and that the weights of all six particles are 0. This is an example of the particle depletion, where the simulated particle path is so unlikely that its weight becomes effectively 0. Let us see how many particles have non-negligible weights.

```
sum(w0pSIS > 0)

## [1] 32
```

Only  $3.2 \times 10^{-4}$  % of particles are useful.



Ignoring this problem, the next step is to take the weighted average value of the particles. This weighted average is our smoothed estimate of the states. To make sure that estimated value makes sense, we need to first scale the weight so they sum to 1.

```
# Scales the weights to sum to 1
wOpSIS <- wOpSIS/sum(wOpSIS)
# Calculate the state estimates using the weights
zsOpSIS <- colSums(wOpSIS*ziOpSis)
```

Let us plot the estimated states on the simulated data.

```
plot(1:TT, y,
     pch=3, cex = 0.8, col="blue", ty="o", lty = 3,
     xlab = "t", ylab = expression(z[t]),
     xlim = c(0,TT), ylim = c(min(y), max(y)+max(y)/5),
     las = 1)
points(0:TT, z,
       pch = 19, cex = 0.7, col = "red", ty = "o")
lines(0:TT, zsOpSIS,
      col="darkgoldenrod1", lwd = 2, lty = 5)
legend("top",
      legend = c("Obs.", "True states", "Smooth. states"),
      pch = c(3, 19, NA),
      col = c("blue", "red", "darkgoldenrod1"),
      lwd = c(1, 1, 2), lty = c(3, 1, 5),
      horiz=TRUE, bty="n", cex=0.9)
```

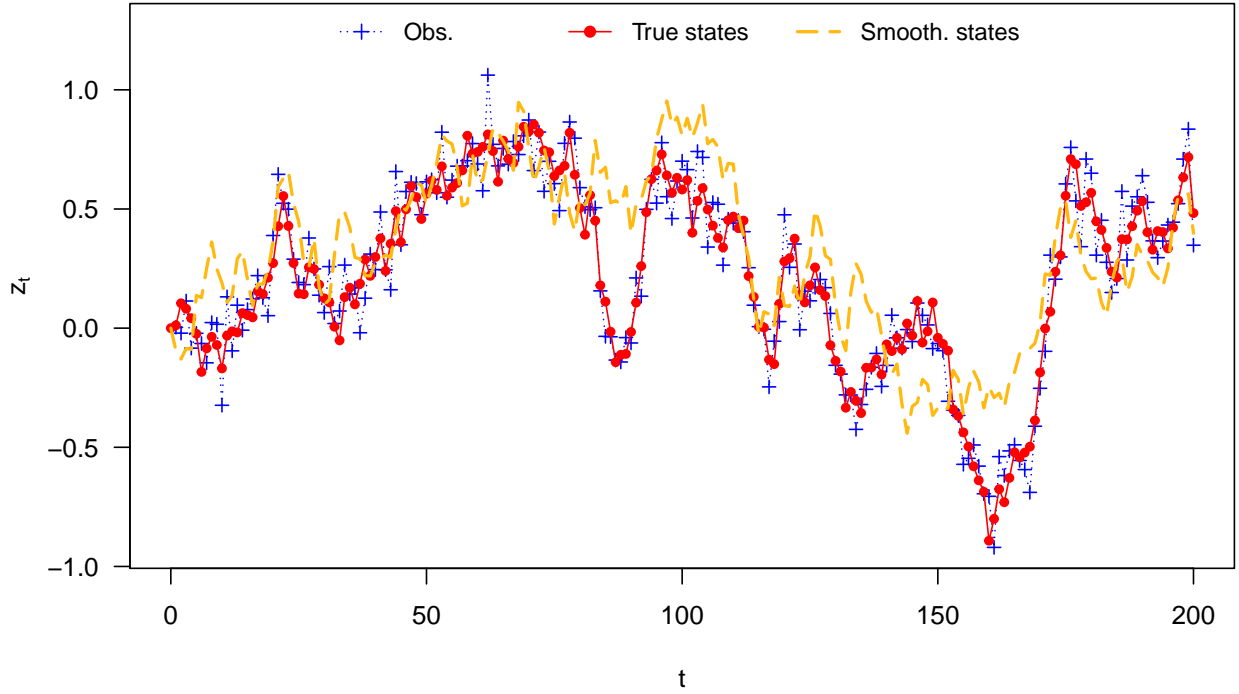

Figure S1.22: State estimates from SIS along with the true states and observations.

We can see that the state estimates are not fantastic, particularly for low  $z_t$  values. This is largely due to the problem of particle depletion. If the SIS process was repeated, with a different seed, the resulting state estimates are likely to vary considerably, i.e., there is high Monte Carlo variation. Increasing the number of particles, using  $N=2$  million for example, is a partial remedy. However, as the time series length increases, the problem of particle depletion and Monte Carlo variation worsens. The Bootstrap Filter, which is explained next, is a modification of SIS aimed at lessening the problem of particle depletion, although the problem will remain at some level.

### S1 1.3.3.2 SIS with bootstrap filter

Now let us look at a SIS with bootstrap filter. The idea behind the bootstrap filter is to sequentially sample the particles at each time step  $t$  according to the weights at time  $t$ . Because particles with low weight are unlikely to be sampled, this should limit particle depletion. Like SIS, to generate the  $z_t$  at time  $t$ , we use the process equation to generate  $z_t$  conditional on  $z_{t-1}$ . The key difference is that the vector of  $z_{t-1}$  values used to generate the  $z_t$  values are not the original set of  $N$   $z_{t-1}$  values generated at time  $t-1$ . Instead the vector of  $z_{t-1}$  values used are a random sample, selected with replacement and proportional to the weights as of time  $t-1$  (what is potentially confusingly called a resample), from that originally generated set. In fact, state matrix as of time  $t-1$  is a resampled matrix, where the entire rows have been sampled with replacement according the (scaled) weight vector as of time  $t-1$  (see main text). Thus, time series vectors with higher weights are more likely selected than those with lower weights, thus some rows in the resampled

matrix are duplicates of rows in the matrix prior to resampling, while other rows that were in the matrix are now completely gone.

As a simple demonstration, suppose we have three particles ( $N = 3$ ) and the states at time  $t=4$  are to be generated. First simulate new proposed values for time  $t = 3$ :

$$\tilde{\mathbf{Z}}^*[1:3, 0:3] = \begin{bmatrix} 0 & 0.9 & 1.1 & 0.8 \\ 0 & -0.2 & 0.5 & 0.7 \\ 0 & 0.6 & 0.8 & 0.3 \end{bmatrix}. \quad (1.14)$$

Then, calculate the un-normalized weight of each particle using the observation equation:

$$\mathbf{w}_3^* = \begin{bmatrix} 0.04 \\ 0.02 \\ 0.05 \end{bmatrix}. \quad (1.15)$$

The rows of the proposed particles  $\tilde{\mathbf{Z}}^*[1:3, 0:3]$  are sampled with replacement with probabilities equal to the scaled weights: `sample(1:3,size=3,prob=c(0.36364, 0.18182 0.45454))` with the results 3,3,2. Thus, the resampled matrix has row 3 twice, row 2 once, and row 1 is now gone:

$$\mathbf{Z}^*[1:3, 0:3] = \begin{bmatrix} 0 & 0.6 & 0.8 & 0.3 \\ 0 & 0.6 & 0.8 & 0.3 \\ 0 & -0.2 & 0.5 & 0.7 \end{bmatrix}. \quad (1.16)$$

The weight calculations are simplified with the bootstrap filter. Because we resample based on the weight, there is no sequential updating of the weights.

For a numerical example, let us start as before by setting up the procedures.

```
set.seed(338) # Set random seed
# Matrix that keeps track of particles
ziOpBf <- matrix(data=NA, nrow=N, ncol=TT+1)
ziOpBf[,1] <- 0 # Set z_0 = 0
# Create weight vector
wOpBf <- rep(1,N)
# This matrix keeps track of the number of retained original particles
histOpBf <- matrix(data=NA, nrow=N, ncol=TT+1)
histOpBf[,1] <- 1:N
```

Now we can start generating the particles. At each time step, we: 1) sample from the process equation (Eq. 1.3), 2) calculate the weight using the probability density function associated with the observation equation (Eq. 1.4), and 3) resample the particles based on their weight.

```
for(t in 2:(TT+1)){
  # Sample from the process equation
  ziOpBf[,t] <- rnorm(n=N, mean=ziOpBf[,t-1], sd=sdp)
  # Calculate the weight from observation equation
```

```

wOpBf <- dnorm(y[t-1], mean=ziOpBf[,t], sd=sdo)
# Resample the particles based on weight
resampOpBf <- sample(1:N, N, replace=TRUE, prob=wOpBf)
# Replace particles by resampled ones
ziOpBf[,1:t] <- ziOpBf[resampOpBf, 1:t]
# Add to the listing of retained particles
histOpBf[,t] <- histOpBf[resampOpBf,t-1]
}

```

Here, the weight will not tell us if we have particle depletion because it only represents the weight at a given time step rather than the overall weight of the particle. However, since we are resampling, we may end up with only a few parent particles. Let us look at the particles.

```

head(ziOpBf[,2:6])

```

|         | [,1]        | [,2]         | [,3]        | [,4]          | [,5]        |
|---------|-------------|--------------|-------------|---------------|-------------|
| ## [1,] | 0.07535301  | 0.158531740  | 0.073113483 | 0.0517030222  | -0.01090048 |
| ## [2,] | -0.05331083 | 0.005377253  | 0.032215100 | -0.0622257157 | -0.09413141 |
| ## [3,] | -0.07749822 | -0.065915384 | 0.019661625 | -0.0938259490 | -0.02542868 |
| ## [4,] | -0.06217534 | -0.011376135 | 0.082542380 | -0.0501783094 | 0.02137679  |
| ## [5,] | 0.05700603  | 0.105859482  | 0.086391208 | 0.0005223168  | 0.01395669  |
| ## [6,] | -0.10123834 | 0.058805931  | 0.006395101 | -0.0385428287 | -0.03079425 |

At least these six particles are not the same, so that is a good sign. Examination of the “history” matrix is more informative as it kept track of how many of the originally generated  $N=100,000$  particles are used. To find out how many unique particles are used at the end, we can simply look at the number of unique values in the last time step.

```

length(unique(histOpBf[,TT+1]))

```

```

## [1] 252

```

We can also look at the number of particles retained throughout the 200 time points:

```

num.unique <- apply(histOpBf,2,function(x) length(unique(x)))
plot(1:(TT+1), num.unique,
     xlab="Time t", ylab="", type="l", las=1,
     main="Number of original particles at each time point")

```

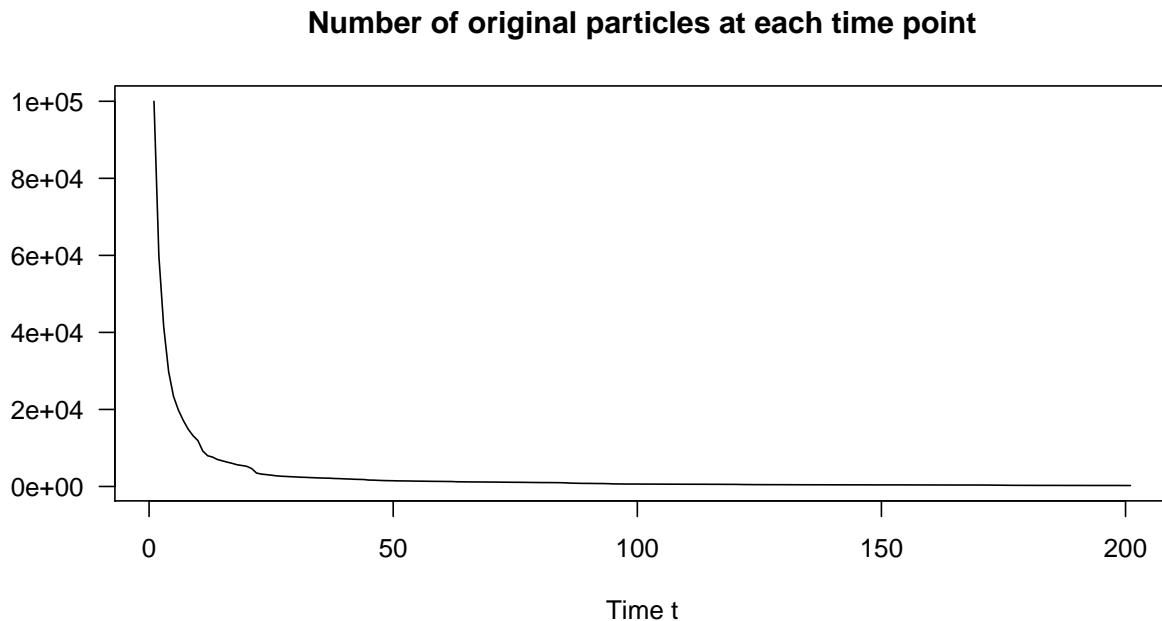

Figure S1.23: Temporal depletion in the number of unique particles in the bootstrap filter.

Thus 0.252 % of the originally generated particles were retained. This is better than for the SIS example we had above, but still quite small.

Now let us look at estimated state values. Here, since the weight is used to resample, we do not need to take a weighted average. We can simply take the average.

```
zs0pBf <- colMeans(zi0pBf)
```

Let us visually compare SIS and BF.

```
plot(1:TT, y,
     pch=3, cex = 0.8, col="blue", ty="o", lty = 3,
     xlab = "t", ylab = expression(z[t]),
     xlim = c(0,TT), ylim = c(min(y), max(y)+max(y)/5),
     las = 1)
points(0:TT, z,
       pch = 19, cex = 0.7, col = "red", ty = "o")
lines(0:TT, zs0pSIS,
      col="darkgoldenrod1", lwd = 2, lty = 5)
lines(0:TT, zs0pBf,
```

```

col="cyan3", lwd = 3)
legend("top",
  legend = c("Obs.", "True states", "States SIS", "States BF"),
  pch = c(3, 19, NA, NA),
  col = c("blue", "red", "darkgoldenrod1", "cyan3"),
  lwd = c(1, 1, 2, 3), lty = c(3, 1, 5, 1),
  horiz=TRUE, bty="n", cex=0.9)

```

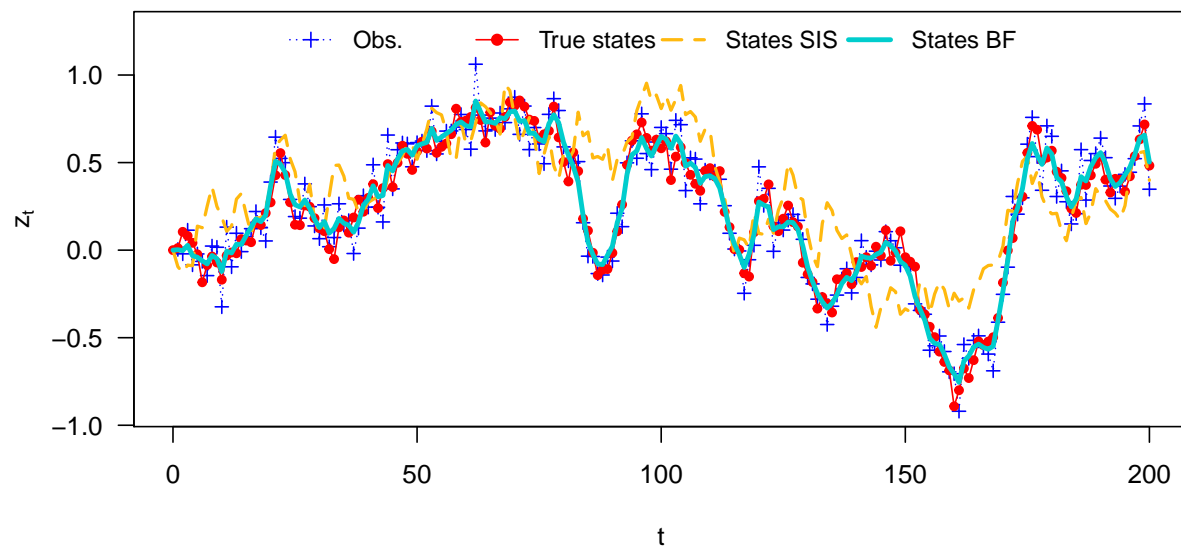

Figure S1.24: Time series of state estimates using SIS and bootstrap filter.

We can see that the bootstrap filter really improves the state estimates. This is further clarified by looking at the plots of the true simulated state values,  $z_t$ , vs the estimated state values  $\hat{z}_t$ .

```

# SIS zhat vs z
plot(z, zs0pSIS,
  xlab=expression(z[t]), ylab=expression(hat(z)[t]), las=1,
  main="SIS: Smoothed vs True States",
  pch=19, col="darkgoldenrod1", cex=0.5)
abline(0,1)

```

```
# BF zhat vs z
plot(z, zs0pBf,
     xlab=expression(z[t]), ylab=expression(hat(z)[t]), las=1,
     main="Bootstrap Filter:Smoothed vs True States",
     pch=19, col="cyan3", cex=0.5)
abline(0,1)
```

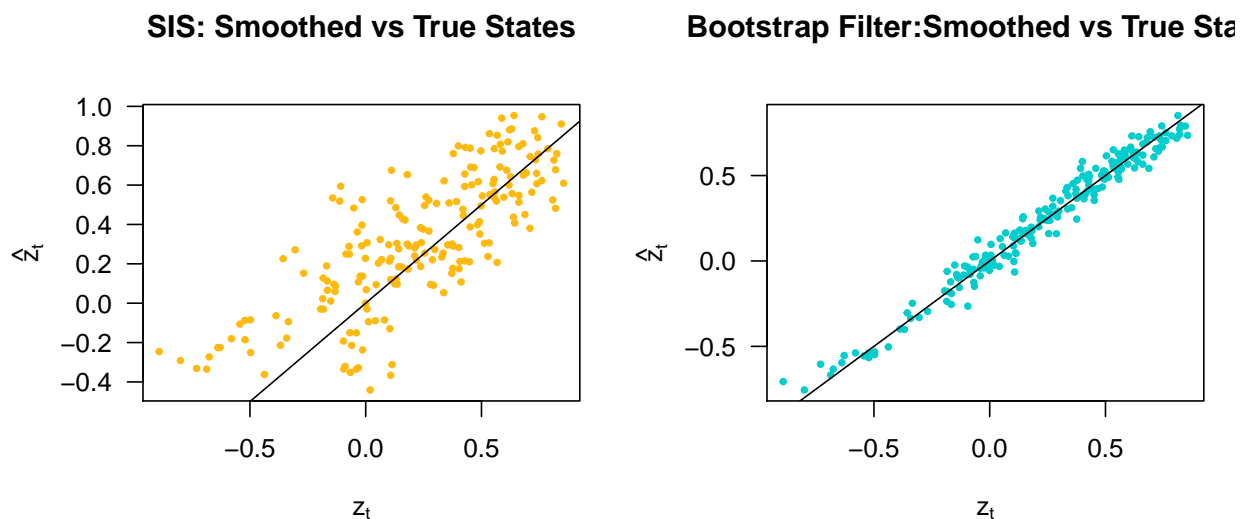

Figure S1.25: Comparison of the state estimates with their true simulated values using SIS and bootstrap filter.

One of the great advantages of particle filter techniques is that it allows the researcher to explore process equations for which it would be difficult to write down a proper likelihood. With particle filter methods, as long as you can simulate from the process and you have a proper likelihood function for the observation which can be evaluated, you are good to go. Here we only demonstrated how to estimate the states. To estimate the parameters would require creating a function that performs SIS or BF as a function of parameter values and then optimize the parameter values. Due to parameter depletion, this can be quite challenging. It is useful to look at the package **pomp**, see below, which implements iterated filtering (IF) to help with this issue.

### S1 1.3.4 **pomp**

In this section, we show how to implement the simple model of section S1 1.1 in the **pomp** package (King et al., 2016). For computational efficiency, **pomp** compiles C, and thus requires a C compiler. As with

TMB, Windows users are thus required to install `Rtools` and Mac OS users are required to install `Xcode`. Detailed installation instructions are available on the `pomp` website: <https://kingaa.github.io/pomp/install.html> and troubleshooting tips can be found at: <https://kingaa.github.io/pomp/FAQ.html>. Since compilers are ordinarily included in Linux installations, no additional installations are typically required for Linux users.

Here, we demonstrate one of `pomp`'s approach to the estimation of parameters and filtered trajectories of the state process.

```
library(pomp)
```

As for most packages we have seen so far, the first step is to construct an object (called a “`pomp` object”) that describes the model in the language of the package. Here, we create a `pomp` object that describes the simpler version of the toy model (Eqs. 1.3-1.4). The constructor has several important arguments, the first of which is `data`: this takes a data frame containing the observations along with the time of each observation<sup>4</sup>. Let us therefore create such a data frame.

```
dataPomp <- data.frame(t=1:TT, y=y)
```

The `pomp` object constructor is given information about the model via several arguments: `rprocess` describes a procedure for simulating the process equation; `rmeasure` describes one for simulating the observation equation; `dmeasure` describes how to compute the probability of each observation; and `rinit` parameterizes the initial state value. Each of these is most simply specified via an R function, as we show below.

When constructing the `pomp` object, we indicate which of the variables in the `data` data frame is the time variable via the `times` argument. We specify the time of the initial state using `t0`. We can also use the `partrans` argument to provide parameter transformations.

```
m2pPomp <- pomp(  
  data = dataPomp,  
  times='t', t0=1,  
  rprocess=discrete_time(  
    function (z, sdp, ...) {  
      c(z=rnorm(n=1, mean=z, sd=sdp))  
    }  
  ),  
  rmeasure=function (z, sdo, ...) {  
    c(y=rnorm(n=1, mean=z, sd=sdo))  
  },  
  dmeasure=function (y, z, sdo, log, ...) {  
    dnorm(x=y, mean=z, sd=sdo, log=log)  
  },  
  rinit=function (...) {
```

---

<sup>4</sup>It could also be another `pomp` object.



```

    c(z=0)
  },
  partrans = parameter_trans(log=c("sdp", "sdo")),
  paramnames=c("sdp", "sdo")
)

```

Notice that the `paramnames` argument appears here: it names the parameters that are being transformed.

Note also that the `dmeasure` function takes a `log` argument: if `log = TRUE`, this function should return the log probability density.

One obtains much faster computation using the alternative “C snippet” interface provided by **pomp**, as follows.

```

m2pPomp <- pomp(
  data = dataPomp,
  times='t',
  t0=1,
  rprocess=discrete_time(Csnippet("z = rnorm(z,sdp);")),
  rmeasure=Csnippet("y = rnorm(z,sdo);"),
  dmeasure=Csnippet("lik = dnorm(y,z,sdo,give_log);"),
  rinit=Csnippet("z = 0;"),
  partrans = parameter_trans(log=c("sdp", "sdo")),
  paramnames=c("sdp", "sdo"),
  statenames=c("z")
)

```

With a **pomp** object in hand, **pomp** provides many functions for working with the model and the data. For example, we can use `simulate` to simulate data from the model. In particular, to perform a simple particle filter computation, we use the function `pfilter`. If we desire the filtered state estimates, we set the argument `filter.mean` to `TRUE`. The following code runs such a particle filter using 2000 particles.

```

pf0pPomp <- pfilter(
  m2pPomp,
  Np=2000,
  params=c(sdp=sdp, sdo=sdo),
  filter.mean=TRUE
)

```

When we plot the results from `pfilter`, we see, among other things, how the effective sample size changes through time and the filtered state estimates.

```
plot(pf0pPomp)
```

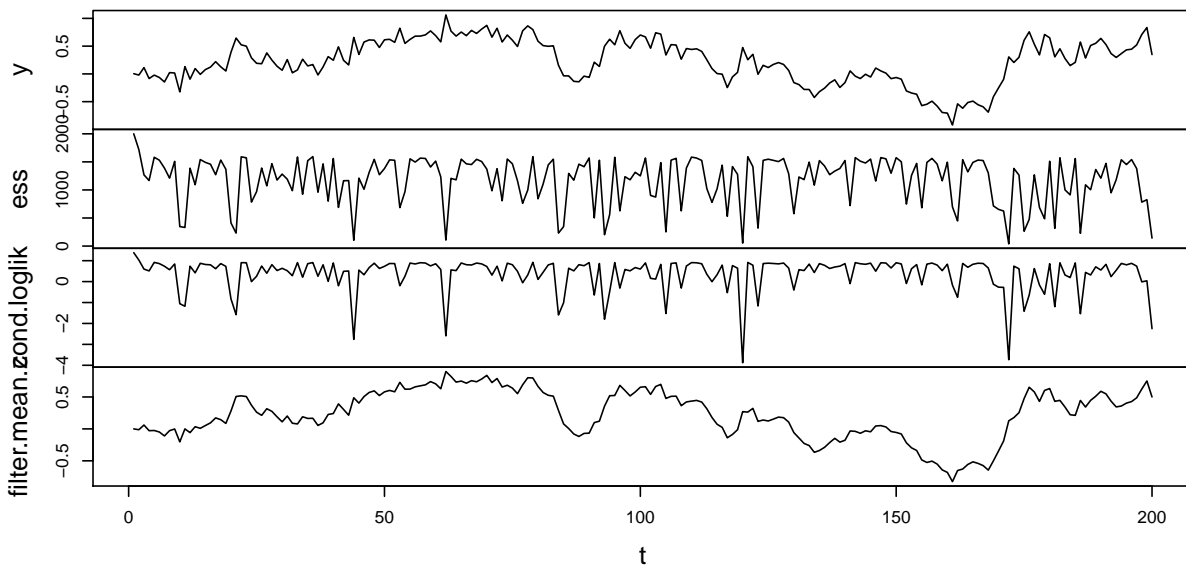

Figure S1.26: Diagnostic plots from `pfilter`. From top to bottom are displayed: the data, the *effective sample size* of the filter, the log likelihood of each observation conditional on the preceding ones, and the estimates of the state process  $z$  (the *filter mean*).

To extract the state estimates, we use the function `filter.mean`. To extract the estimated log likelihood, we can use the function `logLik`. This log likelihood depends on the simulated state values, and thus will change every time you run the `pfilter` function.

```
zf0pPomp <- filter.mean(pf0pPomp)
logLik(pf0pPomp)

## [1] 73.51225
```

To estimate of the uncertainty in the log likelihood, we need to run the particle filter multiple times. It is useful to use parallel computing to expedite the process. Here, we load packages that will facilitate parallelizing the computations.

```
library(doParallel)
library(doRNG)
```

To be able to do the process in parallel we need to register the parallel backend for the foreach function and set the random seed.

```
registerDoParallel()
registerDoRNG(1301370376)
```

Here, we run the particle filter multiple times. To get an estimate of the log likelihood we then take the average with the function `logmeanexp`. This function allows to calculate the log mean while avoiding over and under flow.

```
# Run particle filter 10x
pfsOpPomp <- foreach(i=1:10, .combine=c, .packages=c("pomp")) %dopar% {
  pfilter(m2pPomp, Np=2000, params=c(sdp=sdp, sdo=sdo))
}
# Extract all of the log likelihoods
logLik(pfsOpPomp)

## [1] 73.89884 73.93212 72.18766 71.81398 72.65202 72.49160 72.51926 72.74673
## [9] 72.45887 73.79859

# Calculate the log of the mean of the estimated likelihoods
logmeanexp(logLik(pfsOpPomp), se=TRUE)

##
##          se
## 73.118008 0.261995
```

So far, we have only looked at Monte Carlo methods to estimate the states. If we want to estimate the parameters, an attractive option is to find the parameters that maximize the likelihood. As discussed in the main text, we can use iterated filtering (IF) to do so: in **pomp**, this is implemented as the function `mif2`. As its first argument, this function takes the pomp object describing the model, here `m2pPomp`. As with most optimizers, we need to specify starting values for our parameters: here, we choose the true values (values we used to simulate the data). We also need to specify how many filtering iterations to perform (`Nmif`), the number of particles to use in each iteration (`Np`), the magnitude of the perturbations applied to each of model parameters at each observation (`rw.sd`), and the rate at which the intensity of these perturbations is reduced as the algorithm proceeds (`cooling.fraction`). The main text describes how iterative filtering works.

```
f2pPomp <- mif2(
  m2pPomp,
  params = c(sdp=0.1, sdo=0.1),
  Nmif=50, Np=2000,
  rw.sd= rw.sd(sdp=0.005, sdo=0.005),
  cooling.fraction.50=0.5
)
```

We can use the function `plot` to look at how the parameters and log likelihood changes through different iterations of the process.

```
# Diagnostic plots
plot(f2pPomp)
```

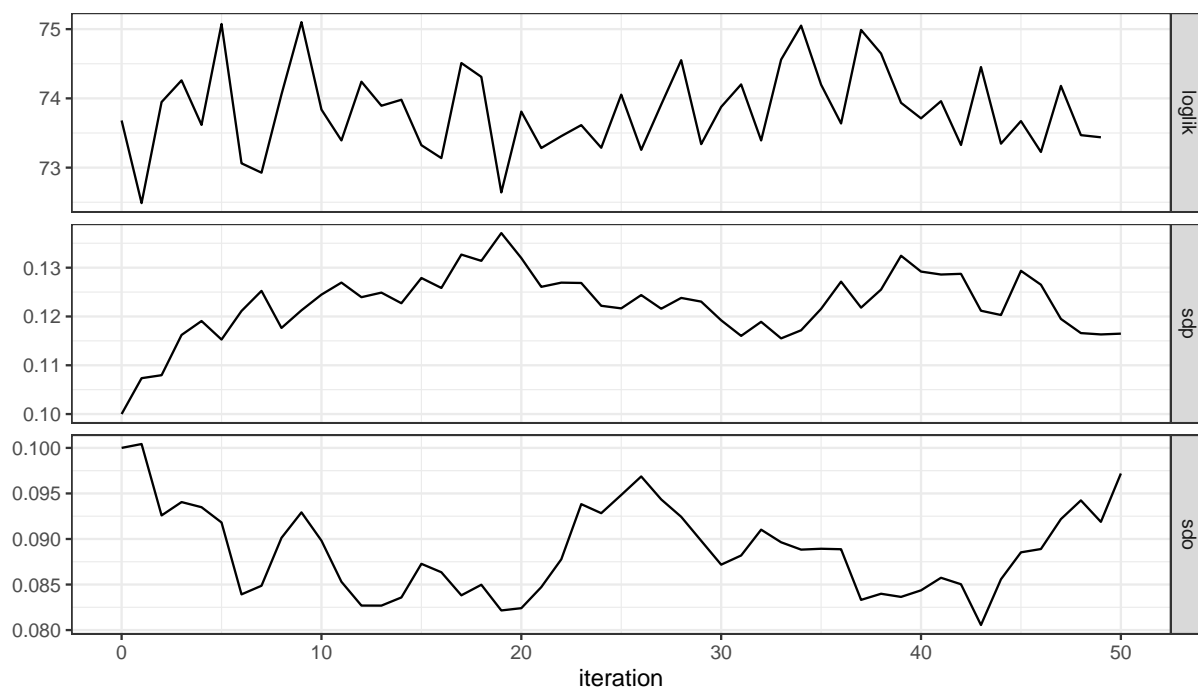

Figure S1.27: Diagnostic plots from `mif2`. Each trace shows how the variable indicated changed with filter iteration.

The function `coef` will return the point estimates of the parameters.

```
# Estimates
cbind("True"=c(sdp, sdo), "Estimated"=coef(f2pPomp))

##      True Estimated
## sdp  0.1 0.11647762
## sdo  0.1 0.09718817
```

The function `logLik` applied to `f2pPomp`, will return the estimated log likelihood of the perturbed model (i.e., the model with parameters that are random variables). To get the (more relevant) log likelihood of the model with fixed parameters, we would, as above, run the particle filter multiple times and get the mean value. In the preceding, we have cheated slightly in that we used the true parameter values as starting values, likely helping the optimizer.

With real data, we do not know the true values of the parameters. To help increase our chance of finding the global maximum, it is helpful to run the optimizer with multiple different starting values. We can use the function `runifDesign` to create a set of random starting values for our parameters. All we need to specify is the lower and upper values we think each parameter could have. Here, we know that the standard deviation should be bounded at 0, and we somewhat arbitrarily set the upper bound to 1. We also specify how many start values we want to have (here 100).

```
guesses <- runifDesign(
  lower=c(sdp=0, sdo=0),
  upper=c(sdp=1, sdo=1),
  nseq=100
)
head(guesses)

##      sdp      sdo
## 1 0.2319292 0.4456504
## 2 0.6359523 0.3975456
## 3 0.1354265 0.7929366
## 4 0.7455454 0.1119596
## 5 0.5873958 0.4719982
## 6 0.5734615 0.3391000
```

Using `foreach`, we then run `mif2` using each of the starting values sets. If, as in the present case, we have already run `mif2`, we can just feed the resulting of the previous calculation to `mif2`. The new computation, will be run using all the same settings as before, though we can change individual settings at will. The only thing we wish to change in this case is the starting point. This code may take a long time to run and it will use a lot of CPU.

```
fg2pPomp <- foreach(
  guess=iter(guesses, "row"), .combine=c,
  .packages=c("pomp"), .errorhandling="remove",
  .inorder=FALSE
) %dopar% {
  mif2(f2pPomp, params=guess)
}
```

Again, we examine diagnostic trace plots.

```
library(ggplot2)
library(magrittr)
fg2pPomp %>%
  traces() %>%
  melt() %>%
  subset(variable!="nfail") %>%
  ggplot(aes(x=iteration,y=value,group=L1,color=factor(L1)))+
  geom_line()+
  facet_wrap(~variable,ncol=1,scales="free_y",strip.position="right")+
  guides(color=FALSE)+
  labs(y="")+
  theme_bw()
```

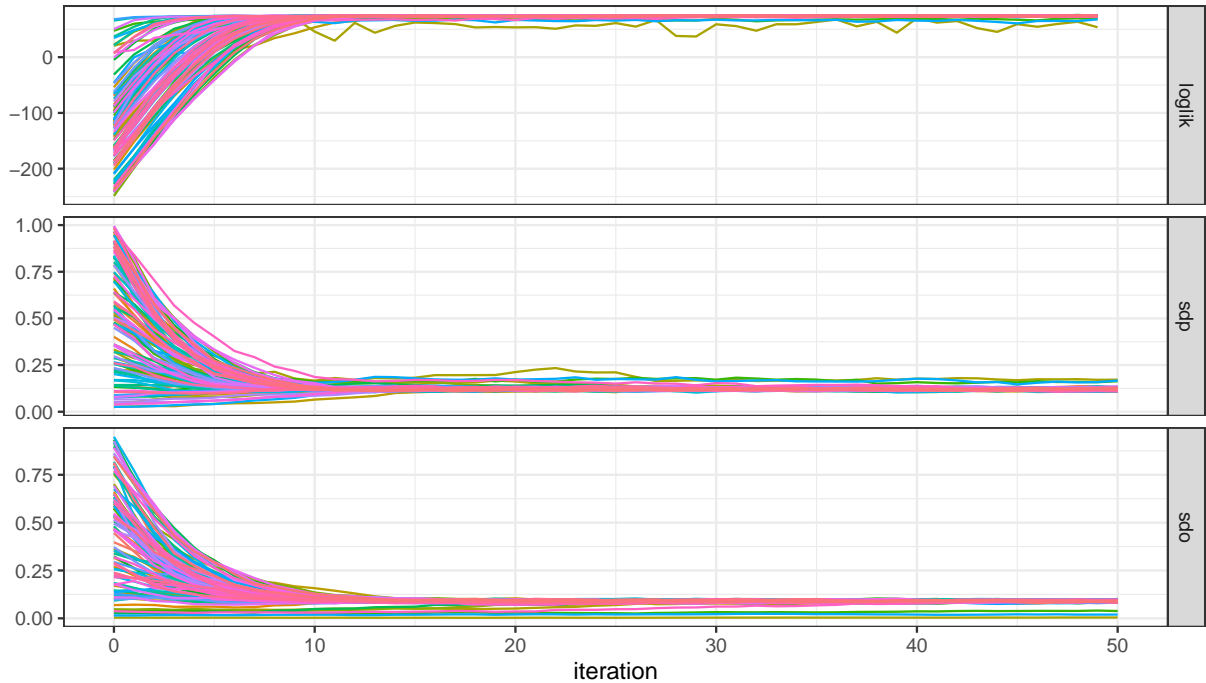

Figure S1.28: Diagnostic plots for the many parallel mif2 computations.

We can see here that the log likelihood of the perturbed models increased with iterations for all starting values. In this case, despite starting at values relatively far from the true values, the parameters estimates of almost all runs end up relatively close to the true values after 50 iterations.

To be able to choose the best set of parameters, we want to compare the likelihood of the different `mif2` runs. We want to do this using the likelihood of the model of interest, not the likelihood of the perturbed model. As such we run the particle filter multiple times on the results of each `mif2` run.

```
foreach (
  mf=fg2pPomp,
  .combine=rbind, .packages=c("pomp"),
  .errorhandling="remove", .inorder=FALSE
) %dopar% {
  replicate(
    10,
    mf %>% pfilter() %>% logLik()
  ) %>%
    logmeanexp(se=TRUE) -> ll

  data.frame(as.list(coef(mf)), loglik=ll[1], loglik.se=ll[2])
}
```

```
} -> pares2pPomp
```

To get a maximum likelihood estimate, we find the values associated with the highest log-likelihood values.

```
cbind(
  Estimated=c(pares2pPomp[which.max(pares2pPomp$loglik),]),
  True=c(coef(pfs0pPomp[[1]]),loglik=logmeanexp(logLik(pfs0pPomp),se=TRUE))
)
```

| ##           | Estimated  | True     |
|--------------|------------|----------|
| ## sdp       | 0.1224633  | 0.1      |
| ## sdo       | 0.08911649 | 0.1      |
| ## loglik    | 74.71701   | 73.11801 |
| ## loglik.se | 0.1414779  | 0.261995 |

Note that the likelihood at the MLE is significantly higher than that at the truth, as expected. Model comparison and validation should also be performed when fitting models with `pomp` and tools described in other sections could be implemented here. Functions such as `probe` may be particularly helpful in this connection. For more information on `pomp`, see King et al. (2020) and <http://kingaa.github.io/pomp/>.

## S1 1.3.5 JAGS

JAGS, which stands for Just Another Gibbs Sampler, is an MCMC package which is primarily aimed at carrying out Bayesian analyses (see main text). The R package `rjags` can be used as a front end to JAGS. While `rjags` can be installed from CRAN, to be able to use the package, one needs to install JAGS first. You can find information on JAGS here: <http://mcmc-jags.sourceforge.net/>. You can download JAGS from here: <https://sourceforge.net/projects/mcmc-jags/files/>

Here, we demonstrate fitting our simplified model (Eqs. 1.3-1.4), namely, estimating the unknown states,  $z_t$ ,  $t=1, \dots, T$ , two different ways. First, we will assume that the standard deviations of process variation and observation error (`sdp` and `sdo`) are known (and the true values are used). Second, we will explore estimating the states and those standard deviations. In both cases the initial state,  $z_0$ , is treated as a known value and is set equal to the true value of 0.

### S1 1.3.5.1 Using `rjags` to estimate the states when the parameters are known

First, let us load `rjags`.

```
library(rjags)
```



Input to the JAGS program includes: a) the model description, b) the data (observations and sometimes hyperparameter values for prior distributions), and c) initial values of the parameters or random effects for the Markov chains that will be generated, which are optional. With SSMS the model description includes the process and observation equations, as well as prior distributions for unknown parameters.

Let us start with defining the model. Just as for TMB, the model in JAGS are written in a different language than the R language, specifically, JAGS use the BUGS language. With `rjags` it can be either written in a separate file or as a string. Here we demonstrate the later.

```
toyOpJags <- "
  model {

    #### Transforming sd into precision
    state.precision <- 1/(sdp*sdp)
    obs.precision   <- 1/(sdo*sdo)

    ### Process equation
    # 1st time step (based on known z0)
    z[1] ~ dnorm(z0,state.precision)
    # Remaining time steps
    for(t in 2:TT) {
      z[t] ~ dnorm(z[t-1],state.precision)
    }

    ### Observation equation
    for(t in 1:TT) {
      y[t] ~ dnorm(z[t],obs.precision)
      # Calculate the pointwise log-likelihoods
      # Needed for waic and loo
      loglik[t] <- logdensity.norm(y[t],z[t],obs.precision)
    }
  }
"
```

A few things to note. Here, because we fix all parameters to their known values, we have no priors. However, we do transform our standard deviations into precision  $\frac{1}{\sigma^2}$  as in the BUGS language the normal distribution functions (e.g., `dnorm`) use precision rather than standard deviation. In addition, we added the observation equation a line that calculates the pointwise log likelihood. These can be used to calculate the conditional log likelihood and are needed to calculate WAIC with the package `loo` (see below).

Now we can define the data. All of the objects used in the model that are not defined explicitly in the model description need to be listed as data. Thus here, we need: `sdp`, `sdo`, `z0`, `TT`, and `y`. This has to be defined in a list.

```
data0pJags <- list(TT=TT, y=y, sdp=sdp, sdo=sdo, z0=0)
```

Multiple chains are useful for diagnostics on the performance of the MCMC sampler, e.g., detecting how sensitive posterior distributions are to initial values. Here, we will use three chains. The next step, is to define the initial values for each chain. There are three sets of initial values from which JAGS will then create three separate sets of Markov chains.

```
nc0pJags <- 3
initval0pJags <- list()
for(i in 1:nc0pJags) {
  zinit <- numeric(TT)
  zinit[1] <- rnorm(1, mean=0, sd=sdp)
  for(t in 2:TT) {
    zinit[t] <- rnorm(1, mean=zinit[t-1], sd=sdp)
  }
  initval0pJags[[i]] <- list(z=zinit)
}
```

With `rjags`, you need to define the length of the `burnin` period and the length of the chains after the initial burnin period. The second value represent the number of iterations that forms the samples from the posterior distributions.

```
burn0pJags <- 1000
infer0pJags <- 10000
```

The function `jags.model` sets up and “compiles” the JAGS model, loading the data and initial values. The function `update` runs the Markov chain through the burnin period.

```
m0pJags <- jags.model(file=textConnection(object=toy0pJags),
                      data=data0pJags,
                      inits=initval0pJags,
                      n.chains=nc0pJags)

## Compiling model graph
##   Resolving undeclared variables
##   Allocating nodes
## Graph information:
##   Observed stochastic nodes: 200
##   Unobserved stochastic nodes: 200
##   Total graph size: 607
##
## Initializing model
```

```
update(m0pJags, n.iter=burn0pJags)
```

The function `coda.samples` continues the chain for the inference length. Here, we need to specify the variables to monitor. Here, we primarily want to monitor the states. However, to be able to calculate WAIC, we also want to monitor the pointwise log-likelihoods.

```
jagsp0VarM <- c("z", "loglik")
f0pJags <- coda.samples(m0pJags,
                        variable.names=jagsp0VarM,
                        n.iter=infer0pJags)
```

The output from JAGS is a `mcmc.list`, where each element is one of the chains.

```
f0pJags[[1]][1:3,1:5]

##      loglik[1] loglik[2] loglik[3] loglik[4] loglik[5]
## [1,]  1.320344  1.114548 -0.3644327  1.226761  1.3836323
## [2,]  1.260297  1.383372 -0.1536632  1.281275  1.1435989
## [3,]  1.359733  1.281672  0.8815791  1.315995  0.9984412
```

The output from each chain can be easily converted to a matrix with the row entries corresponding to chain iterations and columns being the variables specified in the `variable.names` argument to `coda.samples`. We can use these matrices to get at the state estimates, for example by taking the mean. To extract just the states and not the pointwise log likelihoods, we can use the following code.

```
zs0pJags <- apply(as.matrix(f0pJags)[,paste0("z[",1:TT,")"]],2,mean)
head(zs0pJags)

##      z[1]      z[2]      z[3]      z[4]      z[5]      z[6]
## 0.002297183 0.003104805 0.029311226 -0.030061753 -0.037337317 -0.060322730
```

One could also use the summary function. For example, the element `statistics` returned by the `summary` function contains the posterior mean, as well as the standard error and other useful information. The element `quantiles` contains the quantiles of the posterior distribution, which can be quite useful to create 95% credible intervals.

```
zsv0pJags <- summary(f0pJags[,paste0("z[",1:TT,")"],])
head(zsv0pJags$statistics)
```

```
##           Mean      SD      Naive SE Time-series SE
## z[1]  0.002297183 0.06232439 0.0003598300  0.0004126610
## z[2]  0.003104805 0.06638498 0.0003832739  0.0004984688
## z[3]  0.029311226 0.06636411 0.0003831534  0.0005190290
## z[4] -0.030061753 0.06669536 0.0003850658  0.0005182878
## z[5] -0.037337317 0.06617053 0.0003820357  0.0005054911
## z[6] -0.060322730 0.06693742 0.0003864634  0.0005134204
```

```
head(zsv0pJags$quantiles)
```

```
##           2.5%      25%      50%      75%      97.5%
## z[1] -0.1206533 -0.04030920 0.002230491 0.044652655 0.12483856
## z[2] -0.1264725 -0.04143313 0.002877332 0.047931968 0.13334271
## z[3] -0.1015656 -0.01535747 0.029396816 0.073845475 0.15987269
## z[4] -0.1593505 -0.07513194 -0.030159207 0.014283566 0.10174578
## z[5] -0.1673018 -0.08198890 -0.037437636 0.007401938 0.09226354
## z[6] -0.1901433 -0.10577587 -0.060016542 -0.014995174 0.07038402
```

We can now plot the estimates on top of the simulations.

```
plot(1:TT, y,
     pch=3, cex = 0.8, col="blue", ty="o", lty = 3,
     xlab = "t", ylab = expression(z[t]),
     xlim = c(0,TT), ylim = c(min(y), max(y)+max(y)/5),
     las = 1)
points(0:TT, z,
       pch = 19, cex = 0.7, col = "red", ty = "o")
lines(1:TT, zs0pJags,
      col="darkgoldenrod1", lwd = 2)
legend("top",
      legend = c("Obs.", "True states", "Smooth. states"),
      pch = c(3, 19, NA),
      col = c("blue", "red", "darkgoldenrod1"),
      lwd = c(1, 1, 2), lty = c(3, 1, 1),
      horiz=TRUE, bty="n", cex=0.9)
```

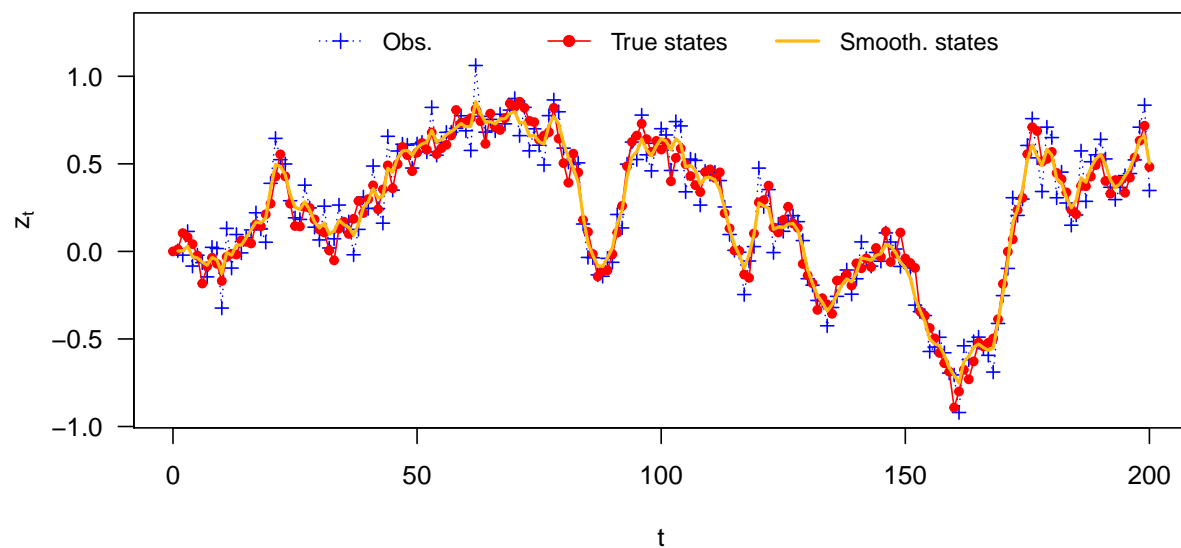

Figure S1.29: Estimated states with JAGS for the toy model with known parameter values.

#### S1 1.3.5.2 Using rjags to estimate the states and the parameters

Now, we can reproduce the same procedure but for the case where we want to estimate the states and the standard deviations of the process variation and observation error.

Let us start with the model.

```
toy2pJags <- "
  model {

    ### Priors
    sdp ~ dunif(sdp.hyper.a,sdp.hyper.b)
    sdo ~ dunif(sdo.hyper.a,sdo.hyper.b)
    # Transform sd in precision
    state.precision <- 1/(sdp*sdp)
    obs.precision   <- 1/(sdo*sdo)

    ### Process equation
    # 1st time step (based on known z0)
```

```

z[1] ~ dnorm(z0,state.precision)
# Remaining time steps
for(t in 2:TT) {
  z[t] ~ dnorm(z[t-1],state.precision)
}

### Observation equation
for(t in 1:TT) {
  y[t] ~ dnorm(z[t],obs.precision)
  # Calculate the pointwise log-likelihoods
  # Needed for waic and loo
  loglik[t] <- logdensity.norm(y[t],z[t],obs.precision)
}
}
"

```

Now let us set up the data. We now need to define hyperparameters for the priors. As defined in the model above, we are using uniform distribution. We will set the range of the uniform to go from 0.01 to 10 (remember the true values are 0.1). Note that the use of uniform priors is not necessarily optimal in this situation, but we use it here as a simple example.

```

data2pJags <- list(TT=TT, y=y,
  sdp.hyper.a=0.01, sdp.hyper.b=10,
  sdo.hyper.a=0.01, sdo.hyper.b=10,
  z0=0)

```

Again we will run three chains and initialize them.

```

nc2pJags <- 3
initval2pJags <- list()
for(i in 1:nc2pJags) {
  sdpinit <- runif(1, min=data2pJags$sdp.hyper.a,
    max=data2pJags$sdp.hyper.b)
  sdoinit <- runif(1, min=data2pJags$sdo.hyper.a,
    max=data2pJags$sdo.hyper.b)
  zinit <- numeric(TT)
  zinit[1] <- rnorm(1,mean=0,sd=sdpinit)
  for(t in 2:TT) {
    zinit[t] <-rnorm(1,mean=zinit[t-1],sd=sdpinit)
  }
  initval2pJags[[i]] <- list(sdp=sdpinit,sdo=sdoinit,z=zinit)
}

```

We will use the same burnin period and the same inference chain length.

```
burn2pJags <- 1000
infer2pJags <- 10000
```

Finally, we will use the same functions to run the models.

```
m2pJags <- jags.model(file=textConnection(object=toy2pJags),
                      data=data2pJags,
                      inits=initval2pJags,
                      n.chains=nc2pJags)

## Compiling model graph
##   Resolving undeclared variables
##   Allocating nodes
## Graph information:
##   Observed stochastic nodes: 200
##   Unobserved stochastic nodes: 202
##   Total graph size: 613
##
## Initializing model

update(m2pJags, n.iter=burn2pJags)
```

One of the only difference is that now that we are estimates the standard deviations, we are going to monitor these variables.

```
jagsp2VarM <- c("sdp", "sdo", "z", "loglik")
f2pJags <- coda.samples(m2pJags,
                       variable.names=jagsp2VarM,
                       n.iter=infer2pJags)
```

We can now extract the state estimates from the summary function.

```
zsv2pJags <- summary(f2pJags[,paste0("z[",1:TT,"]"),])
head(zsv2pJags$statistics)

##              Mean          SD      Naive SE Time-series SE
## z[1]  0.003017880 0.06356185 0.0003669745   0.0003982883
```

```
## z[2]  0.002556867 0.06597029 0.0003808796 0.0004499947
## z[3]  0.046268371 0.06722152 0.0003881036 0.0005316287
## z[4] -0.038417826 0.06618044 0.0003820929 0.0004651608
## z[5] -0.036385583 0.06635460 0.0003830985 0.0004632774
## z[6] -0.063622371 0.06687153 0.0003860830 0.0004655098
```

```
zs2pJags <- zsv2pJags$statistics[, "Mean"]
```

We can now visually compare the state estimates to the one obtained when we used the known parameter values.

```
plot(1:TT, y,
     pch=3, cex = 0.8, col="blue", ty="o", lty = 3,
     xlab = "t", ylab = expression(z[t]),
     xlim = c(0,TT), ylim = c(min(y), max(y)+max(y)/5),
     las = 1)
points(0:TT, z,
       pch = 19, cex = 0.7, col = "red", ty = "o")
lines(1:TT, zs0pJags,
      col="darkgoldenrod1", lwd = 2)
lines(1:TT, zs2pJags,
      col="cyan3", lty = 5, lwd=3)
legend("top",
      legend = c("Obs.", "Tr. stat.",
                  "Es. stat. (kn. par.)", "Es. stat. (es. par.)"),
      pch = c(3, 19, NA, NA),
      col = c("blue", "red", "darkgoldenrod1", "cyan3"),
      lwd = c(1, 1, 2, 3), lty = c(3, 1, 1, 5),
      horiz=TRUE, bty="n", cex=0.9)
```



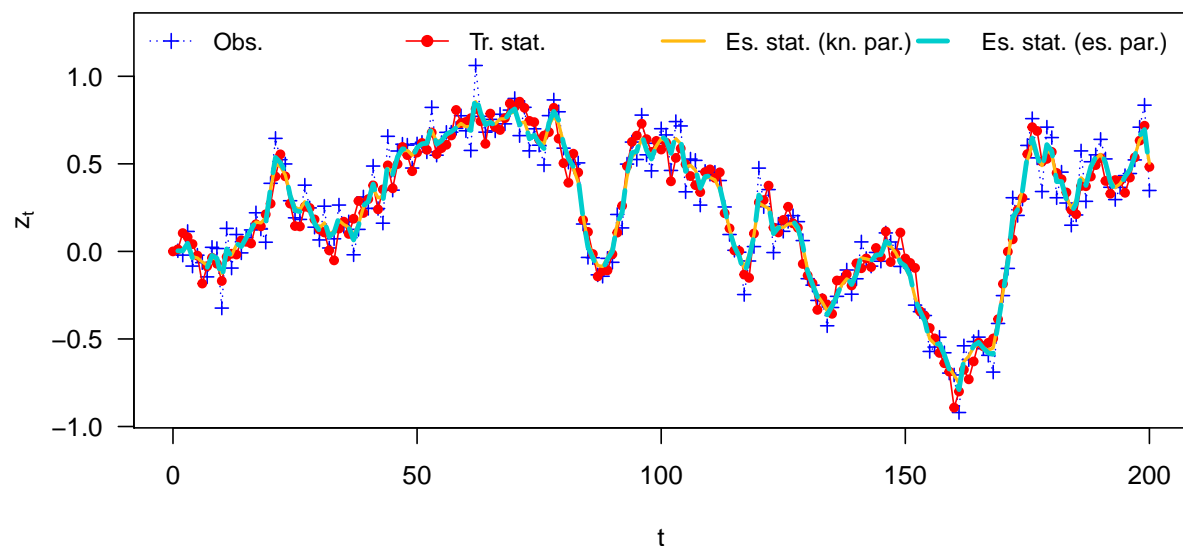

Figure S1.30: Estimated states with JAGS for the toy model with known and estimated parameter values.

The results are quite similar, which is not surprising since the parameter estimates are quite good.

```
summary(f2pJags[,c("sdp", "sdo"),])$statistic
```

| ##     | Mean       | SD         | Naive SE     | Time-series SE |
|--------|------------|------------|--------------|----------------|
| ## sdp | 0.12116490 | 0.01281980 | 7.401513e-05 | 0.0003324358   |
| ## sdo | 0.08945533 | 0.01164509 | 6.723297e-05 | 0.0003230687   |

The object returned by `coda.samples`, here `f2pJags`, will contain all of the values monitored. For this model, the pointwise log likelihoods and the posterior samples of the states and the two parameters. We can extract the posterior from the parameters as follow.

```
postSdp2pJags <- f2pJags[, "sdp", ]
postSdo2pJags <- f2pJags[, "sdo", ]
```

We can use these to plot the trace plot and the posterior density. Let us do this for the standard deviation of the process equation first.

```
plot(postSdp2pJags)
```

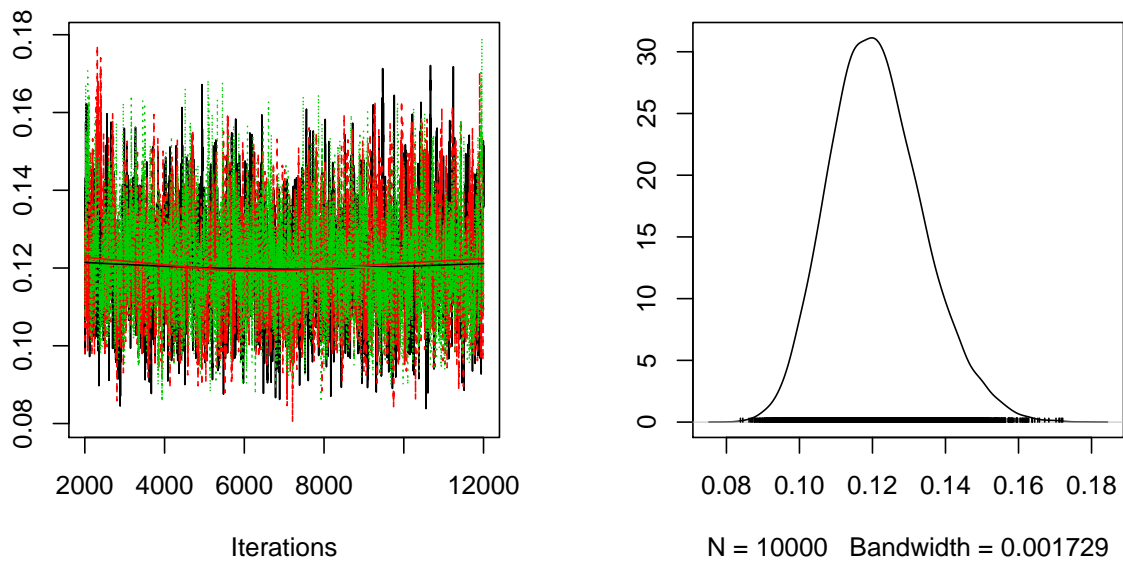

Figure S1.31: Trace plot and density distribution of the samples from  $sdp$ .

The chains, represented by each color on the trace plot, look relatively well mixed. The peak of the posterior is close to the true value of 0.1.

Now, let us do it for the observation error.

```
plot(postSdo2pJags)
```

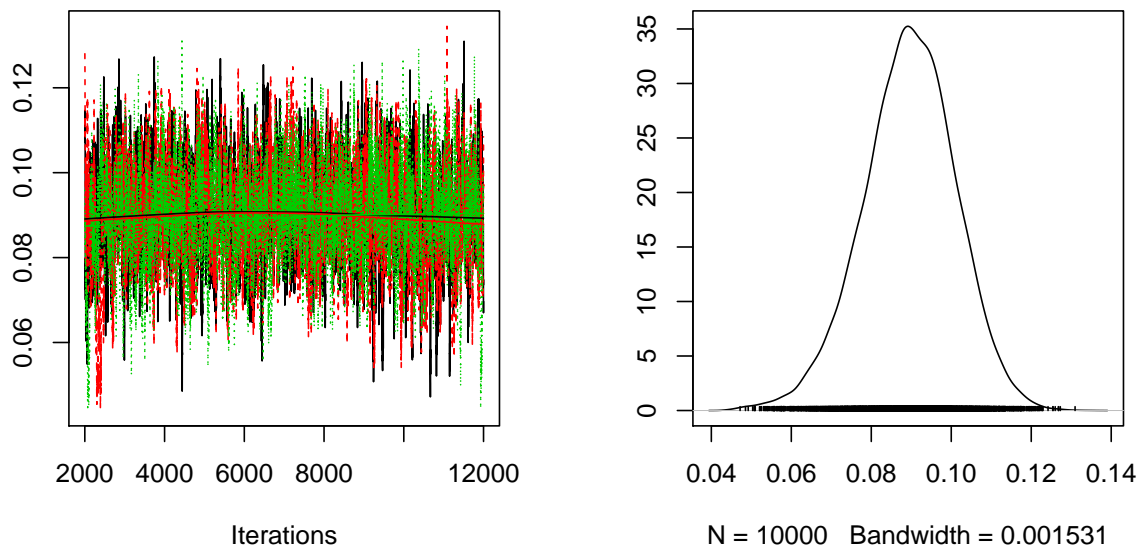

Figure S1.32: Trace plot and density distribution of the samples from sdo.

To look at the convergence, we can also look at the Gelman-Rubin metric using the function `gelman.diag`. We can do it for all variables (e.g., `gelman.diag(f2pJags)`) or for specific variable as follow.

```
gelman.diag(postSdp2pJags)

## Potential scale reduction factors:
##
##      Point est. Upper C.I.
## [1,]          1          1
```

All values are below the 1.1 threshold, indicating that the chains have likely converged.

We can use the package `loo` to calculate WAIC. Note however the `waic` function returns is based on the conditional, not the marginal, likelihood.

```
library(loo)
```

As mentioned above we are monitoring the pointwise log likelihoods, which we will use as main input in the function `waic`. However, to be able to input the results from `coda.samples` in `waic` we need to change the output into an array of the good dimension (i.e., an I by C by N array, where I is the number of iterations, C is the number of chains, N is the number of observations - see `?waic` for other options).

```

# Transforming the mcmc.list into an array
# m0p
pll0pJags <- as.array(f0pJags[,paste0("loglik[",1:TT,"]"),])
# m2p
pll2pJags <- as.array(f2pJags[,paste0("loglik[",1:TT,"]"),])

# Transposing the arrays
pll0pJags <- aperm(pll0pJags, c(1,3,2))
dim(pll0pJags)

## [1] 10000      3    200

pll2pJags <- aperm(pll2pJags, c(1,3,2))
dim(pll2pJags)

## [1] 10000      3    200

```

Now we can use the function `waic` to calculate the WAIC of each model and we can use the function `loo_compare` to compare the two models.

```

waic0pJags <- waic(pll0pJags)

## Warning:
## 54 (27.0%) p_waic estimates greater than 0.4. We recommend trying loo instead.

waic2pJags <- waic(pll2pJags)

## Warning:
## 63 (31.5%) p_waic estimates greater than 0.4. We recommend trying loo instead.

loo_compare(waic0pJags, waic2pJags)

##           elpd_diff se_diff
## model2      0.0         0.0
## model1 -15.1         1.4

```

It looks like the more flexible model (with the estimated standard deviations estimated) is better according to WAIC, which is somewhat surprising in this case. This could be an artifact that this WAIC is based on the conditional likelihood and there are two warnings indicating that results are likely unreliable. In

this case, it may be to our advantage to use the function `loo` to calculate the approximate leave-one-out cross-validation or to perform actual cross-validation. See the extensive vignettes from the `loo` packages for details. One could also calculate the marginal WAIC, see <http://semtools.r-forge.r-project.org/> for an example.

### S1 1.3.6 nimble

In this section, we are demonstrating how to fit the toy example with the R package `nimble`. This package allows to fit models using Bayesian methods and is an alternative to JAGS, where the user can more easily control the sampling algorithms.

`nimble` is available through CRAN, but just like TMB, it requires the installation of a C++ compiler. For detailed installation information (including troubleshooting tips), see [https://r-nimble.org/html\\_manual/cha-installing-nimble.html](https://r-nimble.org/html_manual/cha-installing-nimble.html).

Once installed, let us load `nimble`.

```
library(nimble)

## nimble version 0.10.1 is loaded.
## For more information on NIMBLE and a User Manual,
## please visit http://R-nimble.org.

##
## Attaching package: 'nimble'

## The following object is masked from 'package:stats':
##
## simulate
```

Type `library(help="nimble")` to get more information about the R package. A full user manual is available at <https://r-nimble.org>.

The steps to set up `nimble` are very similar to those for JAGS. First, we define the model. Second, we create a data object. Third, we specify initial values for the parameters. Fourth, we specify constants. These constants can be viewed as fixed parameter values or data used only to set up the model (e.g., length of time series). Then, as we show below, we have multiple additional steps that define the sampling algorithm.

#### Step 1: define the model

We use the function `nimbleCode()` to define the model. The model syntax is very similar to the BUGS language used by JAGS.

```
toy2pNimble <- nimbleCode({
  sdp ~ dunif(1e-04, 1)
  sdo ~ dunif(1e-04, 1)
  z[1] ~ dnorm(z0, sd=sdp)
  y[1] ~ dnorm(z[1], sd=sdo)
  for (i in 2:TT) {
    z[i] ~ dnorm(z[i - 1], sd = sdp)
    y[i] ~ dnorm(z[i], sd=sdo)
  }
})
```

## Step 2: define the data

```
dataNimble <- list(y = y)
```

## Step 3: define the initial values

```
init2pNimble <- list(
  sdp = sdp,
  sdo = sdo
)
```

## Step 4: define the constants

```
const2pNimble <- list(
  TT = TT,
  z0 = 0
)
```

## Step 5: create the nimble model object

Then, we create a nimble model called `m2pNimble`, which contains results from Steps 1-4 and thus contains all of the basic information to fit the model.

```
m2pNimble <- nimbleModel(toy2pNimble,
  data = dataNimble,
  constants = const2pNimble,
  inits = init2pNimble,
  check = FALSE)
```

```
## defining model...
## building model...
## setting data and initial values...
## running calculate on model (any error reports that follow may simply reflect
missing values in model variables) ...
## checking model sizes and dimensions... This model is not fully initialized.
This is not an error. To see which variables are not initialized, use model$initialize
For more information on model initialization, see help(modelInitialization).
## model building finished.
```

#### Step 6: compile the nimble model object

We then compile the results from the `nimbleModel` results. The function `compileNimble` generates C++ code, loads the compiled model, and returns an interface object.

```
comp2pNimble <- compileNimble(m2pNimble)

## compiling... this may take a minute. Use 'showCompilerOutput = TRUE' to see
C++ compilation details.

## compilation finished.
```

#### Step 7: configure MCMC sampler

This step configures the MCMC sampler. One option, shown below, is to use the function `configureMCM` to find the default samplers to be used for the variables of interest.

```
conf2pNimble <- configureMCMC(m2pNimble, print=FALSE)
```

If we set `print=TRUE`, the default samplers chosen for each random variables will be printed. In this case, 202 lines would be the output, showing that random walks would be used by default for the process and observation standard deviations, while conjugate normal samplers would be used for the states.

While here we use the default samplers, there are many options for the type of MCMC sampling that could be done and this is one area where `nimble` stands out from `BUGS` and `JAGS`. See the help file on the class `MCMCconf` for more information on how to change the samplers.

#### Step 8: Specify the variables to monitor

We then specify which variables should be monitored and kept for printing, plotting, etc. Here, we will monitor both standard deviations and all the 200 state values.

```
conf2pNimble$addMonitors(c("sdp", "sdo", "z"))

## thin = 1: sdp, sdo, z
```

### Step 9: Build and compile the MCMC function

Now, based on our model and algorithm, we build an MCMC function, that we then compile.

```
mcmc2pNimble <- buildMCMC(conf2pNimble)
mcmcc2pNimble <- compileNimble(mcmc2pNimble,
                               project=m2pNimble,
                               resetFunctions=TRUE)

## compiling... this may take a minute. Use 'showCompilerOutput = TRUE' to see
C++ compilation details.

## compilation finished.
```

### Step 10: run the MCMC algorithm

Finally, we can run one or more chains of an MCMC algorithm and get samples of our posterior distribution. Here will run 2 chains with 60,000 iterations that will have a burn-in of 10,000 and then the next 50,000 iterations yield the samples for inference.

This may take a few minutes to run.

```
set.seed(231)
f2pNimble <- runMCMC(mcmcc2pNimble,
                    nburnin=10000,
                    nchains=2,
                    niter=60000)

## running chain 1...

## |-----|-----|-----|-----|
## |-----|-----|-----|-----|

## running chain 2...

## |-----|-----|-----|-----|
## |-----|-----|-----|-----|
```



The output is stored as list with an element for each chain. For each chain, we have a matrix with number of rows = `niter - nburnin` and number of columns = the number of parameters/variables specified in the `addMonitors` field above. For example, here are the first few rows and columns of chain 1.

```
f2pNimble$chain1[1:3,1:6]
```

| ## |      | sdo      | sdp        | z[1]        | z[2]        | z[3]        | z[4]        |
|----|------|----------|------------|-------------|-------------|-------------|-------------|
| ## | [1,] | 0.109201 | 0.10031746 | -0.03764566 | 0.02961975  | 0.04397682  | -0.03585785 |
| ## | [2,] | 0.109201 | 0.09732752 | -0.07690303 | -0.03154761 | -0.06116048 | -0.05120515 |
| ## | [3,] | 0.109201 | 0.09732752 | 0.03804806  | -0.06444083 | 0.03770490  | -0.03665527 |

### Step 11: examine the results

As for JAGS, it is good to look at the trace plots. Here, let us look at the trace plots of the two standard deviations.

```
plot(f2pNimble$chain1[ , "sdp"], type = "l", xlab = "iteration",
     ylab = expression(sigma[p]), col="hotpink", las=1)
lines(f2pNimble$chain2[ , "sdp"], col="purple")
plot(f2pNimble$chain1[ , "sdo"], type = "l", xlab = "iteration",
     ylab = expression(sigma[o]), col="hotpink", las=1)
lines(f2pNimble$chain2[ , "sdo"], col="purple")
```

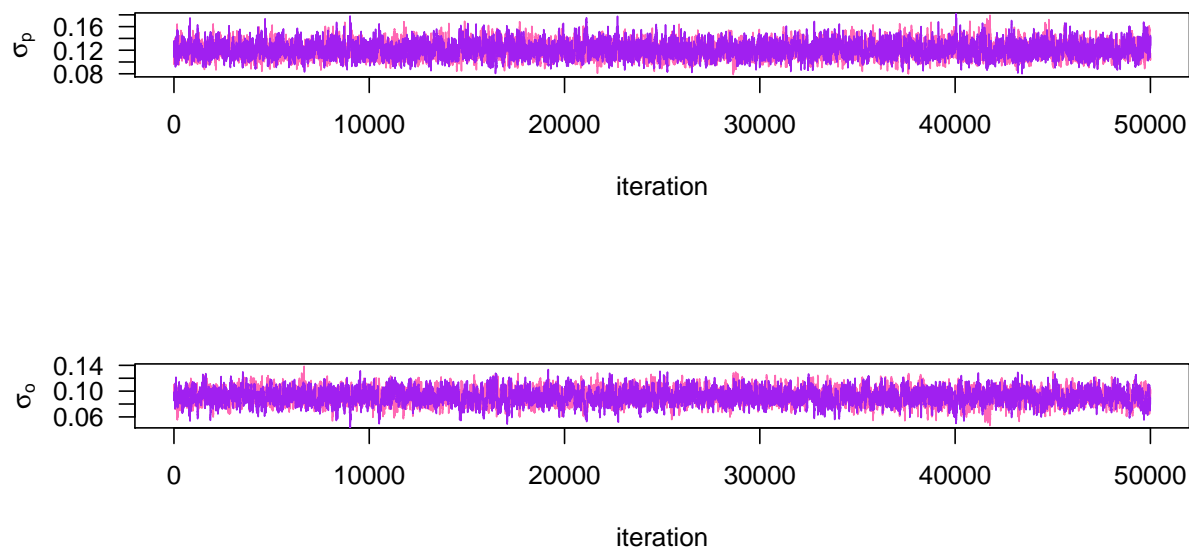

Figure S1.33: Trace plots of standard deviations samples from nimble

The chains look well mixed.

We can now calculate the smoothed states.

```
zsp2pNimble <- rbind(f2pNimble$chain1[,3:(TT+2)],
                     f2pNimble$chain2[,3:(TT+2)])
zs2pNimble <- apply(zsp2pNimble,2,mean)
head(zs2pNimble)
```

| ## | z[1]        | z[2]        | z[3]        | z[4]         | z[5]         | z[6]         |
|----|-------------|-------------|-------------|--------------|--------------|--------------|
| ## | 0.002197514 | 0.001808551 | 0.044561823 | -0.037923039 | -0.036845080 | -0.064372071 |

We can plot the estimated states on alongside true states.

```
plot(1:TT, y,
     pch=3, cex = 0.8, col="blue", ty="o", lty = 3,
     xlab = "t", ylab = expression(z[t]),
     xlim = c(0,TT), ylim = c(min(y), max(y)+max(y)/5),
     las = 1)
```

```

points(0:TT, z,
      pch = 19, cex = 0.7, col = "red", ty = "o")
lines(1:TT, zs2pNimble,
      col="darkgoldenrod1", lwd = 2)
legend("top",
      legend = c("Obs.", "True states",
                  "Est. states"),
      pch = c(3, 19, NA),
      col = c("blue", "red", "darkgoldenrod1"),
      lwd = c(1, 1, 2), lty = c(3, 1, 1),
      horiz=TRUE, bty="n", cex=0.9)

```

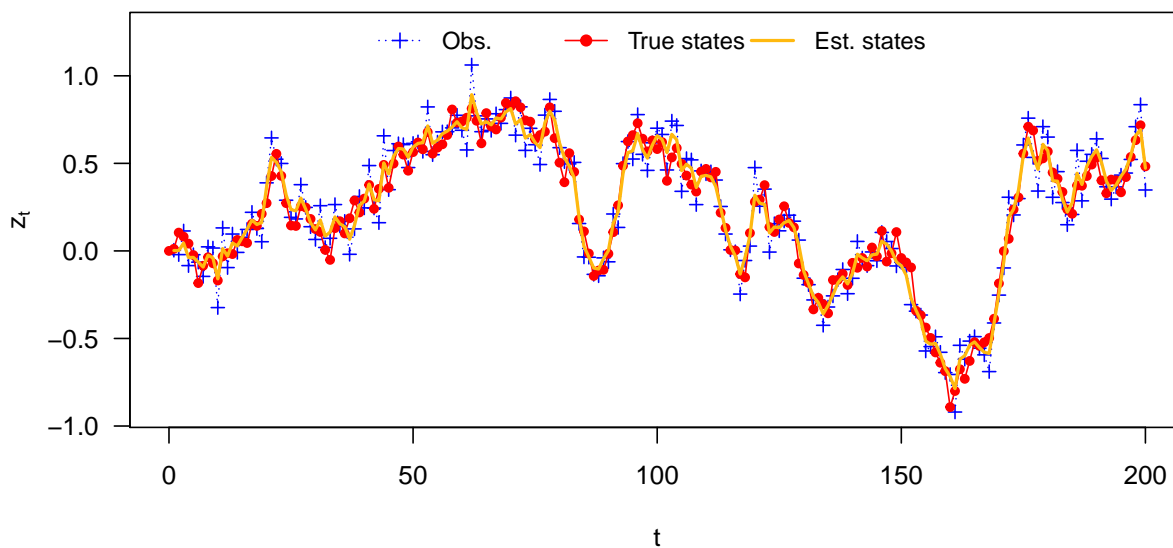

Figure S1.34: Comparison of the estimated states with nimble with the true simulated values.

Nimble does not include any MCMC diagnostics, such as `gelman.diag`, but the package `coda` can be applied to Nimble samples. As previously noted, we can apply the Gelman-Rubin metric to all of the variables or a specific variables as follows. To be able to use the functions from the package `coda`, we need to use the function `covert.mcmc.list` from the package `mcmcplots`.

```

# Convert nimble samples to mcmc
library(mcmcplots)
fcoda2pNimble <- convert.mcmc.list(f2pNimble)
# Gelman-Rubin metric using coda package gelman.diag
head(gelman.diag(fcoda2pNimble)$psrf)

##      Point est. Upper C.I.
## sdo  1.0006842  1.0014309
## sdp  1.0008434  1.0025035
## z[1] 1.0001077  1.0001087
## z[2] 0.9999809  0.9999824
## z[3] 0.9999869  0.9999882
## z[4] 0.9999914  1.0000002

gelman.diag(fcoda2pNimble)$mpsrf

## [1] 1.005536

```

All values are below the 1.1 threshold. Thus, it looks like the chains have likely converged.

## S1 1.3.7 Stan

**Stan** is a probabilistic programming language commonly used to conduct Bayesian inference (Stan Development Team, 2012). It implements a dynamic Hamiltonian Monte Carlo (HMC) algorithm that can be used to draw samples directly from a joint posterior distribution of interest. As mentioned in the main text, HMC can be implemented as long as all parameters are continuous, either by construction or by marginalization of the joint posterior distribution over the discrete parameters. As we will demonstrate below, **Stan** can be called through R using the package **rstan**. **rstan** is available through CRAN. While **rstan** is an interface to **Stan**, you do not need to separately install **Stan**, see [https://mc-stan.org/docs/2\\_18/stan-users-guide/some-differences-when-running-from-r.html](https://mc-stan.org/docs/2_18/stan-users-guide/some-differences-when-running-from-r.html). However, you need to check your C++ toolchain, see <https://github.com/stan-dev/rstan/wiki/RStan-Getting-Started> for more info.

For more information, interested readers should also look at these two links: <https://github.com/stan-dev/rstan/wiki/RStan-Getting-Started>, and <https://github.com/stan-dev/stan/wiki/Stan-Best-Practices>.

Let us first load **rstan** and set up options so it runs processes in parallel and does not recompile unchanged programs.

```

library(rstan)
# To run in parallel on multiple cores
options(mc.cores=parallel::detectCores())
# To avoid recompiling unchanged Stan program

```

```
rstan_options(auto_write=TRUE)
```

As for many other packages we have investigated above, we need to write the model in a different language. Here, to write the model using the Stan language, we define *blocks* of interest. A basic model can have three blocks: *data*, *parameters* and *model*. As for TMB, the model information is saved in a separate file with a .stan extension. Here, we will save the following in a file called *toy2p.stan*. Note: be sure that your Stan program ends with a blank line and do not use tabs - use two spaces instead.

```
/*----- Data -----*/
/* Data block: defines the objects that will be inputted as data */
data {
  int TT; // Length of state and observation time series
  vector[TT] y; // Observations
  real z0; // Initial state value
}

/*----- Parameters -----*/
/* Parameter block: defines the variables that will be sampled */
parameters {
  real<lower=0> sdp; // Standard deviation of the process equation
  real<lower=0> sdo; // Standard deviation of the observation equation
  vector[TT] z; // State time series
}

/*----- Model -----*/
/* Model block: defines the model */
model {
  // Prior distributions
  sdo ~ normal(0, 1);
  sdp ~ normal(0, 1);

  // Distribution for the first state
  z[1] ~ normal(z0, sdp);

  // Distributions for all other states
  for(t in 2:TT){
    z[t] ~ normal(z[t-1], sdp);
  }

  // Distributions for the observations
  for(t in 1:TT){
```

```

    y[t] ~ normal(z[t], sdo);
  }
}

```

The data block indicates the length of the time series, `TT`, defined as an integer with a minimum value of 1 and the data, `y`, is in a vector of length `TT`. The generic vector type allows for `y` to contain any values defined on  $\mathbb{R}$ .

The next block defines all the parameters of interest. In this example, we would like to estimate the standard deviation of the process variation and the observation error. The two standard deviations are defined over the interval  $(0, \infty)$ . In **Stan**, this is defined as `real<lower=0>`. We also define the latent states as parameters of interest.

The next block defines the model. The model block defines first prior distributions for the observation and process error. Note that here we use normal priors. Then, it defines the data generating model. Although we define the latent states ‘`z`’ as parameters, we do not specify a prior distribution as they are completely specified by their distributional form and the process model.

The joint posterior defined in **Stan** is,

$$p(\sigma_o, \sigma_p, \mathbf{z} | \mathbf{y}, z_0) \propto \mathbf{g}(\mathbf{y} | \mathbf{z}, \sigma_o) \mathbf{f}(\mathbf{z} | \sigma_p, z_0) h(\sigma_o) h(\sigma_p), \quad (1.17)$$

where, with a slight abuse of notation:

$$\mathbf{g}(\mathbf{y} | \mathbf{z}, \sigma_o) = \prod_{t=1}^T g(y_t | z_t, \sigma_o), \quad (1.18)$$

$$\mathbf{f}(\mathbf{z} | \sigma_p, z_0) = \prod_{t=2}^T f(z_t | z_{t-1}, \sigma_p) f(z_1 | \sigma_p, z_0), \quad (1.19)$$

and  $h(\sigma_o)$  and  $h(\sigma_p)$  are the prior distributions of the two estimated parameters. Here,  $g(y_t | z_t, \sigma_o)$  and  $f(z_t | z_{t-1}, \sigma_p)$  are the observation and process equations respectively.

The estimate of the latent states, in this case, corresponds to the smoothed states, i.e.  $p(\mathbf{z} | \mathbf{y})$ . That is, it provides estimates of the distributions of the states given the entire data set, `y`.

Once the model is defined, we then set up the data. We use a `list` structure for the data, as required by the **Stan** language.

```

dataStan <- list(y=y, TT=TT, z0=0)

```

We can now call the model file to fit the model. We use the `stan` function to sample from the joint posterior distribution. We specify that **Stan** should use three chains and simulate 3000 iterations from each chain. By default, **Stan** uses half of the iterations specified for each chain for the warm-up period. In the warm-up period, the chains explore the parameter space in search of the typical set of the target distribution, estimate the gradient for use in the sampling stage and go through a period of adaptation (Betancourt, 2017). The process in the warm-up period is not always necessary in MCMC, but is always necessary for simulation via

HMC in **Stan**. As such, **Stan** eschews the term ‘burn-in’ in favor of ‘warm-up’ as this correctly describes the processes occurring before samples are drawn from the posterior distribution.

This may take a few minutes to run.

```
f2pStan <- stan(file = "toy2p.stan",  
               data = dataStan,  
               chains = 3, iter = 3000)
```

We want to look at the traceplot that includes the warmup to make sure that our warmup period is long enough.

```
# Traceplot for sdp  
traceplot(f2pStan, pars="sdp", inc_warmup = TRUE)
```

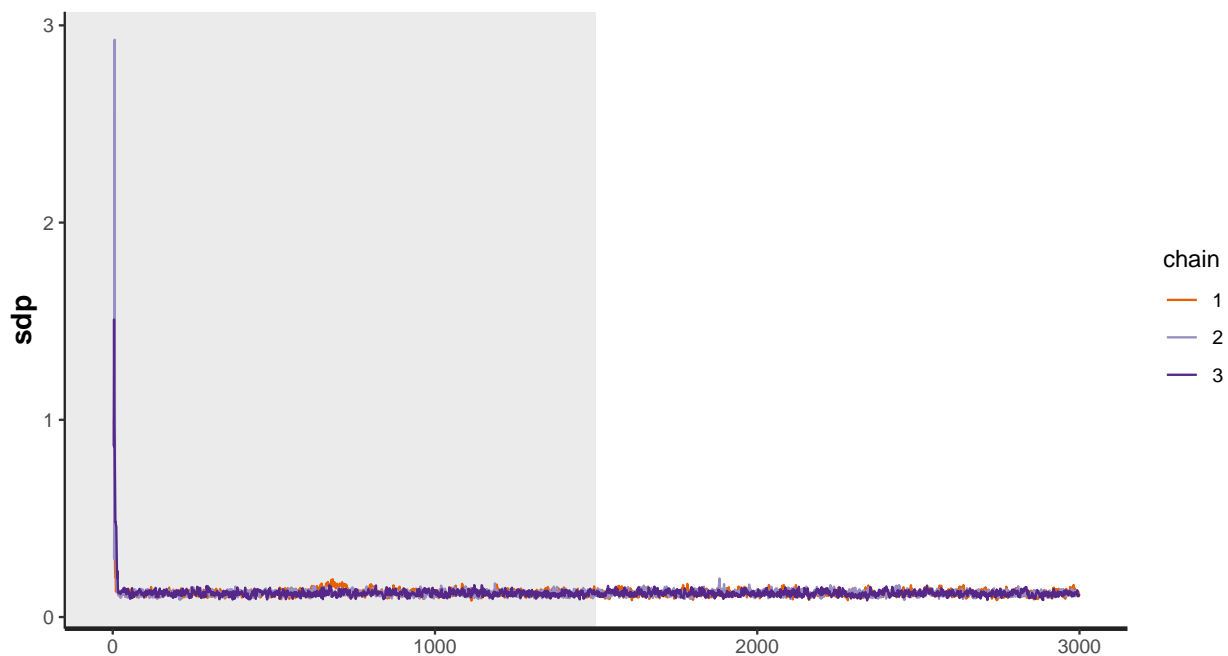

From the plot we can see that the warmup period, show in the shaded region, is more than long enough.

We can print the results from the fitted model and obtain quantiles from the marginal posterior distributions of the parameters and estimated values of  $\hat{R}$  (Gelman et al., 2013).

```
print(f2pStan, max = 50)
```

```
## Inference for Stan model: toy2p.
## 3 chains, each with iter=3000; warmup=1500; thin=1;
## post-warmup draws per chain=1500, total post-warmup draws=4500.
##
##          mean se_mean      sd   2.5%   25%   50%   75%  97.5% n_eff Rhat
## sdp      0.12     0.00  0.01   0.10   0.11   0.12   0.13   0.15   787 1.01
## sdo      0.09     0.00  0.01   0.07   0.08   0.09   0.10   0.11   598 1.01
## z[1]     0.00     0.00  0.06  -0.12  -0.04   0.00   0.04   0.13  7164 1.00
## z[2]     0.00     0.00  0.07  -0.13  -0.04   0.00   0.05   0.13  5868 1.00
## z[3]     0.04     0.00  0.07  -0.09   0.00   0.04   0.09   0.18  3659 1.00
## [ reached getOption("max.print") -- omitted 198 rows ]
##
## Samples were drawn using NUTS(diag_e) at Fri Nov  6 17:14:37 2020.
## For each parameter, n_eff is a crude measure of effective sample size,
## and Rhat is the potential scale reduction factor on split chains (at
## convergence, Rhat=1).
```

As mentioned in the main text, we would like to see that  $\hat{R} < 1.1$ , which is an indication that the chains have converged. It is also good to look at the effective sample size,  $n_{eff}$ . For  $N$  = number of posterior draws. Here, we have 3000 total posterior draws, we want  $n_{eff}/N > 0.001$ . Before proceeding any further, we also check HMC specific diagnostics: *Divergences*, *Tree depth*, and *Energy Bayesian Fraction of Missing Information*.

```
rstan::check_hmc_diagnostics(f2pStan)

##
## Divergences:

## 0 of 4500 iterations ended with a divergence.

##
## Tree depth:

## 0 of 4500 iterations saturated the maximum tree depth of 10.

##
## Energy:

## E-BFMI indicated no pathological behavior.
```



Looks like all is good here.

Once we check that there are no issues with respect to  $\hat{R}$ , the effective sample size or the HMC diagnostics, we can proceed to evaluate our fitted model.

First, let us extract the posterior distribution of the variables of interest using the `rstan` function `extract`.

```
zsp2pStan <- rstan::extract(f2pStan, pars=c("z"))[[1]]
sdop2pStan <- rstan::extract(f2pStan, pars=c("sdo"))[[1]]
sdpp2pStan <- rstan::extract(f2pStan, pars=c("sdp"))[[1]]
```

We can use the mean of the posterior distribution of the states as their estimates and the quantiles of the posterior distribution of the states to get their 95% credible intervals.

```
zs2pStan <- colMeans(zsp2pStan)
zsCIl2pStan <- apply(zsp2pStan, 2, quantile, probs=0.025)
zsCIu2pStan <- apply(zsp2pStan, 2, quantile, probs=0.975)
```

We can then plot the estimated states over the simulated data.

```
plot(1:TT, y,
     pch=3, cex = 0.8, col="blue", ty="o", lty = 3,
     xlab = "t", ylab = expression(z[t]),
     xlim = c(0,TT), ylim = c(min(y), max(y)+max(y)/5),
     las = 1)
points(0:TT, z,
       pch = 19, cex = 0.7, col = "red", ty = "o")
polygon(c(1:TT, TT:1),
        c(zsCIl2pStan, rev(zsCIu2pStan)),
        col=rgb(1,0.7,0.4,0.3), border=FALSE)
lines(1:TT, zs2pStan,
      col = "darkgoldenrod1", lwd = 2)
legend("top",
      legend = c("Obs.", "True states", "Filter. states"),
      pch = c(3, 19, NA),
      col = c("blue", "red", "darkgoldenrod1"),
      lwd = c(1, 1, 2), lty = c(3, 1, 1),
      horiz=TRUE, bty="n", cex=0.9)
```

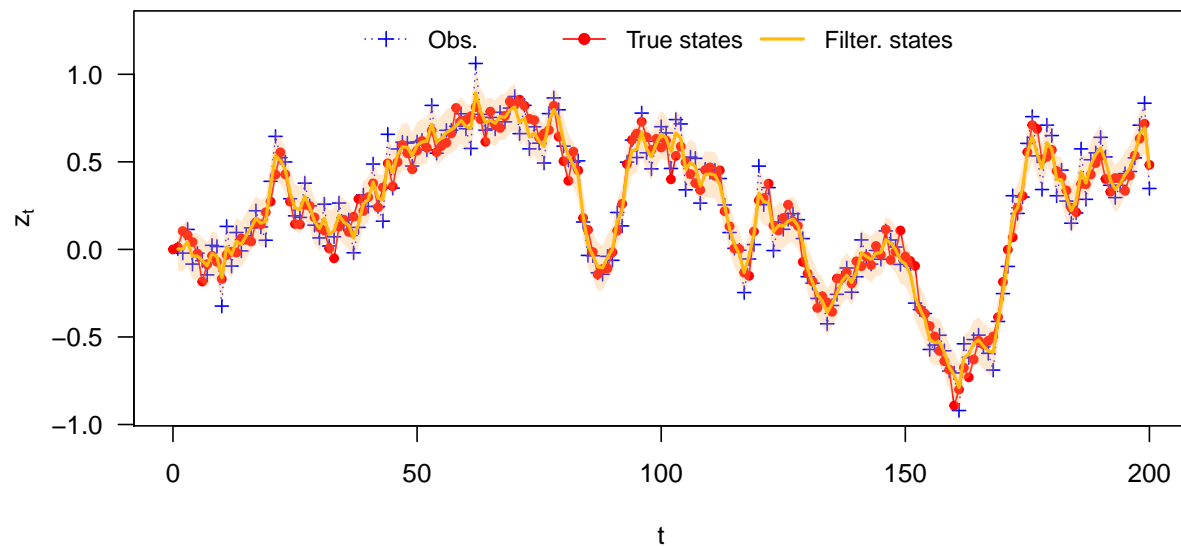

Figure S1.35: Estimated states from Stan overlaid on the simulated data.

We can also use the simulated data to look at how well the states are estimated.

```
# Direct comparison
plot(z[2:(TT+1)], zs2pStan,
     xlab=expression(z[t]),
     ylab=expression(widehat(z)[t]),
     pch=16, cex=0.8)
abline(0,1, col="hotpink", lwd=2)
# How the differen changes through time
plot(1:TT, z[2:(TT+1)] - zs2pStan,
     xlab="t",
     ylab= expression(z[t] - widehat(z)[t]),
     pch=16, cex=0.8)
abline(h=0, col="hotpink", lwd=2)
```

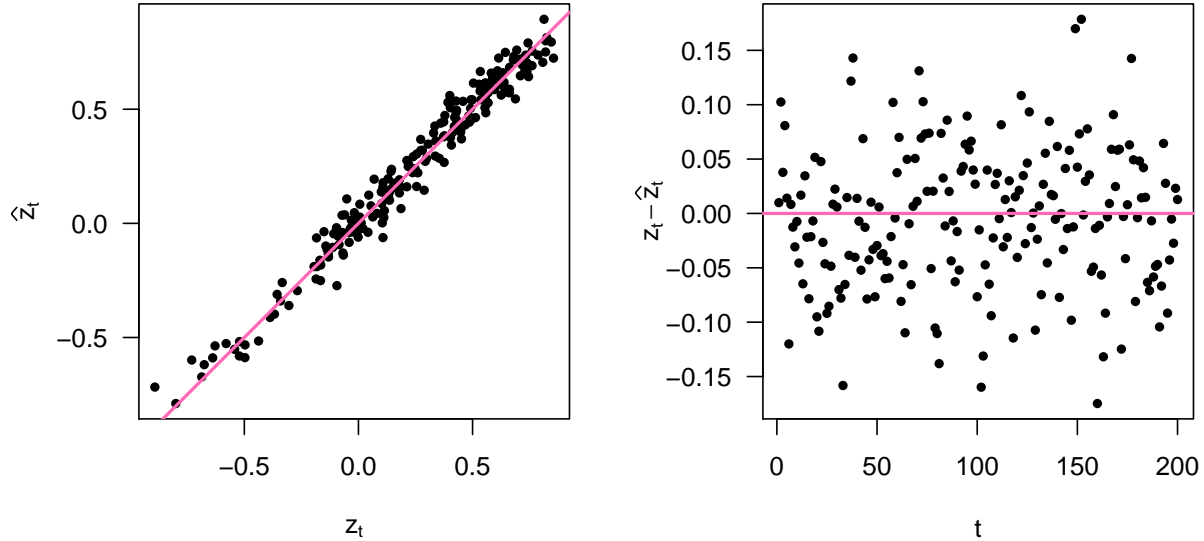

Figure S1.36: Comparison of the estimated states with Stan and the true simulated values.

Looks like we are estimating the states relatively well, or at least with no consistent bias. Note that we could also use the R package `shinystan` to evaluate and visualize the fitted model.

As a note, we have not described in details model selection and comparison for the Bayesian packages. However, we want to highlight that the package `loo` is extremely useful for this and is compatible with models fitted with `rstan`. However, to be able to use `loo` we need to rewrite the stan model so that quantities, such as the pointwise log-likelihoods, can be extracted. See the extensive vignettes from the `loo` packages for details.

## S1 1.4 Assessing parameter redundancy and identifiability with the Hessian method

As discussed in the main text, SSMs can often suffer from parameter identifiability issues. We will demonstrate here how we can use the Hessian method to assess whether this is the case.

Suppose we adapted our simple linear Gaussian SSM, so that the state equation is

$$z_t = \beta_1 \beta_2 z_{t-1} + \epsilon_t, \quad \epsilon_t \sim N(0, \sigma_p^2), \quad (1.20)$$

and the observation equation remains as

$$y_t = \alpha z_t + \eta_t, \quad \eta_t \sim N(0, \sigma_o^2), \quad (1.21)$$

for  $t = 1, \dots, T$ . The parameters in this model are  $\alpha, \beta_1, \beta_2$ . We fix the parameters  $\sigma_o = 0.1$  and  $\sigma_p = 0.1$ .

However, we can reparameterize this model so that  $\beta = \beta_1\beta_2$ , getting back our original model (Eq. 1.1).

It would not be possible to find unique estimates for parameters  $\beta_1$  and  $\beta_2$ , whereas a unique estimate of  $\beta$  could theoretically be found. This is an example of parameter redundancy or non-identifiability and the one we will use to explore the Hessian method.

To get a feel for the method, it helps to discuss a few matrix algebra concepts in the context of maximum likelihood. The Hessian is a square matrix of second-order partial derivatives of a function. In the context of maximum likelihood, the Hessian of the log likelihood function at the MLE gives a sense of the curvature of the likelihood surface with respect to changes in parameter values. So for example, the Hessian of our model above (Eqs. 1.20-1.21), where we estimate three parameters ( $\alpha$ ,  $\beta_1$ , and  $\beta_2$ ) and the log-likelihood function is denoted by  $l$  would be:

$$\begin{bmatrix} \frac{\partial^2 l}{\partial \alpha^2} & \frac{\partial^2 l}{\partial \alpha \partial \beta_1} & \frac{\partial^2 l}{\partial \alpha \partial \beta_2} \\ \frac{\partial^2 l}{\partial \alpha \partial \beta_1} & \frac{\partial^2 l}{\partial \beta_1^2} & \frac{\partial^2 l}{\partial \beta_1 \partial \beta_2} \\ \frac{\partial^2 l}{\partial \alpha \partial \beta_2} & \frac{\partial^2 l}{\partial \beta_1 \partial \beta_2} & \frac{\partial^2 l}{\partial \beta_2^2} \end{bmatrix} \quad (1.22)$$

The second partial derivatives with respect to the same variable twice (e.g.,  $\frac{\partial^2 l}{\partial \alpha^2}$ ) represents the curvature of the log-likelihood surface along the particular axis, while the cross-derivatives ( $\frac{\partial^2 l}{\partial \alpha \partial \beta_1}$ ) describe how the slope in one direction changes as you move along another direction (Bolker, 2008). It is beyond the scope of this tutorial to explain the linear algebra concepts such as eigenvalues, but we can think of them as characteristic values describing a matrix. The main point is that if the model is identifiable (i.e., there is a clear peak in the likelihood at the MLE), all of the eigenvalues of the Hessian matrix will be non-zero. If the model is non-identifiable, then the Hessian matrix will be singular and at least one of the eigenvalues of the Hessian matrix will be 0.

Thus, to assess identifiability, we can calculate numerically the Hessian matrix and then calculate its eigenvalues. We then assess whether one of the eigenvalues is 0. Because the Hessian matrix is calculated numerically (rather than solved), we may get values close to 0 rather than exactly 0. We use a threshold value to assess whether the eigenvalue is close enough to 0 for the model to be deemed non-identifiable. The number of eigenvalues that are non-zero tells us how many parameters are estimable.

Below we show how to use the Hessian method to investigate identifiability.

Step 1: load the Hessian method functions:

Load two generic functions that will allow to calculate the Hessian and its eigenvalues. As we will see in step 2, these functions can be applied to any functions that returns the log likelihood.

The first function calculates the Hessian numerically.

```
hessian <- function(funfcn,x,y,delta){
  # function to calculate the hessian of funfcn at x
  t <- length(x)
  h <- matrix(0, t, t)
  Dx <- delta*diag(t)
  for (i in 1:t) {
```

```

for (j in 1:i) {
  h[i,j] <- (do.call("funfcn",list(x+Dx[i,]+Dx[j,],y)) # LL with
    - do.call("funfcn",list(x+Dx[i,]-Dx[j,],y))
    - do.call("funfcn",list(x-Dx[i,]+Dx[j,],y))
    + do.call("funfcn",list(x-Dx[i,]-Dx[j,],y)))/(4*delta^2)
  h[j,i] <- h[i,j]
}
}
return(h)
}

```

The second function uses the one above to calculate the Hessian, then it calculates the eigenvalues and assesses whether some of these eigenvalues are 0. It returns messages on whether the model is deemed non-identifiable. The functions also calculates how many eigenvalues are greater than 0 and thus how many parameters are thought to be estimable.

```

hessianmethod <- function(funfcn,pars,y,delta,print=TRUE){
  # Applies the Hessian method
  # funfcn - function which return negative loglikelihood
  # pars - parameter values at which hessian is evaluated
  # y - data to be passed into likelihood
  # delta - error used in calculating Hessian and cutt-off
  # suggested value delta = 0.00001
  # cut-off used delta*p, where p is no. pars
  cutoff <- delta*length(pars)
  # Finds hessian matrix
  h <- do.call("hessian",list(funfcn,pars,y,delta))
  # Calculates eigenvalues
  E <- eigen(h)
  # find standardised eigenvalues
  standeigenvalues <- abs(E$values)/max(abs(E$values))
  # find number of estimable parameters
  # number of parameters with eigenvalues below the cutoff
  noestpars <- 0
  for (i in 1:length(pars)) {
    if (standeigenvalues[i] > cutoff) {
      noestpars <- noestpars + 1
    }
  }
  if (print) {
    # Prints whether model is parameter redundant or not

```

```

# Then prints smallest eigenvalue and
# number of estimable parameters
if (min(standeigenvalues) < cutoff) {
  cat("model is non-identifiable or parameter redundant")
}
else {
  cat("model is identifiable or not parameter redundant")
}
cat("\n")
cat('smallest standardized eigenvalue',min(standeigenvalues))
cat("\n")
cat('number of estimable parameters',noestpars)
}
result <- list(standeigenvalues=standeigenvalues,noestpars=noestpars)
return(result)
}

```

Step 2: Create a function that defines the model as a function of the parameter values to estimate and returns the log-likelihood.

The next step is to create a function that returns the log likelihood of the model. Here we use `d1m`, but we could use `TMB` or any package that allow us to write a function that inputs parameter values and data and returns the log likelihood of your model. This would generally be done as part of the model fitting procedure.

```

# Here beta[1] = theta[1], beta[2] = theta[2] and alpha = theta[3]
mfx <- function(theta) {
  d1m(m0 = 0, C0 = 0,
      GG = theta[1]*theta[2], W = 0.1^2,
      FF = theta[3], V = 0.1^2)
}
likfx <- function(theta,y) {
  RW.obj <- mfx(theta)
  d1mLL(y = y, mod = RW.obj)
}

```

Step 3: Find the maximum likelihood estimates of the parameters.

The Hessian is evaluated at the MLE. Thus, the next step involves finding the MLE. Again, this is a step that would normally be done as part of the model fitting procedures. We continue using `d1m` here, but any other package that allow to find the MLE would work.

```
ffx <- dlmMLE(y = y, parm = c(1,1,1),
             build = mfx)
```

Step 4: Use the function `hessianmethod` to find whether or not the model is identifiable.

We use the function we defined in Step 1 to assess whether the model is identifiable.

```
results <- hessianmethod(likfx, ffx$par, y, 0.00001)

## model is non-identifiable or parameter redundant
## smallest standardized eigenvalue 1.473652e-07
## number of estimable parameters 2
```

By default, the function prints messages that state: 1) whether the model is identifiable, 2) the smallest standardized eigenvalue, and 3) the number of estimable parameters. The function returns the standardized eigenvalues and the number of parameters that can be estimated. The standardized eigenvalues were calculated by taking the absolute value of each eigenvalue and dividing by the largest eigenvalue.

In this case, as the smallest eigenvalue is very close to zero the model is non-identifiable. For a non-identifiable model, the number of estimable parameters is the number of parameters that could be estimated if the model was reparameterized in a form that was identifiable. If using model selection techniques, such as AIC, the number of estimable parameters, rather than the number of parameters, should be used in the calculation for non-identifiable models. In this case the number of estimable parameters is 2, whereas the number of parameters is 3.

Next consider the reparameterized model with  $\beta = \beta_1\beta_2$ . This has two parameters  $\beta$  and  $\alpha$ .

```
# Setting up model with parameters beta = theta[1] and alpha = theta[2]
mfx <- function(theta) {
  dlm(m0 = 0, C0 = 0,
      GG = theta[1], W = 0.1^2,
      FF = theta[2], V = 0.1^2)
}
# Find the MLE
ffx <- dlmMLE(y = y, parm = c(1,1),
             build = mfx)
# Check identifiability using the Hessian method
results <- hessianmethod(likfx, ffx$par, y, 0.00001)

## model is identifiable or not parameter redundant
## smallest standardized eigenvalue 0.03481255
## number of estimable parameters 2
```

As the smallest eigenvalue is now 0.035, this model is identifiable. Note that in an identifiable model the number of estimable parameters is the same as the number of parameters, which in this case is 2.

This method can be inaccurate, as it involves deciding whether an eigenvalue is *close to zero*. The program uses a threshold of  $\tau = \delta p$ , where  $p$  is the number of parameters in the model and  $\delta$  specifies the interval length used in the Hessian approximation. Regardless of the threshold used it is possible to misclassify identifiability. Also the result will depend on the data used.

An alternative method, which is accurate, involves using symbolic algebra. A symbolic algebra package is needed to execute the symbolic algebra, and it is easier to use software such as Maple, rather than R. Please see Appendix S3 for more details.



## Chapter 2

# Movement SSM

Now that we have explored an extensive array of tools using a toy example, we will explore a few of the tools a bit further using more complex SSM, which has been used extensively in the animal movement literature.

### S1 2.1 The model

The model is called a first difference correlated random walk model (DCRW; Jonsen et al., 2005). We will use a slightly simplified version of the model here.

The process equation is:

$$\mathbf{z}_t = \mathbf{z}_{t-1} + \gamma(\mathbf{z}_{t-1} - \mathbf{z}_{t-2}) + \boldsymbol{\epsilon}_t, \quad \boldsymbol{\epsilon}_t \sim N(0, \boldsymbol{\Sigma}), \quad (2.1)$$

where

$$\boldsymbol{\Sigma} = \begin{bmatrix} \sigma_{\epsilon,lon}^2 & 0 \\ 0 & \sigma_{\epsilon,lat}^2 \end{bmatrix}, \quad (2.2)$$

where  $\mathbf{z}_t$  is a vector with the two coordinates of the animal location at time  $t$ . This equation assumes that the animal's location at time  $t$ ,  $\mathbf{z}_t$ , depends on the previous locations,  $\mathbf{z}_{t-1}$ , and on the animal's previous movement in each direction ( $\mathbf{z}_{t-1} - \mathbf{z}_{t-2}$ ). The parameter  $\gamma$  controls the level of correlation between steps. This parameter can take values between 0 and 1, with values close to 1 meaning that the animals has a tendency to move at the same speed and in the same direction as the previous step. See main text for more details.

The observation equations is:

$$\mathbf{y}_i = (1 - j_i)\mathbf{z}_{t-1} + j_i\mathbf{z}_t + \boldsymbol{\eta}_i, \quad \boldsymbol{\eta}_i \sim T(\boldsymbol{\Psi} \circ \mathbf{S}_i, \mathbf{D}_i), \quad (2.3)$$

where

$$\boldsymbol{\Psi} = \begin{bmatrix} \psi_{lon} \\ \psi_{lat} \end{bmatrix}, \quad (2.4)$$

$$\mathbf{S}_i = \begin{bmatrix} s_{lon,q_i} \\ s_{lat,q_i} \end{bmatrix}, \quad (2.5)$$

$$\mathbf{D}_i = \begin{bmatrix} df_{lon,q_i} \\ df_{lat,q_i} \end{bmatrix}. \quad (2.6)$$

The observation equation allows for irregularly timed observations and a complex error structure, two characteristics common to the Argos Doppler shift data for which it was developed. Because data are taken at irregular time intervals,  $i$ , the true location of the animal is linearly interpolated to the time of the observation, with  $j_i$  representing the proportion of the regular time interval between  $t - 1$  and  $t$  when the observation,  $y_i$  was made. Because the data often have outliers, it uses a t-distribution, which has fat tails. Finally, each Argos location comes with an associated quality category, which represents how good the data are. The parameters of the t-distribution depends on the quality category of the observation,  $q_i$ . In particular, in the R package **bsam**, which was developed to fit different versions of this model to Argos data, we have information on the scale parameter of each category and coordinate. This information is contained in  $\mathbf{S}_i$ . The original model estimates one correction factor for these values, to allow deviations from the fixed values. Here we allow for two independent correction factors found in  $\Psi$ , one for each the latitude and longitude, as the error in these two coordinates are known to vary differently. The Hadamard product,  $\circ$ , simply states that we perform entry-wise multiplication of the correction factors the scale parameters, i.e.,  $\psi_c s_{c,q_i}$ , for  $c = (lon, lat)$ . As in **bsam**, we also use known values for the degrees of freedom, which are found here in  $\mathbf{D}_i$ .

Because the state at time  $t$ ,  $\mathbf{z}_t$ , depends on the two previous time steps, we need to start the process with a different equation. In particular, we assume for  $t = 1$  that the model is just a simple random walk:

$$\mathbf{z}_1 = \mathbf{z}_0 + \epsilon_1, \quad (2.7)$$

where we use the same error distribution as above.

## S1 2.2 Polar bear movement data

Dr. Andrew Derocher (University of Alberta, Canada) shared one movement track of a polar bear with a collar that provided both Argos data and GPS data. This provides us a unique opportunity to fit the model to error-prone Argos data and check the state estimates with the GPS data, see Auger-Méthé et al. (2017). Data is available through Dryad (doi:10.5061/dryad.4qrfj6q96).

Let us load and investigate the Argos data first.

```
# Read the data
dataPbA <- read.csv("Data/PB_Argos.csv")
# Look at what it contains
head(dataPbA)
```

| ##   |            | DateTime | QualClass | Lat    | Lon      |
|------|------------|----------|-----------|--------|----------|
| ## 1 | 2009.04.20 | 17:01:39 | B         | 70.365 | -131.837 |
| ## 2 | 2009.04.20 | 17:23:00 | A         | 70.953 | -131.381 |
| ## 3 | 2009.04.20 | 18:12:15 | A         | 70.957 | -131.365 |
| ## 4 | 2009.04.20 | 20:43:17 | A         | 70.909 | -131.418 |
| ## 5 | 2009.04.21 | 17:11:29 | B         | 71.331 | -131.607 |
| ## 6 | 2009.04.21 | 17:47:36 | B         | 71.225 | -132.099 |

We can see that we have a column with the date and time, one with the Argos quality class, one with the latitude and one with the longitude. Let us plot the data.

```
plot(dataPbA[,c("Lon", "Lat")],  
     pch=3, cex=0.7, col = "blue", ty="o", lty=3, las=1)
```

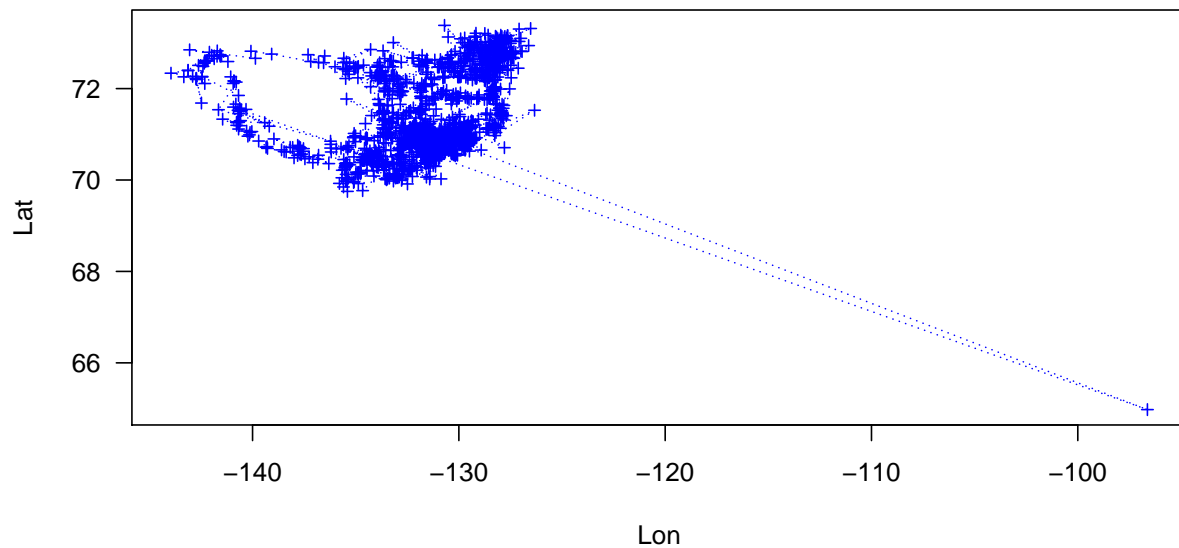

Figure S2.1: Observed Argos polar bear locations.

There are clear outliers, which are likely the results of observation error rather than a bear moving at record speed.

Now let us load the GPS data.

```
# Read the GPS data  
dataPbG <- read.csv("Data/PB_GPS.csv")  
# Look at what it contains  
head(dataPbG)  
  
##           DateTime      Lat      Lon  
## 1 2009.04.20 17:00:37 70.95645 -131.3861  
## 2 2009.04.21 17:00:35 71.08914 -131.5248
```

```
## 3 2009.04.22 17:00:37 71.10673 -131.6351
## 4 2009.04.23 17:00:37 71.08545 -131.6075
## 5 2009.04.24 17:00:37 71.22733 -131.7066
## 6 2009.04.25 17:01:07 71.23823 -131.8137
```

Here again we have a column with the date and time, one with the latitude and one with the longitude. Let us plot the two types of data together.

```
plot(dataPbG[,c("Lon", "Lat")],
     pch=19, cex=0.7, col = "red", ty="o", las=1,
     ylim=c(min(dataPbG$Lat),max(dataPbG$Lat)+0.4))
points(dataPbA[,c("Lon", "Lat")],
       pch=3, cex=0.7, col = "blue", ty="o", lty=3)
legend("top",
      legend = c("Obs. (Argos)", "True states (GPS)"),
      pch = c(3, 19),
      col = c("blue", "red"),
      lty = c(3, 1),
      horiz=TRUE, bty="n", cex=0.9)
```

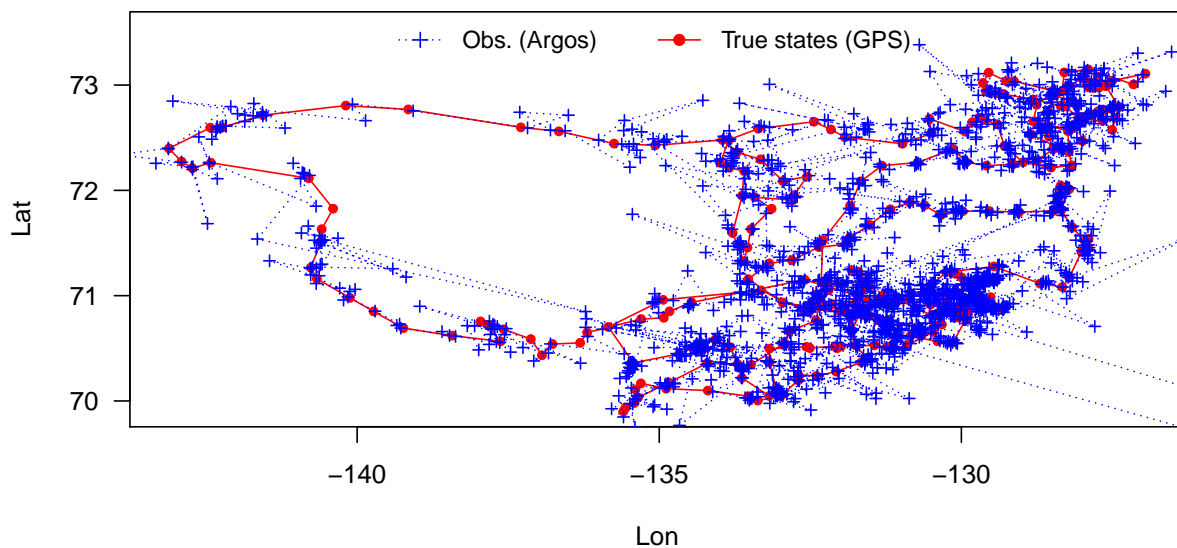

Figure S2.2: Observed Argos polar bear locations with true locations (GPS points) overlaid on top.

We can see that the movement according to Argos data is much more erratic than GPS data, which is entirely due to the observation error associated with Argos data.

Here we will use the Argos data to estimate states at regular time intervals and we will use the GPS data to investigate the model's capacity to estimate the states. So that the estimates are at the same time as the GPS data, we will estimate states once a day at 17:00. The following code chunk is just data manipulation to create the  $i$  index and the time proportion  $j_i$  so that we relate the time of the observed Argos locations to the time of the estimated states and GPS data.

```
# Transform DateTime in R date.time class
dataPbA$Time <- as.POSIXlt(dataPbA$DateTime,
                           format="%Y.%m.%d %H:%M:%S", tz="UTC")
dataPbA$Date <- as.Date(dataPbA$Time)

# Create a regular time series that will
# represent the time at which we will estimate the states (z)
# Note that because our last Argos location is after 17:00,
# we end time series one day after
allDays <- seq(dataPbA$Date[1],
               dataPbA$Date[length(dataPbA$Time)] + 1, 1)
allDays <- as.POSIXlt(paste(allDays, "17:00"), tz="UTC")

# Find in between which z (allDays) observation y fall
# +1 because the it's the proportion of time between t-1 and t, we link with t.
dataPbA$idix <- findInterval(dataPbA$Time, allDays) + 1
# Checking how far from the z_t y is
dataPbA$ji <- as.numeric(24-difftime(allDays[dataPbA$idix],
                                     dataPbA$Time, units="hours"))/24
```

It is customary to use error data to help the estimation process. Here we create a matrix with the error values, these values are based on those used in the package **bsam**, see below. We have done a few changes to the values used in **bsam**. In particular, the skewness of the t-distribution is undefined when the degree of freedom is  $\leq 3$ . We have thus set any degree of freedom values smaller or equal to 3 to 3.00001.

```
ArgosC <- matrix(nrow=6, ncol=4)
colnames(ArgosC) <- c("TLon", "NuLon", "TLat", "NuLat")
ArgosC[, "TLon"] <- c(0.037842190, 0.004565261, 0.019461776,
                    0.008117727, 0.002807138, 0.002608584)
ArgosC[, "TLat"] <- c(0.027369282, 0.004594551, 0.014462340,
                    0.004142703, 0.002344425, 0.001098409)
ArgosC[, "NuLon"] <- c(3.00001, 3.00001, 3.00001,
                    3.00001, 3.00001, 3.070609)
ArgosC[, "NuLat"] <- c(3.00001, 3.00001, 3.00001,
```

```

                                3.896554, 6.314726, 3.00001)
rownames(ArgosC) <- c("B", "A", "0",
                     "1", "2", "3")

```

Now we create new columns in the data set that indicate the standard deviation and the degrees of freedom to use with each location.

```
dataPbA$ac <- ArgosC[as.character(dataPbA$QualClass),]
```

## S1 2.3 Fitting the model and checking model fit

A very similar model to the one above can be easily fitted using a package called **bsam**, which was specifically designed for this model and its extensions. But here we will only explore a few of the generic tools we have presented above.

### S1 2.3.1 TMB

As for the toy example, the first thing we need to do to be able to fit the model in TMB is to create a file that will contain the C++ code to evaluate the negative log-likelihood value of the model. We will name the file *dcrw.cpp*.

```

/*----- SECTION A -----*/
// State that we need the TMB package
#include <TMB.hpp>
// Needed for the multivariate normal function: MVNORM_t
using namespace density;

/*----- SECTION B -----*/
// Define main function
template<class Type>
Type objective_function<Type>::operator() ()
{

    /*----- SECTION C -----*/
    // Specify the input data
    DATA_ARRAY(y); // Longitude and latitude of locations
    DATA_VECTOR(idx); // Index linking irregular obs. time i to state time t
    DATA_VECTOR(ji); // When is obs. i relative to state t-1 and t
    DATA_MATRIX(ac); // Argos category

```

```

// For one-step-ahead residuals
DATA_ARRAY_INDICATOR(keep, y);

// Input parameters - i.e. parameters to estimate.
PARAMETER(logitGamma); // Autocorrelation
PARAMETER(logSdLon); // Process standard deviation in lon
PARAMETER(logSdLat); // Process standard deviation in lat
PARAMETER(logPsiLon); // Scaling parameter for error values
PARAMETER(logPsiLat); // Scaling parameter for error values

// The true/unobserved locations of the animal, i.e states
PARAMETER_MATRIX(z);

/*----- SECTION D -----*/
// Transformation of the input parameters to model format
/* These transformations are made to insured that
   the parameters have sensical values.
   They do not change the model, they are only a computational trick. */
Type gamma = 1.0/(1.0+exp(-logitGamma)); // b/c we want  $0 < \gamma < 1$ 
Type sdLon = exp(logSdLon); // b/c we want  $sd > 0$ 
Type sdLat = exp(logSdLat); // b/c we want  $sd > 0$ 
Type psiLon = exp(logPsiLon); // b/c we want  $\psi > 0$ 
Type psiLat = exp(logPsiLat); // b/c we want  $\psi > 0$ 

/*----- SECTION E -----*/
// Setting the bivariate normal
// Variance-covariance matrix for the process equation.
// We are using a bivariate normal even if there is no correlation.
matrix<Type> covs(2,2);
covs << sdLon*sdLon, 0, 0, sdLat*sdLat;

// Notes:
// - the mean of MVNORM_t is fixed at 0,
//   thus we only specify the variance-covariance matrix.
// - MVNORM_t evaluates the negative log density
MVNORM_t<Type> nll_dens(covs);

/*----- SECTION F -----*/
// Creating a variable that keeps track of the negative log likelihood
Type nll = 0.0;

```

```

/*----- SECTION G -----*/
// Creating a variable for the value used as data in bivariate normal
vector<Type> tmp(2);

/*----- SECTION H -----*/
// Initializing the model
// For the 2nd time step, we assume that we have a simple random walk:
// z_1 = z_0 + eta
// Here tmp is simply the difference between the first two states:
// d_1 = z_1 - z_0
tmp = z.row(1) - z.row(0);
nll += nll_dens(tmp);

/*----- SECTION I -----*/
SIMULATE{
    z.row(1) = vector<Type>(z.row(0)) + nll_dens.simulate();
}

/*----- SECTION J -----*/
// nll contribution of the process equation after the 2nd time step
// Notes:
// - .row(i) gives the ith row of parameter or data matrix,
//   so locations at time i.
// - loop here is the size of the states vector z,
//   thus, if we have missing data this loop will be longer
//   than the observation equation
//   and will estimate the state value even for
//   time steps where we have no observation.
for(int i = 2; i < z.rows(); ++i){
    tmp = (z.row(i) - z.row(i-1)) - (z.row(i-1) - z.row(i-2)) * gamma;
    nll += nll_dens(tmp);
}

/*----- SECTION K -----*/
SIMULATE{
    z.row(i) = vector<Type>((1+gamma)*z.row(i-1) - gamma*z.row(i-2)) +
        nll_dens.simulate();
}
}

/*----- SECTION L -----*/

```



```

// nll contribution of the observation equation
// The loop here is just the size of the observation vector.
// We use the time index found in idx to relate
// the appropriate state to the observation.
for(int i = 0; i < y.matrix().rows(); ++i){
    // Interpolate the value at time of observation
    // CppAD::Integer because the index used to get value
    // in a vector in c++ needs to be a integer to work.
    tmp = y.matrix().row(i) -
        ((1.0-ji(i))*z.row(CppAD::Integer(idx(i)-1)) +
         ji(i)*z.row(CppAD::Integer(idx(i)))));

    // We are using the non-standardised t distribution,
    // that is why we are correcting the pdf.
    // Longitude
    nll -= keep(i,0) * (log(1/(psiLon*ac(i,0))) +
        dt(tmp(0)/(psiLon*ac(i,0)),ac(i,1),true));
    // Latitude
    nll -= keep(i,1) * (log(1/(psiLat*ac(i,2))) +
        dt(tmp(1)/(psiLat*ac(i,2)),ac(i,3),true));

    /*----- SECTION M -----*/
    // Simulation of observations
    y(i,0) = psiLon * ac(i,0) * rt(ac(i,1)) +
        ((1.0-ji(i))*z(CppAD::Integer(idx(i)-1),0) +
         ji(i)*z(CppAD::Integer(idx(i)),0));
    y(i,1) = psiLat * ac(i,2) * rt(ac(i,3)) +
        ((1.0-ji(i))*z(CppAD::Integer(idx(i)-1),1) +
         ji(i)*z(CppAD::Integer(idx(i)),1));
}

/*----- SECTION N -----*/
// Report the parameters and their standard errors in their model format
ADREPORT(gamma);
ADREPORT(sdLon);
ADREPORT(sdLat);
ADREPORT(psiLon);
ADREPORT(psiLat);

```

```

/*----- SECTION 0 -----*/
// Report simulated values
SIMULATE{
  REPORT(z)
  REPORT(y)
}

return nll;
}

```

See section S1 1.3.2 for some of the basic rules of C++ and TMB. Here are a few additional notes:

- While this is not necessary here, given that we are assuming that there is no correlation in the movement in the latitude and longitude coordinates, we are using a bivariate normal rather than two univariate normal distribution. We are using it here in part because the multivariate normal is a very useful distribution, and we wanted to demonstrate how it works. To be able to evaluate the probability density function of a multivariate normal, we need to use the `namespace density` as we see in section A. In section E, we then create a covariance matrix that we assign to the multivariate normal. Note that the mean of the multivariate normal is 0 and this cannot be changed and that it will return the negative log density.
- `.row(i)` and `.col(i)` will return the  $i$ th row or column of `PARAMETER_MATRIX` and `DATA_MATRIX`. To be able to use `.row()` and `.col()` on `DATA_ARRAY`, we need to precede these calls by `.matrix()`.
- We used a `DATA_ARRAY` for the observations rather than say a `DATA_MATRIX`. We did so because the indicator objects associated with the one-step-ahead residuals (here `DATA_ARRAY_INDICATOR`), can only be either a vector or an array.
- In sections L and M, we have to use `CppAD::Integer` to transform the `idx` values into integers. We need to do this because `.row()` methods can only take integers.
- We have created temporary objects in section J to be able to evaluate the densities.

Again, the next step is to compile the C++ code and load the compiled function. This code may take a few minutes to run and may print warnings.

```

library(TMB)
compile("dcrw.cpp", flags="-Wno-unused-variable")
dyn.load(dynlib("dcrw"))

```

Then, we need to prepare the data, by which we mean create one list that contains all of the data elements needed by C++. Here we need: 1) the matrix `y`, which contains the longitude and latitude of the locations; 2) the vector `idx`, which contains the index that relates the observation at time  $i$  to the appropriate state time  $t$ ; 3) the vector `ji`, which contains when the observation falls between  $t - 1$  and  $t$ ; and 4) the matrix

ac, which contains all of the error information for the given location. As a note, we are removing 1 from the index value `idx` because the index of C++ starts a 0, not 1.

```
dataPbTmb <- list(y = cbind(dataPbA$Lon, dataPbA$Lat),
                 idx=dataPbA$idx-1, ji=dataPbA$ji, ac=dataPbA$ac)
```

We then need to create a list with the starting values for the parameters, including the states. In section S1 1.3.2, we used 0 as starting values for all parameters and states. Here, to help the optimization, we will set the initial value of the states to be the values of the observed Argos location. This will just start the optimization at the good relative magnitude. We could have alternatively, scaled the model so to have transformed longitude and latitude values that are centered at 0.

```
# Setting the initial values for the state.
# We use the 1st obs. location to start the optimization
# at a relatively good place
zinitPbTmb <- matrix(as.numeric(dataPbA[1,c("Lon","Lat")] ),
                    max(dataPbA$idx), 2, byrow=TRUE)
# Creating a list of initial values for the parameters
parPbTmb <- list(logitGamma=0,
                 logSdLon=0, logSdLat=0, logPsiLon=0, logPsiLat=0,
                 z=zinitPbTmb)
```

We have now all of the pieces needed to create the TMB object with `MakeADFun`, which will allow us to minimize the negative log likelihood. Note that for more complex model, it sometimes help to allow for more iterations in the inner maximization. This can slow down the process, but here if we use the default maximum number of inner iterations, we will get the error:

```
## Warning in nlminb(objPBO$par, objPBO$fn, objPBO$gr): NA/NaN function evaluation
## Error in nlminb(objPBO$par, objPBO$fn, objPBO$gr): gradient function must
return a numeric vector of length 5
```

Thus, we increase the number of inner iterations to 5000 using `inner.control`.

```
mPbTmb <- MakeADFun(dataPbTmb, parPbTmb, random="z", DLL="dcrw", silent=TRUE,
                   inner.control = list(maxit=5000))
```

Using the created object, we can find the MLE with `nlminb`.

```
fPbTmb <- nlminb(mPbTmb$par, mPbTmb$fn, mPbTmb$gr)
fPbTmb$message

## [1] "relative convergence (4)"
```

Looks like it converged, so let us now look at the estimated parameters using `sdreport` just as in section S1 1.3.2.

```
parestPbTmb <- summary(sdreport(mPbTmb))
parestPbTmb[c("gamma", "sdLon", "sdLat", "psiLon", "psiLat"),]

##           Estimate Std. Error
## gamma  0.47523211 0.036106875
## sdLon   0.34653407 0.015189583
## sdLat   0.09993379 0.004188735
## psiLon  4.94418136 0.139059904
## psiLat  1.89246300 0.053489969
```

So it appears that the movement of this bear is only partially dependent on the movement from the previous step, i.e.,  $\gamma = 0.475$ . Interestingly, the process variation is quite different in the latitude and longitude direction. This could be due to the fact that one degree of latitude and one degree of longitude are not necessarily covering equivalent distance. We see also that the correction factors for the longitude and latitude are quite different from one another and might point to the advantage of estimating one for each coordinate.

Now let us look at the state estimates. To extract the state value itself, we use `$env$parList()`. To extract the standard error, we use the matrix returned by `summary(sdreport())` above.

```
# Get the point value
zsPbTmb <- mPbTmb$env$parList()$z
# Get the standard errors
zsvPbTmb <- parrestPbTmb[rownames(parrestPbTmb)%in%"z",]
zsvPbTmb <- cbind(zsvPbTmb[1:(nrow(zsvPbTmb)/2),2],
                  zsvPbTmb[(1+nrow(zsvPbTmb)/2):nrow(zsvPbTmb),2])
```

Now, let us compare the estimated states (i.e., the estimated polar bears locations) to the GPS locations. As GPS data often have missing value, this requires making sure we are comparing the locations at the same time step.

```
# Find the index to match GPS time to estimate time
gpsIndex <- match(as.Date(dataPbG$DateTime, format="%Y.%m.%d %T"),
                  as.Date(allDays))
```

Let us take a quick look to see if the estimated values are close to the GPS values.

```
# Lon
head(cbind(zsPbTmb[gpsIndex,1], dataPbG$Lon))
```

```
##           [,1]      [,2]
## [1,] -131.3788 -131.3861
## [2,] -131.5138 -131.5248
## [3,] -131.6396 -131.6351
## [4,] -131.6984 -131.6075
## [5,] -131.7404 -131.7066
## [6,] -131.6696 -131.8137
```

```
# Lat
head(cbind(zsPbTmb[gpsIndex,2], dataPbG$Lat))
```

```
##           [,1]      [,2]
## [1,]  70.94922  70.95645
## [2,]  71.08639  71.08914
## [3,]  71.10204  71.10673
## [4,]  71.08889  71.08545
## [5,]  71.22450  71.22733
## [6,]  71.22316  71.23823
```

It looks pretty good. Now let us compute the root mean square prediction error.

```
sqrt(colSums((zsPbTmb[gpsIndex,] -
              dataPbG[,c("Lon", "Lat")])^2)/nrow(dataPbG))
```

```
##           Lon           Lat
## 0.12696917 0.03384686
```

So less than a degree in both case. Because latitude and longitude are hard to easily interpret, let us look at it on a map.

```
plot(dataPbG[,c("Lon", "Lat")],
     pch=19, cex=0.7, col = "red", ty="o", las=1,
     ylim=c(min(dataPbG$Lat),max(dataPbG$Lat)+0.4))
points(dataPbA[,c("Lon", "Lat")],
       pch=3, cex=0.7, col = "blue", ty="o", lty=3)
lines(zsPbTmb, cex=0.5,
```

```

col="darkgoldenrod1", lwd = 2)
legend("top",
  legend = c("Obs. (Argos)", "True states (GPS)", "Smooth. state"),
  pch = c(3, 19, NA),
  col = c("blue", "red", "darkgoldenrod1"),
  lwd = c(1, 1, 2), lty = c(3, 1, 1),
  horiz=TRUE, bty="n", cex=0.9)

```

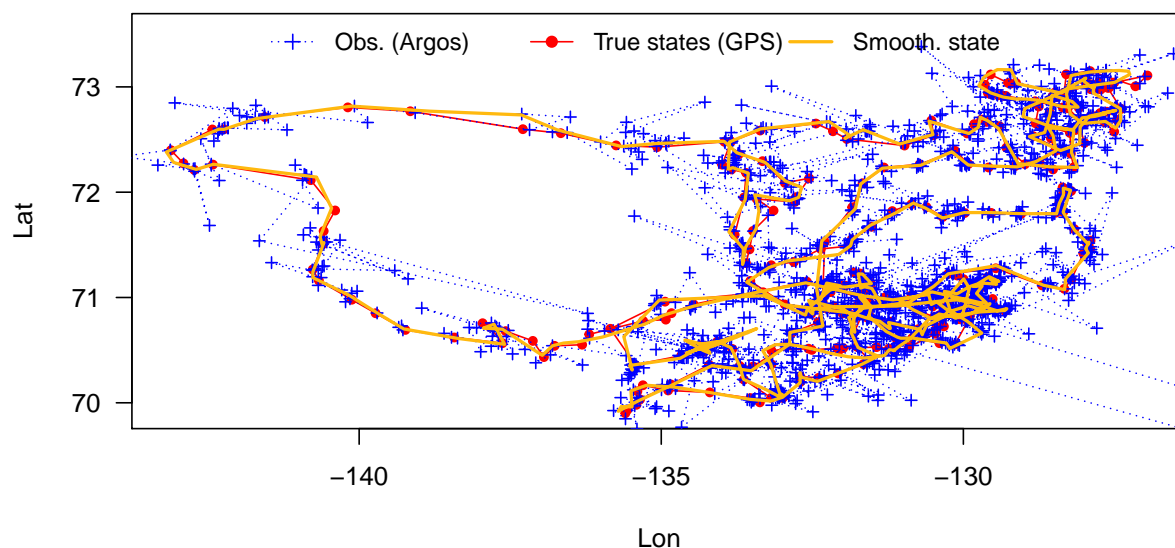

Figure S2.3: Comparison of the estimated locations and the known true locations (GPS points).

Clearly, the estimated locations are much closer to the GPS locations than the Argos locations.

It is good to look at the likelihood profile, and we can use again the function `tmbprofile` as in section S1 1.3.2.7.

Warnings: this can take a few minutes to run.

```

# Get the profile values
proflGammaPbTmb <- tmbprofile(mPbTmb, "logitGamma", trace=FALSE)
proflSdLonPbTmb <- tmbprofile(mPbTmb, "logSdLon", trace=FALSE)
proflSdLatPbTmb <- tmbprofile(mPbTmb, "logSdLat", trace=FALSE)

```

```

proflPpsilonPbTmb <- tmbprofile(mPbTmb, "logPsiLon", trace=FALSE)
proflPsilatPbTmb <- tmbprofile(mPbTmb, "logPsiLat", trace=FALSE)
# Plot the profiles
plot(proflGammaPbTmb)
plot(proflSdLonPbTmb)
plot(proflSdlatPbTmb)
plot(proflPpsilonPbTmb)
plot(proflPsilatPbTmb)

```

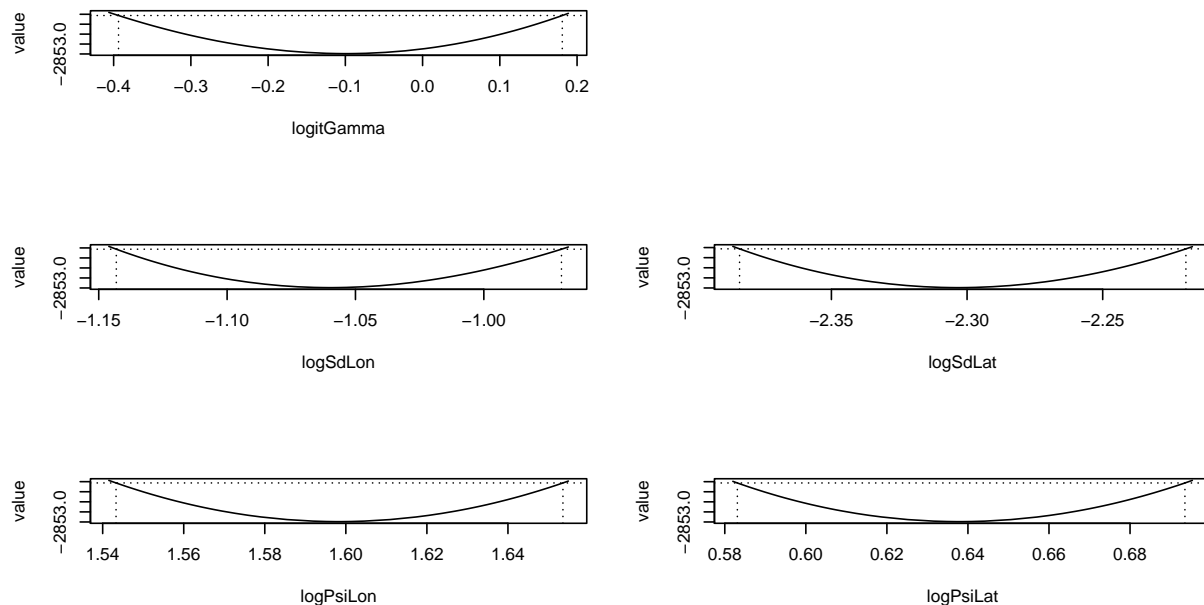

Figure S2.4: Profile of the negative log likelihood of the parameters of the DCRW.

All of these profiles look good.

As we did for the toy model we can also check that the Laplace approximations are good and that our simulations are fitted model. Here because it is a quite complex model, we have increased the number of simulations to 200, to help increase the power of the test.

Warning: this will take a few minutes to run.

```

set.seed(987)
consisPbTmb <- checkConsistency(mPbTmb, n=200)
consisPbTmb

```

```
## Parameters used for simulation:
##  logitGamma    logSdLon    logSdLat    logPsiLon    logPsiLat
## -0.09915273 -1.05977414 -2.30324737  1.59821140  0.63787916
##
## Test correct simulation (p.value):
## [1] 0.4347899
## Simulation appears to be correct
##
## Estimated parameter bias:
##  logitGamma    logSdLon    logSdLat    logPsiLon    logPsiLat
##  0.011456575 -0.008125792 -0.005050737  0.006901017  0.010981128
```

Here, we can see that the p-value for the simulations is high, and above the 0.05 significance level, and thus we are confident that the simulation is consistent with the implemented negative log-likelihood function. The size of the estimated biases for the parameters are both small, indicating that Laplace approximation is not inducing large biases<sup>1</sup>. See `?checkConsistency` for more details.

We can also now simulate from the model. Doing so will simulate a new movement path of the bear and a new set of associated observations.

```
simPbTmb <- mPbTmb$simulate()
```

Let us plot the results.

```
plot(simPbTmb$z,
     pch=19, cex=0.7, col = "red", ty="o", las=1,
     xlab="Longitude", ylab="Latitude",
     ylim=c(min(simPbTmb$z[,2]),max(simPbTmb$z[,2])+0.4))
points(simPbTmb$y,
       pch=3, cex=0.7, col = "blue", ty="o", lty=3)
legend("top",
      legend = c("Obs.", "True states"),
      pch = c(3, 19),
      col = c("blue", "red"),
      lty = c(3, 1),
      horiz=TRUE, bty="n", cex=0.9)
```

<sup>1</sup>If the function returns NA, install TMB from Github (<https://github.com/kaskr/adcomp/>) rather than from CRAN. If using a Mac, you may need to add `SHLIB_OPENMP_CFLAGS=` in the Makevars file.



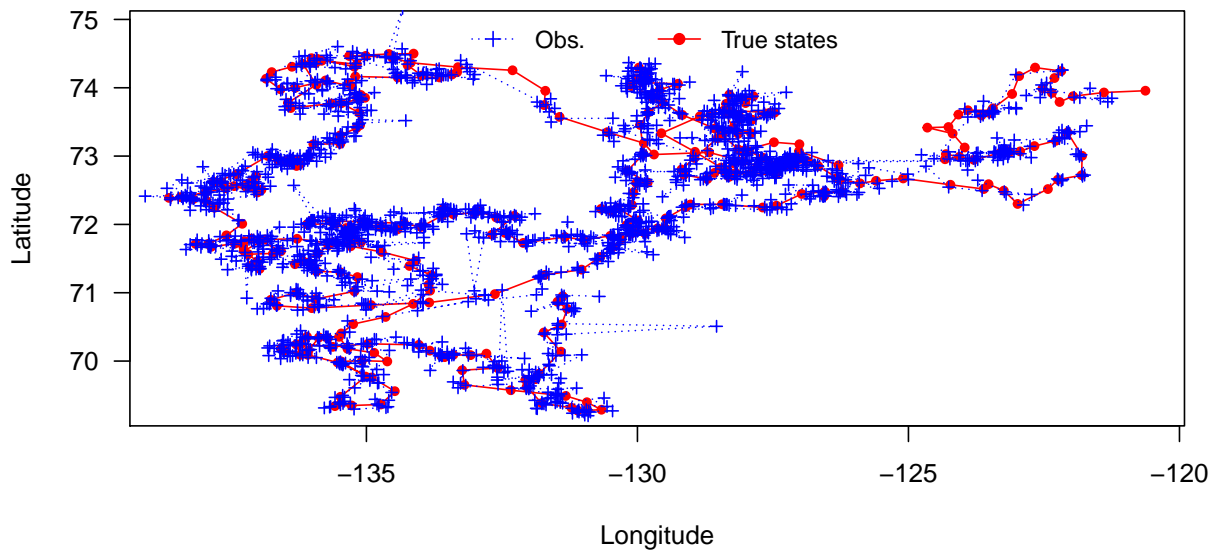

Figure S2.5: Movement path simulated from the fitted model.

We could easily use these simulations to assess, at least informally, whether the parameters are estimable.

We can now look at the one-step-ahead residuals. Because the indicator variable used to keep track of the observations to remove during the calculation of one-step-ahead residuals is an array in the C++ code, it is important to make sure the index used in the `subset` argument correctly describes the order in which the observations are added. When a matrix is transformed into an array, the first column is collated to the second column by default. As such, we want to create an index that goes in sequence from longitude to latitude one time step at a time.

```
# Argos data as a matrix
head(dataPbTmb$y)

##           [,1]    [,2]
## [1,] -131.837 70.365
## [2,] -131.381 70.953
## [3,] -131.365 70.957
## [4,] -131.418 70.909
## [5,] -131.607 71.331
## [6,] -132.099 71.225
```

```

# Argos data when transformed as a array
# Notice that it's the longitude first
head(array(dataPbTmb$y))

## [1] -131.837 -131.381 -131.365 -131.418 -131.607 -132.099

# Create the index vector
# that describes the order of observation to add
pbKeepInd <- as.vector(t(matrix(1:length(dataPbTmb$y), ncol=2)))
head(pbKeepInd)

## [1]      1 1920      2 1921      3 1922

```

Now we can use the function `oneStepPredict` to calculate the one-step-ahead residuals.

Warning: this will take a few minutes to run.

```

pbRes <- oneStepPredict(mPbTmb, observation.name="y",
                        data.term.indicator="keep",
                        discrete=FALSE,
                        subset=pbKeepInd, trace=FALSE)

```

We will separate the residuals for the longitude and latitude. The residuals will be ordered in the same way as `pbKeepInd`, and the first two residuals are not well defined for this model.

```

pbResLon <- pbRes[seq(3, nrow(pbRes), by=2),
                  "residual"]
pbResLat <- pbRes[seq(4, nrow(pbRes), by=2),
                  "residual"]

```

Now let us visually assess the residuals.

```

plot(pbResLon, pch=19, cex=0.5,
      ylab="Residuals - Lon", las=1)
abline(h=0, col="hotpink")
plot(pbResLat, pch=19, cex=0.5,
      ylab="Residuals - Lat", las=1)
abline(h=0, col="hotpink")
acf(pbResLon, main="", ylab="ACF - Lon")
acf(pbResLat, main="", ylab="ACF - Lat")

```

```
hist(pbResLon, breaks=40, freq = FALSE,
     col="darkgrey", las=1,
     main="", ylab="Prob. - Lon")
curve(dnorm, -5, 5, add=TRUE,
      lwd=2, col="hotpink")
hist(pbResLat, breaks=40, freq = FALSE,
     col="darkgrey", las=1,
     main="", ylab="Prob. - Lat")
curve(dnorm, -5, 5, add=TRUE,
      lwd=2, col="hotpink")
```

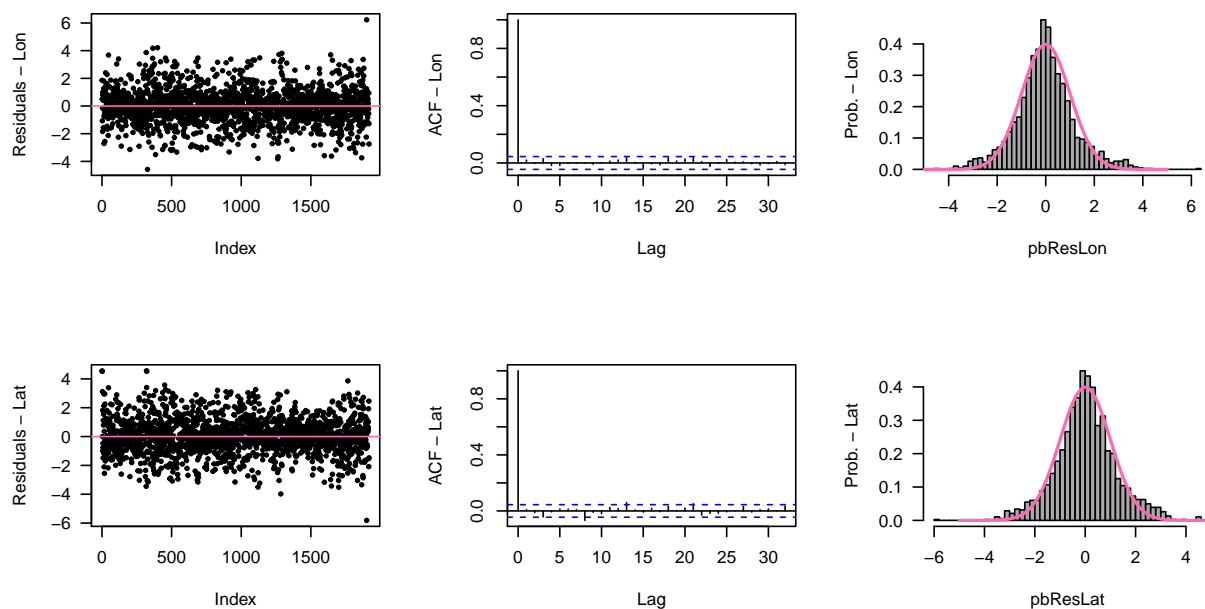

Figure S2.6: One-step-ahead residuals for the DCRW applied to the polar bear Argos data.

Overall the residuals look pretty good. There is no obvious patterns in the residuals through time. There is no autocorrelation. The distribution of the residuals is close to a standard normal. The only sign of a slight problem is that the shape of the residuals is not exactly normal, with some thicker base. This could be due to a mismatch in the values assigned to the different quality categories, and is something worth looking into.

### S1 2.3.2 Stan

We can also write the DCRW model in **Stan**. As for the toy model, the first step is to write the model in the **Stan** language and save it in a file, here called *dcrw.stan*. In the data block, we define: 1) the number of observations, `TTy`; 2) the locations collected through the Argos system, `y`; 3) the interval in which the observations fall into, `intval`; 4) the proportions of time interval when the location falls, `j`; 5) the number of positions to estimate (i.e. the latent states), `TTz`; 5) the degrees of freedom `DD`; and 6) the scaling parameter, `SS`. In the parameter block, we define the parameters and the latent states, `z`. Note that inference can also be done by integrating out the latent states, but is not necessary for inference in **Stan**. The model block contains the manner in which the data are generated as well as the prior distributions for all parameters.

```
data{

  int<lower=1> TTy; // number of observations
  vector[2] y[TTy]; // long/lat from ARGOS
  int<lower=1> intval[TTy]; // which interval do the observations fall into
  vector[TTy] j; //proportions

  int<lower=1> TTz; // number of 'states'

  vector[2] DD[TTy]; // degrees of freedom
  vector[2] SS[TTy]; // scale
}

parameters {
  real<lower=0> sigma_lon;
  real<lower=0> sigma_lat;
  real<lower=0, upper=1> gamma;

  vector[2] z[TTz];

  real<lower=0> psi_lon;
  real<lower=0> psi_lat;
}

model {

  //priors

  gamma ~ uniform(0, 1);
  sigma_lon ~ student_t(3, 0, 1);
  sigma_lat ~ student_t(3, 0, 1);
```

```

psi_lon ~ student_t(3, 0, 1);
psi_lat ~ student_t(3, 0, 1);

//data model

z[2,1] ~ normal(z[1,1], sigma_lon);
z[2,2] ~ normal(z[1,2], sigma_lat);

for(m in 3:TTz){
  z[m,1] ~ normal(z[m-1,1] + gamma*(z[m-1,1] - z[m-2,1]), sigma_lon);
  z[m,2] ~ normal(z[m-1,2] + gamma*(z[m-1,2] - z[m-2,2]), sigma_lat);
}

for(t in 1:TTy){
  y[t,1] ~ student_t(DD[t,1], j[t] * z[intval[t]-1,1] +
    (1-j[t])*z[intval[t],1], psi_lon*SS[t,1]);
  y[t,2] ~ student_t(DD[t,2], j[t] * z[intval[t]-1,2] +
    (1-j[t])*z[intval[t],2], psi_lat*SS[t,2]);
}
}

```

As for the toy model, we then load the `rstan` library and make sure the process is run on multiple cores and is not recompiled unnecessarily.

```

library(rstan)
# To run in parallel on multiple cores
options(mc.cores=parallel::detectCores())
# To avoid recompiling unchanged Stan program
rstan_options(auto_write=TRUE)

```

To fit the model in `Stan`, we include the data in a list and use the `stan` function to fit the model using 3 chains and 4000 iterations. The warm-up period will be 2000 by default. For this complex model, we need to change some of the controls. We increased `adapt_delta`, which is a parameter that set the target average proposal acceptance probability during the warmup period. The default value is 0.8. Increasing it to 0.95 forces `Stan` to take smaller steps. This will mean that we may need to take more steps to properly sample the posterior, and is the reason why we increased the number of iterations. We also change `max_treedepth`. The default value is 10 and here we increase it to 15. This threshold caps the depth of the trees that can be evaluated during each iterations. Increasing `max_treedepth` will make the algorithm less efficient.

Warning: this may take more than 30 minutes to run.

```

dataPbStan <- list(TTy=nrow(dataPbA), y=cbind(dataPbA$Lon, dataPbA$Lat),
  intval=dataPbA$idx, j=dataPbA$ji,
  TTz=max(dataPbA$idx), DD=dataPbA$ac[,c("NuLon", "NuLat")],
  SS=dataPbA$ac[,c("TLon", "TLat")])

fPbStan <- stan(file = "dcrw.stan", data = dataPbStan,
  chains = 3, iter = 4000,
  control=list(adapt_delta=0.95, max_treedepth=15),
  seed= "123") # Set the random to be able to replicate

```

First, we verify that we pass all HMC specific diagnostics.

```

rstan::check_hmc_diagnostics(fPbStan)

##
## Divergences:

## 0 of 6000 iterations ended with a divergence.

##
## Tree depth:

## 0 of 6000 iterations saturated the maximum tree depth of 15.

##
## Energy:

## E-BFMI indicated no pathological behavior.

```

We can print out a subset of the parameters using the `print` argument and specify which parameters are of interest in `pars`.

```

print(fPbStan, pars=c("sigma_lon", "sigma_lat", "gamma", "psi_lon", "psi_lat"))

## Inference for Stan model: dcrw.
## 3 chains, each with iter=4000; warmup=2000; thin=1;
## post-warmup draws per chain=2000, total post-warmup draws=6000.
##
##               mean se_mean    sd 2.5%  25%  50%  75% 97.5% n_eff Rhat

```

```
## sigma_lon 0.35      0 0.02 0.32 0.34 0.35 0.36 0.38 3447 1
## sigma_lat 0.10      0 0.00 0.09 0.10 0.10 0.10 0.11 4433 1
## gamma      0.47      0 0.04 0.40 0.45 0.47 0.50 0.54 4294 1
## psi_lon    5.63      0 0.16 5.33 5.53 5.63 5.74 5.95 4519 1
## psi_lat    2.09      0 0.06 1.97 2.05 2.08 2.12 2.20 4317 1
##
## Samples were drawn using NUTS(diag_e) at Fri Nov 6 18:06:17 2020.
## For each parameter, n_eff is a crude measure of effective sample size,
## and Rhat is the potential scale reduction factor on split chains (at
## convergence, Rhat=1).
```

The values of  $\hat{R}$  and effective sample size are appropriate.

Let us now look at the states.

```
print(fPbStan, pars=c("z"), max=50)

## Inference for Stan model: dcrw.
## 3 chains, each with iter=4000; warmup=2000; thin=1;
## post-warmup draws per chain=2000, total post-warmup draws=6000.
##
##      mean se_mean  sd  2.5%  25%  50%  75%  97.5% n_eff
## z[1,1] -131.49    0.00 0.22 -131.89 -131.63 -131.50 -131.35 -131.02 4382
## z[1,2]  70.81     0.00 0.08  70.65  70.75  70.80  70.86  70.98 5289
## z[2,1] -131.38    0.00 0.02 -131.43 -131.39 -131.38 -131.36 -131.34 4308
## z[2,2]  70.95     0.00 0.01  70.93  70.95  70.95  70.96  70.97 4904
## z[3,1] -131.55    0.00 0.02 -131.59 -131.56 -131.55 -131.53 -131.50 7126
##      Rhat
## z[1,1]  1.00
## z[1,2]  1.00
## z[2,1]  1.00
## z[2,2]  1.00
## z[3,1]  1.00
## [ reached getOption("max.print") -- omitted 729 rows ]
##
## Samples were drawn using NUTS(diag_e) at Fri Nov 6 18:06:17 2020.
## For each parameter, n_eff is a crude measure of effective sample size,
## and Rhat is the potential scale reduction factor on split chains (at
## convergence, Rhat=1).
```

We can extract the predicted locations from the model by using the command `rstan::extract` from the `rstan` package. We further compute the mean, 2.5<sup>th</sup> and 97.5<sup>th</sup> quantiles for the predicted latitude and longitude.

```
zspPbStan <- rstan::extract(fPbStan, pars=c("z"))[[1]]

zsvlonPbStan <- data.frame(mux=colMeans(zspPbStan[,1]),
                          t(apply(zspPbStan[,1], 2, quantile,
                                probs=c(0.025, 0.975))))
zsvlatPbStan <- data.frame(mux=colMeans(zspPbStan[,2]),
                          t(apply(zspPbStan[,2], 2, quantile,
                                probs=c(0.025, 0.975))))
colnames(zsvlonPbStan)[2:3] <- c("q025", "q975")
colnames(zsvlatPbStan)[2:3] <- c("q025", "q975")
```

We can use the extracted states (i.e., the estimated polar bears locations) and compare them to the GPS locations as in the TMB section. As GPS data often have missing value, this requires making sure we are comparing the locations at the same time step.

```
# Find the index to match GPS time to estimate time
gpsIndex <- match(as.Date(dataPbG$DateTime, format="%Y.%m.%d %T"),
                 as.Date(allDays))

## RMSPE
sqrt(sum((dataPbG$Lon - zsvlonPbStan[gpsIndex+1,1])^2)/357)

## [1] 0.1449143

sqrt(sum((dataPbG$Lat - zsvlatPbStan[gpsIndex+1,1])^2)/357)

## [1] 0.03782339
```

Let us plot the results and compare the estimated states to the known locations (GPS locations).

```
plot(dataPbG[, c("Lon", "Lat")],
     pch = 19, cex = 0.7, col = "red", ty = "o",
     las = 1,
     ylim = c(min(dataPbG$Lat), max(dataPbG$Lat) + 0.4))
points(dataPbA[, c("Lon", "Lat")],
       pch = 3, cex = 0.7, col = "blue", ty = "o", lty = 3)
```



```

lines(cbind(zsvlonPbStan$mux[gpsIndex+1], zsvlatPbStan$mux[gpsIndex+1]),
      col = "darkgoldenrod1", lwd = 2)
legend("top",
      legend = c("Obs. (Argos)", "True states (GPS)", "Smooth. state"),
      pch = c(3, 19, NA),
      col = c("blue", "red", "darkgoldenrod1"),
      lwd = c(1, 1, 2), lty = c(3, 1, 1),
      horiz = TRUE, bty = "n", cex = 0.9)

```

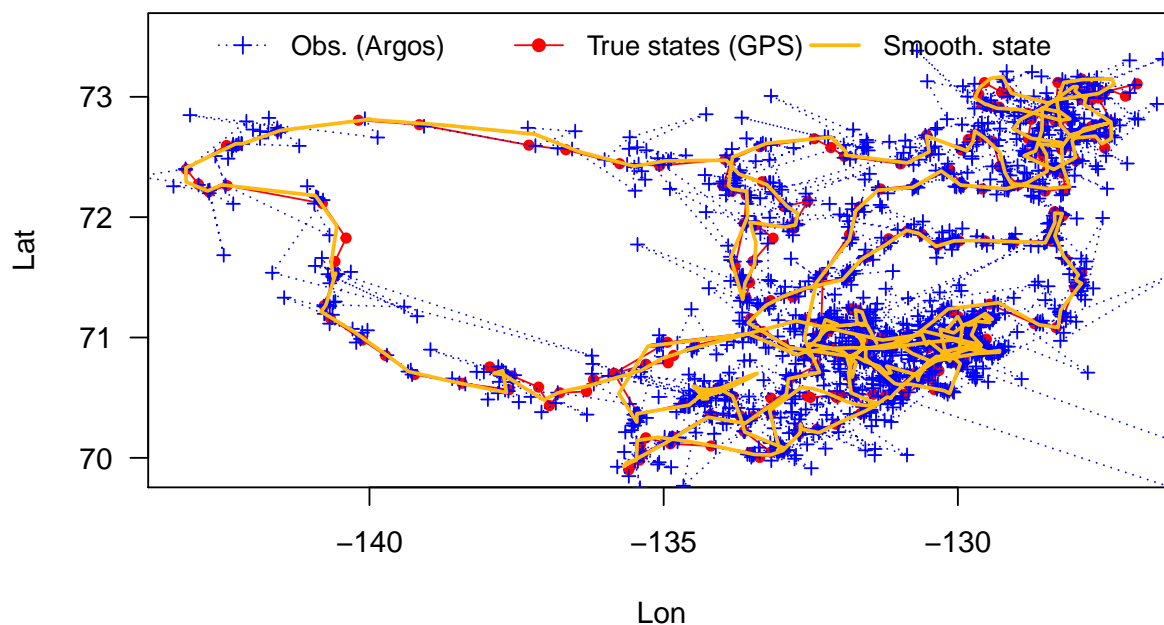

Figure S2.7: Comparison of estimated locations with Stan with the true locations of the polar bear.

Looks good. For model validation methods, see the vignette of the package `loo`.

# Literature Cited

- Auger-Méthé, M., Albertsen, C. M., Jonsen, I. D., Derocher, A. E., Lidgard, D. C., Studholme, K. R., Bowen, W. D., Crossin, G. T., and Mills Flemming, J. (2017). Spatiotemporal modelling of marine movement data using Template Model Builder (TMB). *Marine Ecology Progress Series*, 565:237–249.
- Betancourt, M. (2017). A conceptual introduction to Hamiltonian Monte Carlo. arXiv:1701.02434v2 [stat.ME].
- Bolker, B. M. (2008). *Ecological models and data in R*. Princeton University Press, Princeton, NJ.
- Gelman, A., Carlin, J. B., Stern, H. S., Dunson, D. B., Vehtari, A., and Rubin, D. B. (2013). *Bayesian data analysis, Third Edition*. CRC Press, Boca Raton, FL, 3rd edition edition.
- Jonsen, I. D., Mills Flemming, J., and Myers, R. A. (2005). Robust state-space modeling of animal movement data. *Ecology*, 86(11):2874–2880.
- King, A. A., Ionides, E. L., Bretó, C. M., Ellner, S. P., Ferrari, M. J., Kendall, B. E., Lavine, M., Nguyen, D., Reuman, D. C., Wearing, H., and Wood, S. N. (2020). *pomp: Statistical Inference for Partially Observed Markov Processes*. R package, version 3.1.1.7.
- King, A. A., Nguyen, D., and Ionides, E. L. (2016). Statistical inference for partially observed Markov processes via the R package pomp. *Journal of Statistical Software*, 69(12):1–43.
- Newman, K. B., Buckland, S. T., Morgan, B. J. T., King, R., Borchers, D. L., Cole, D. J., Besbeas, P., Gimenez, O., and Thomas, L. (2014). *Modelling population dynamics: model formulation, fitting and assessment using state-space methods*. Springer, New York.
- Petris, G. (2010). An R package for Dynamic Linear Models. *Journal of Statistical Software*, 36:1–16.
- Stan Development Team (2012). *Stan: A C++ library for probability and sampling*. <http://mc-stan.org>.
